# Supplementary material for: Time-multiplexed Neural Holography: A flexible framework for holographic near-eye displays with fast heavily-quantized spatial light modulators
Source: arXiv:2205.02367 source file (2022-05-05)

Full Light Field

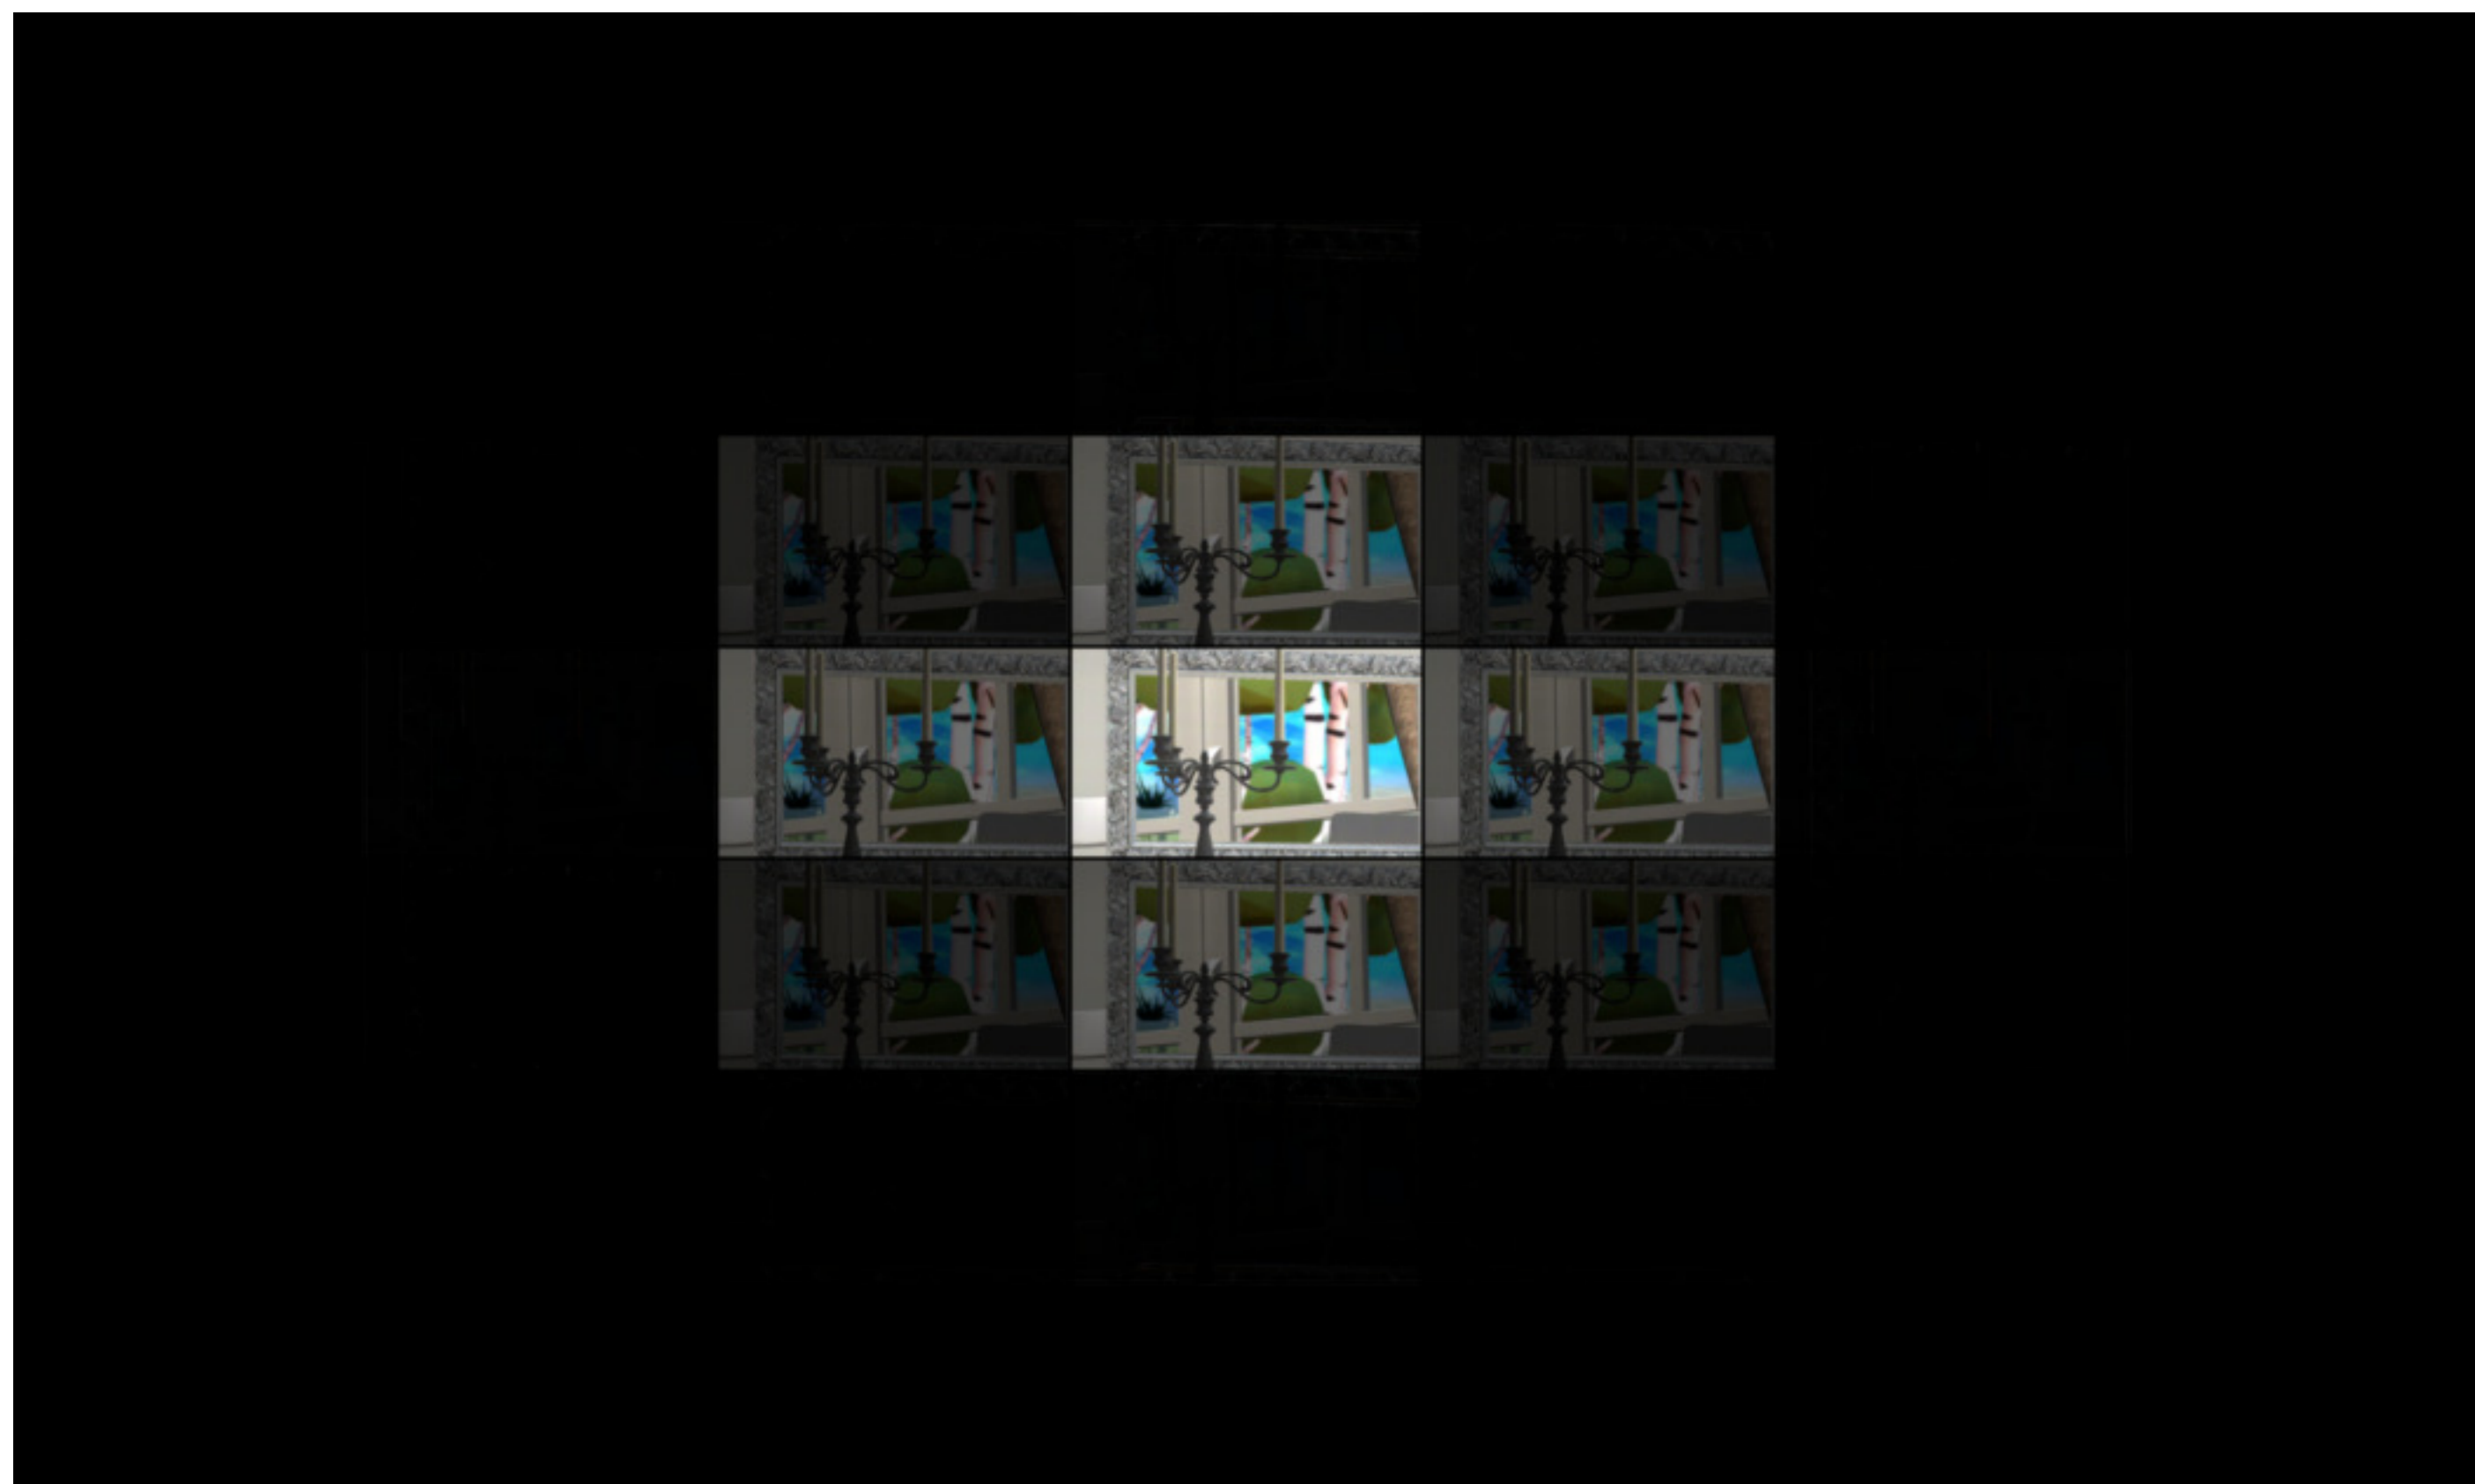

Left View

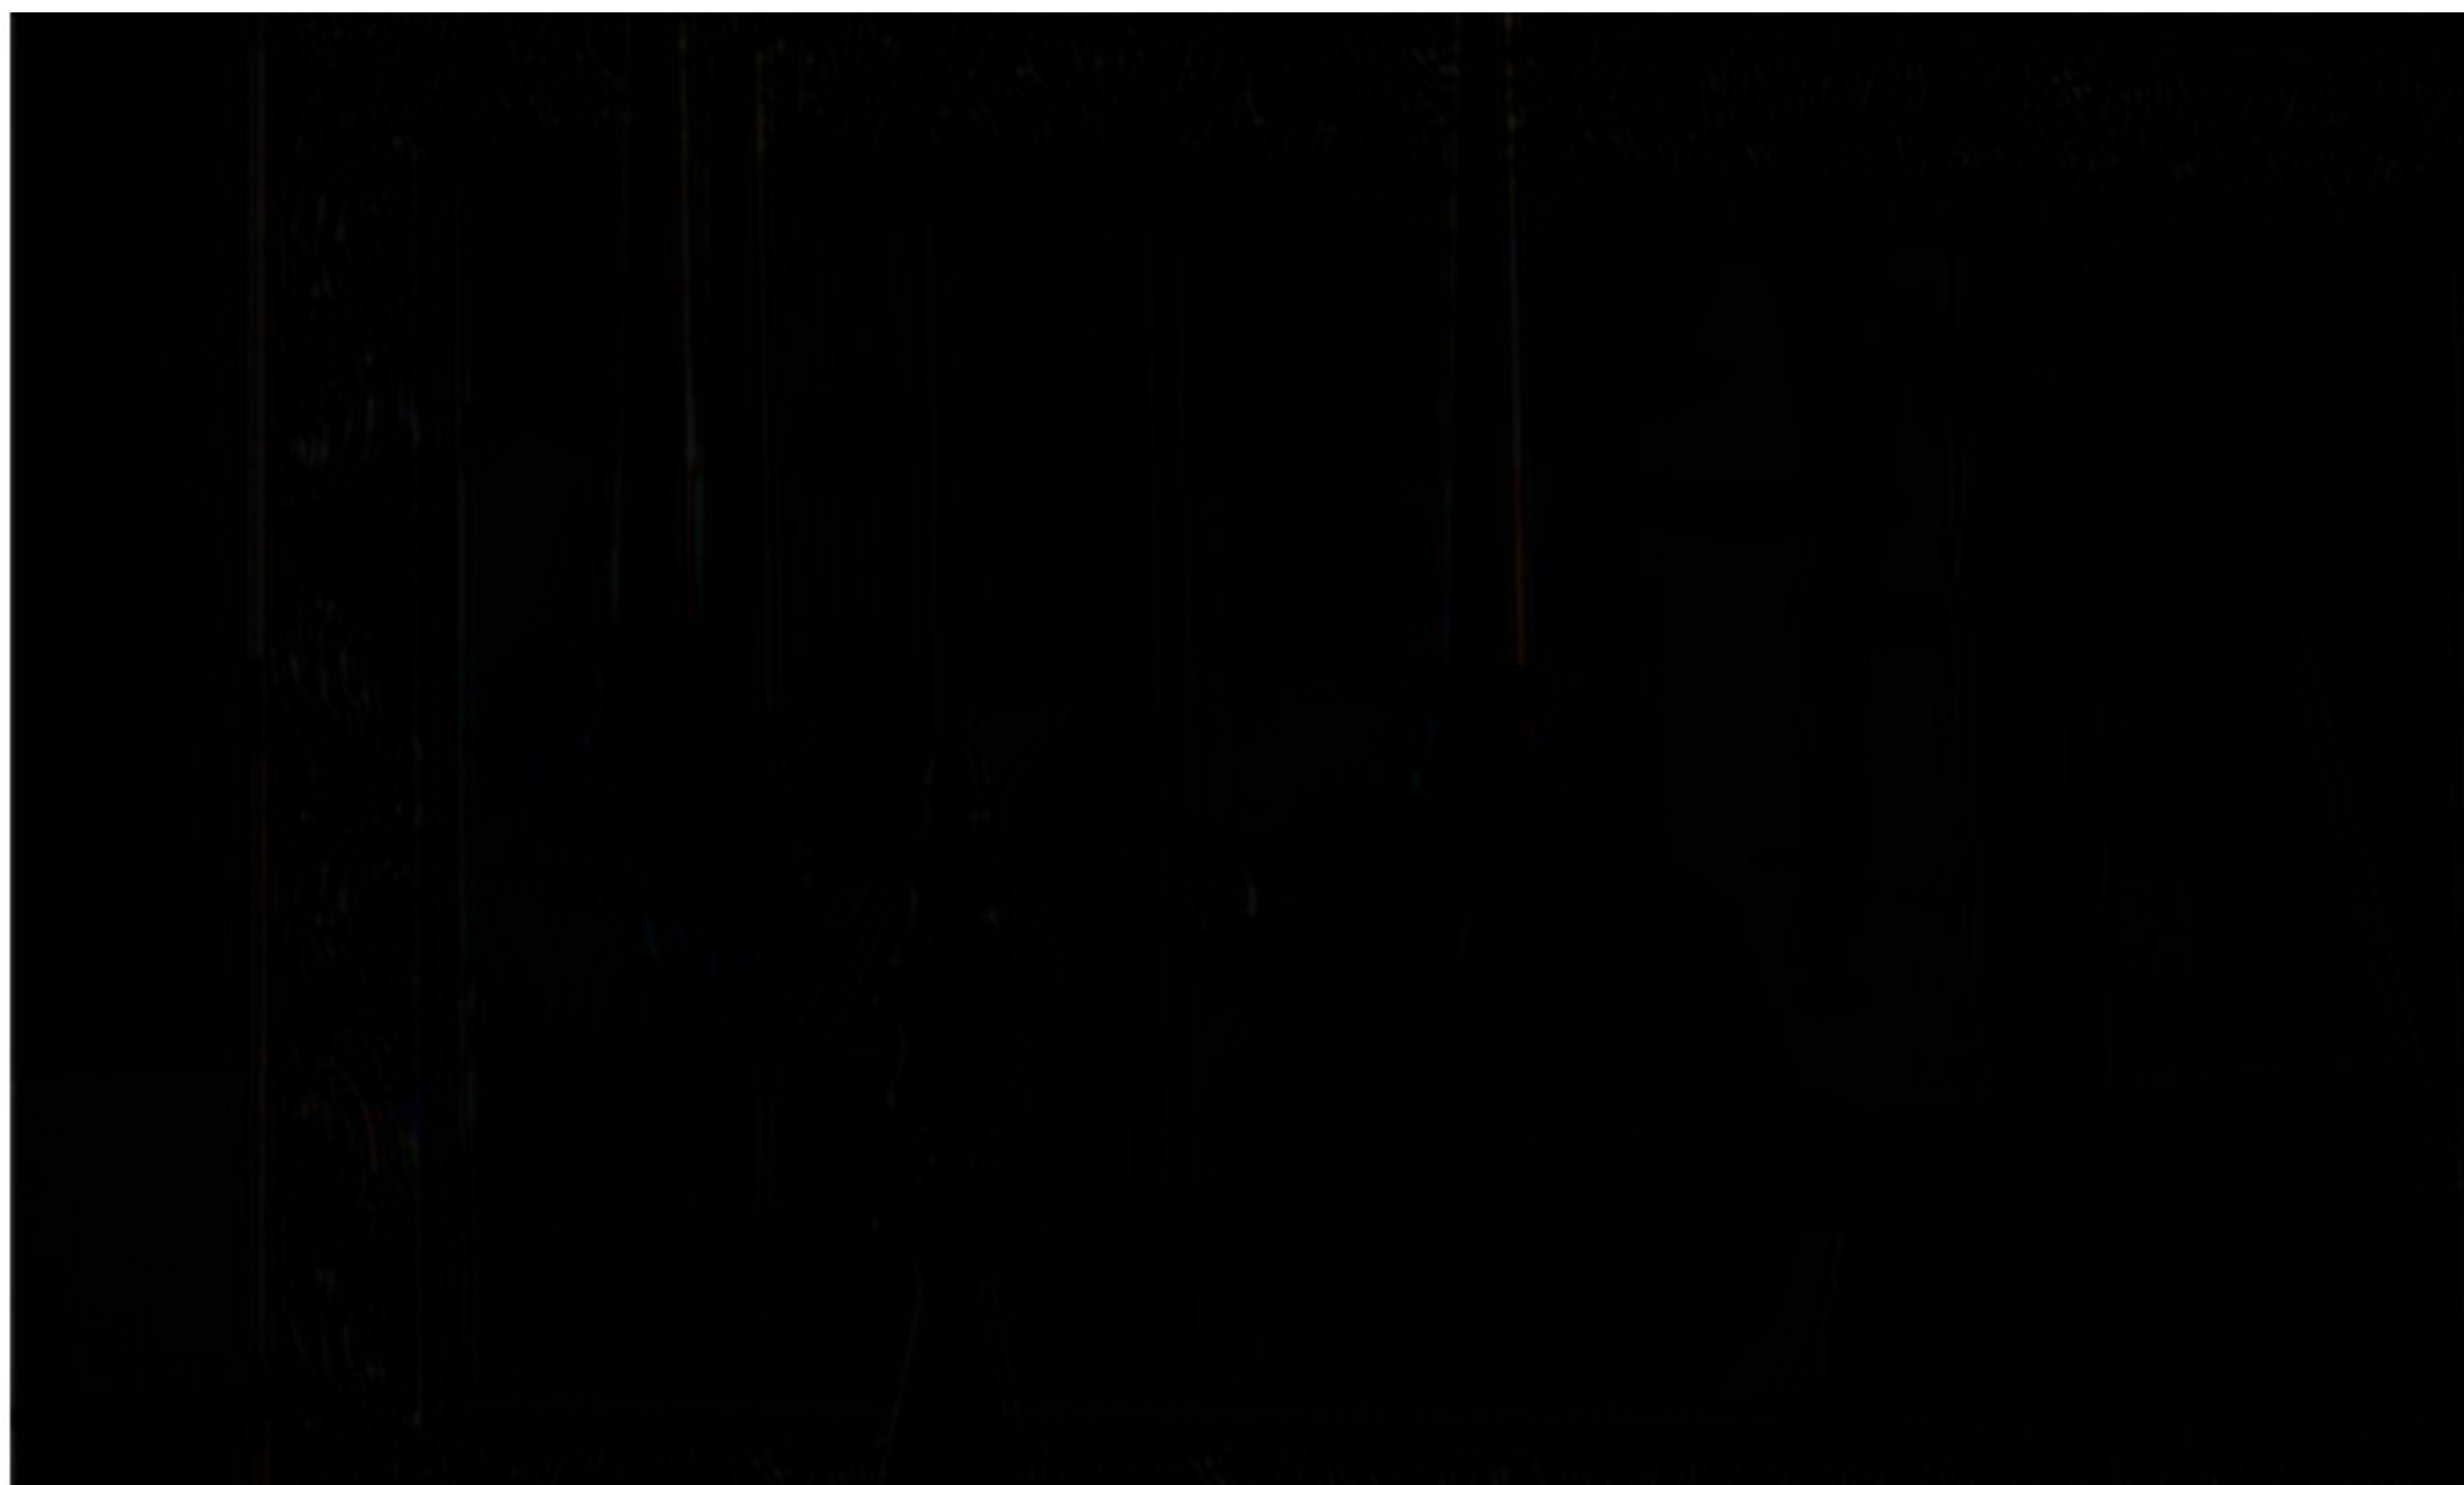

Middle View

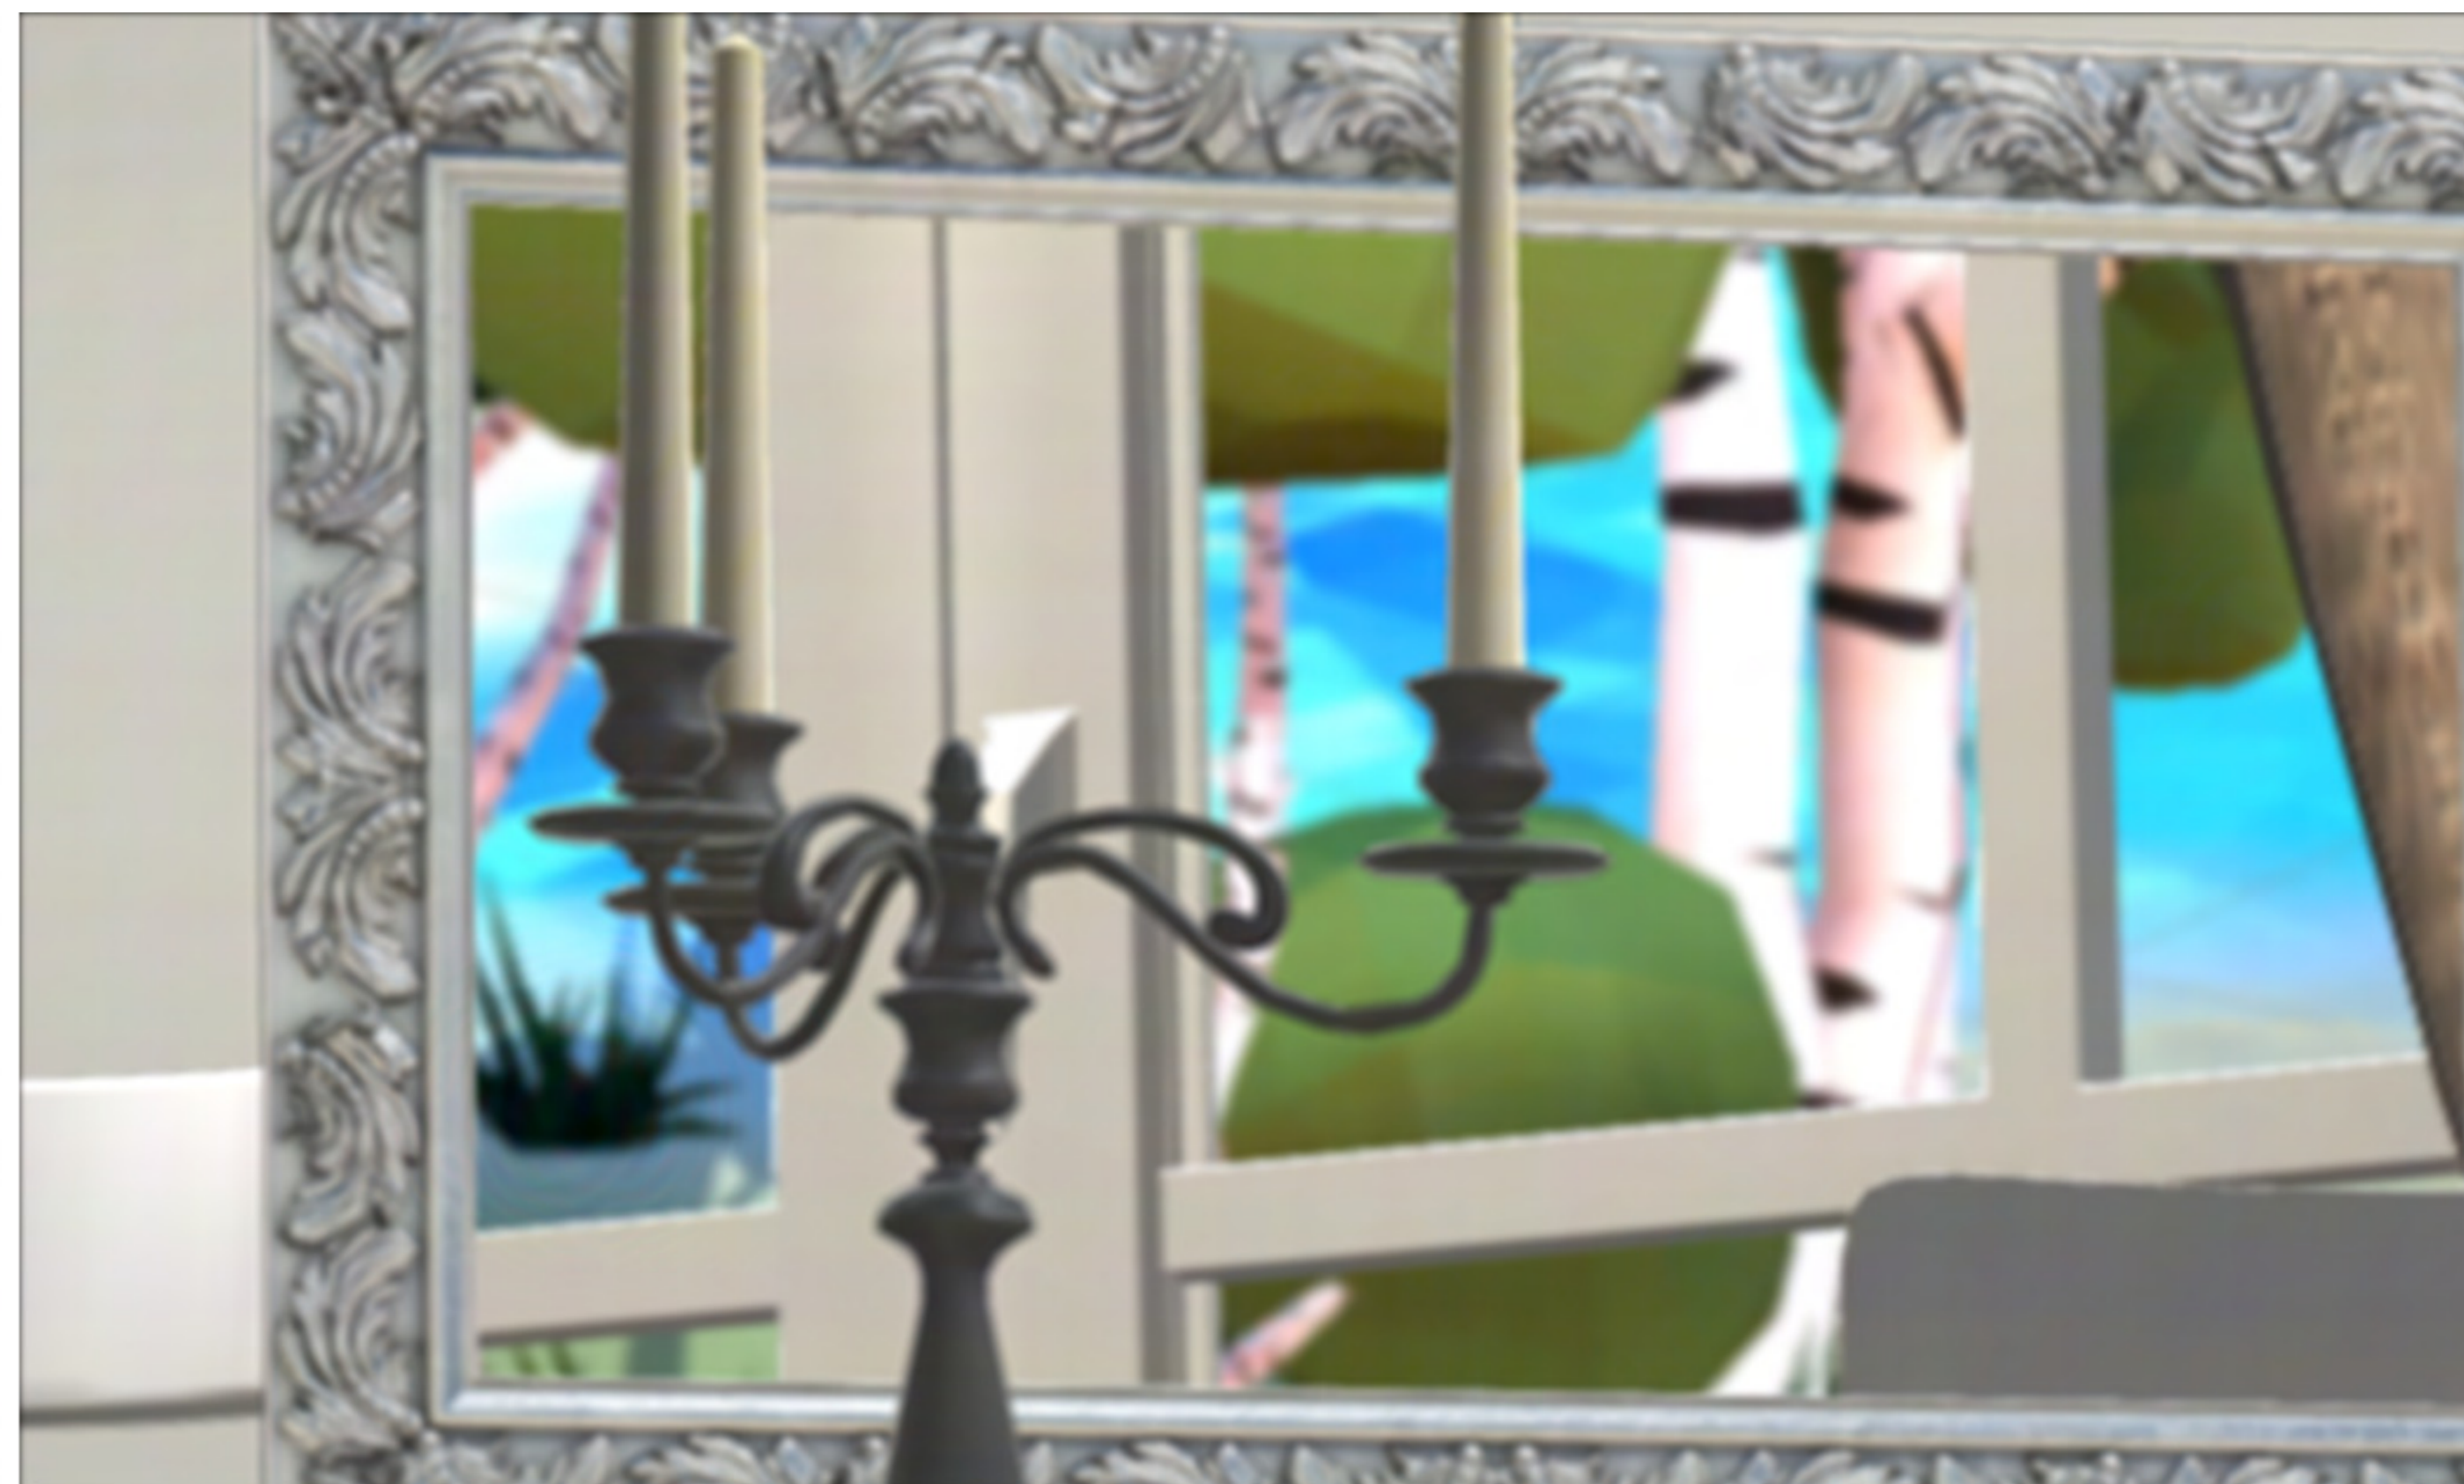

Right View

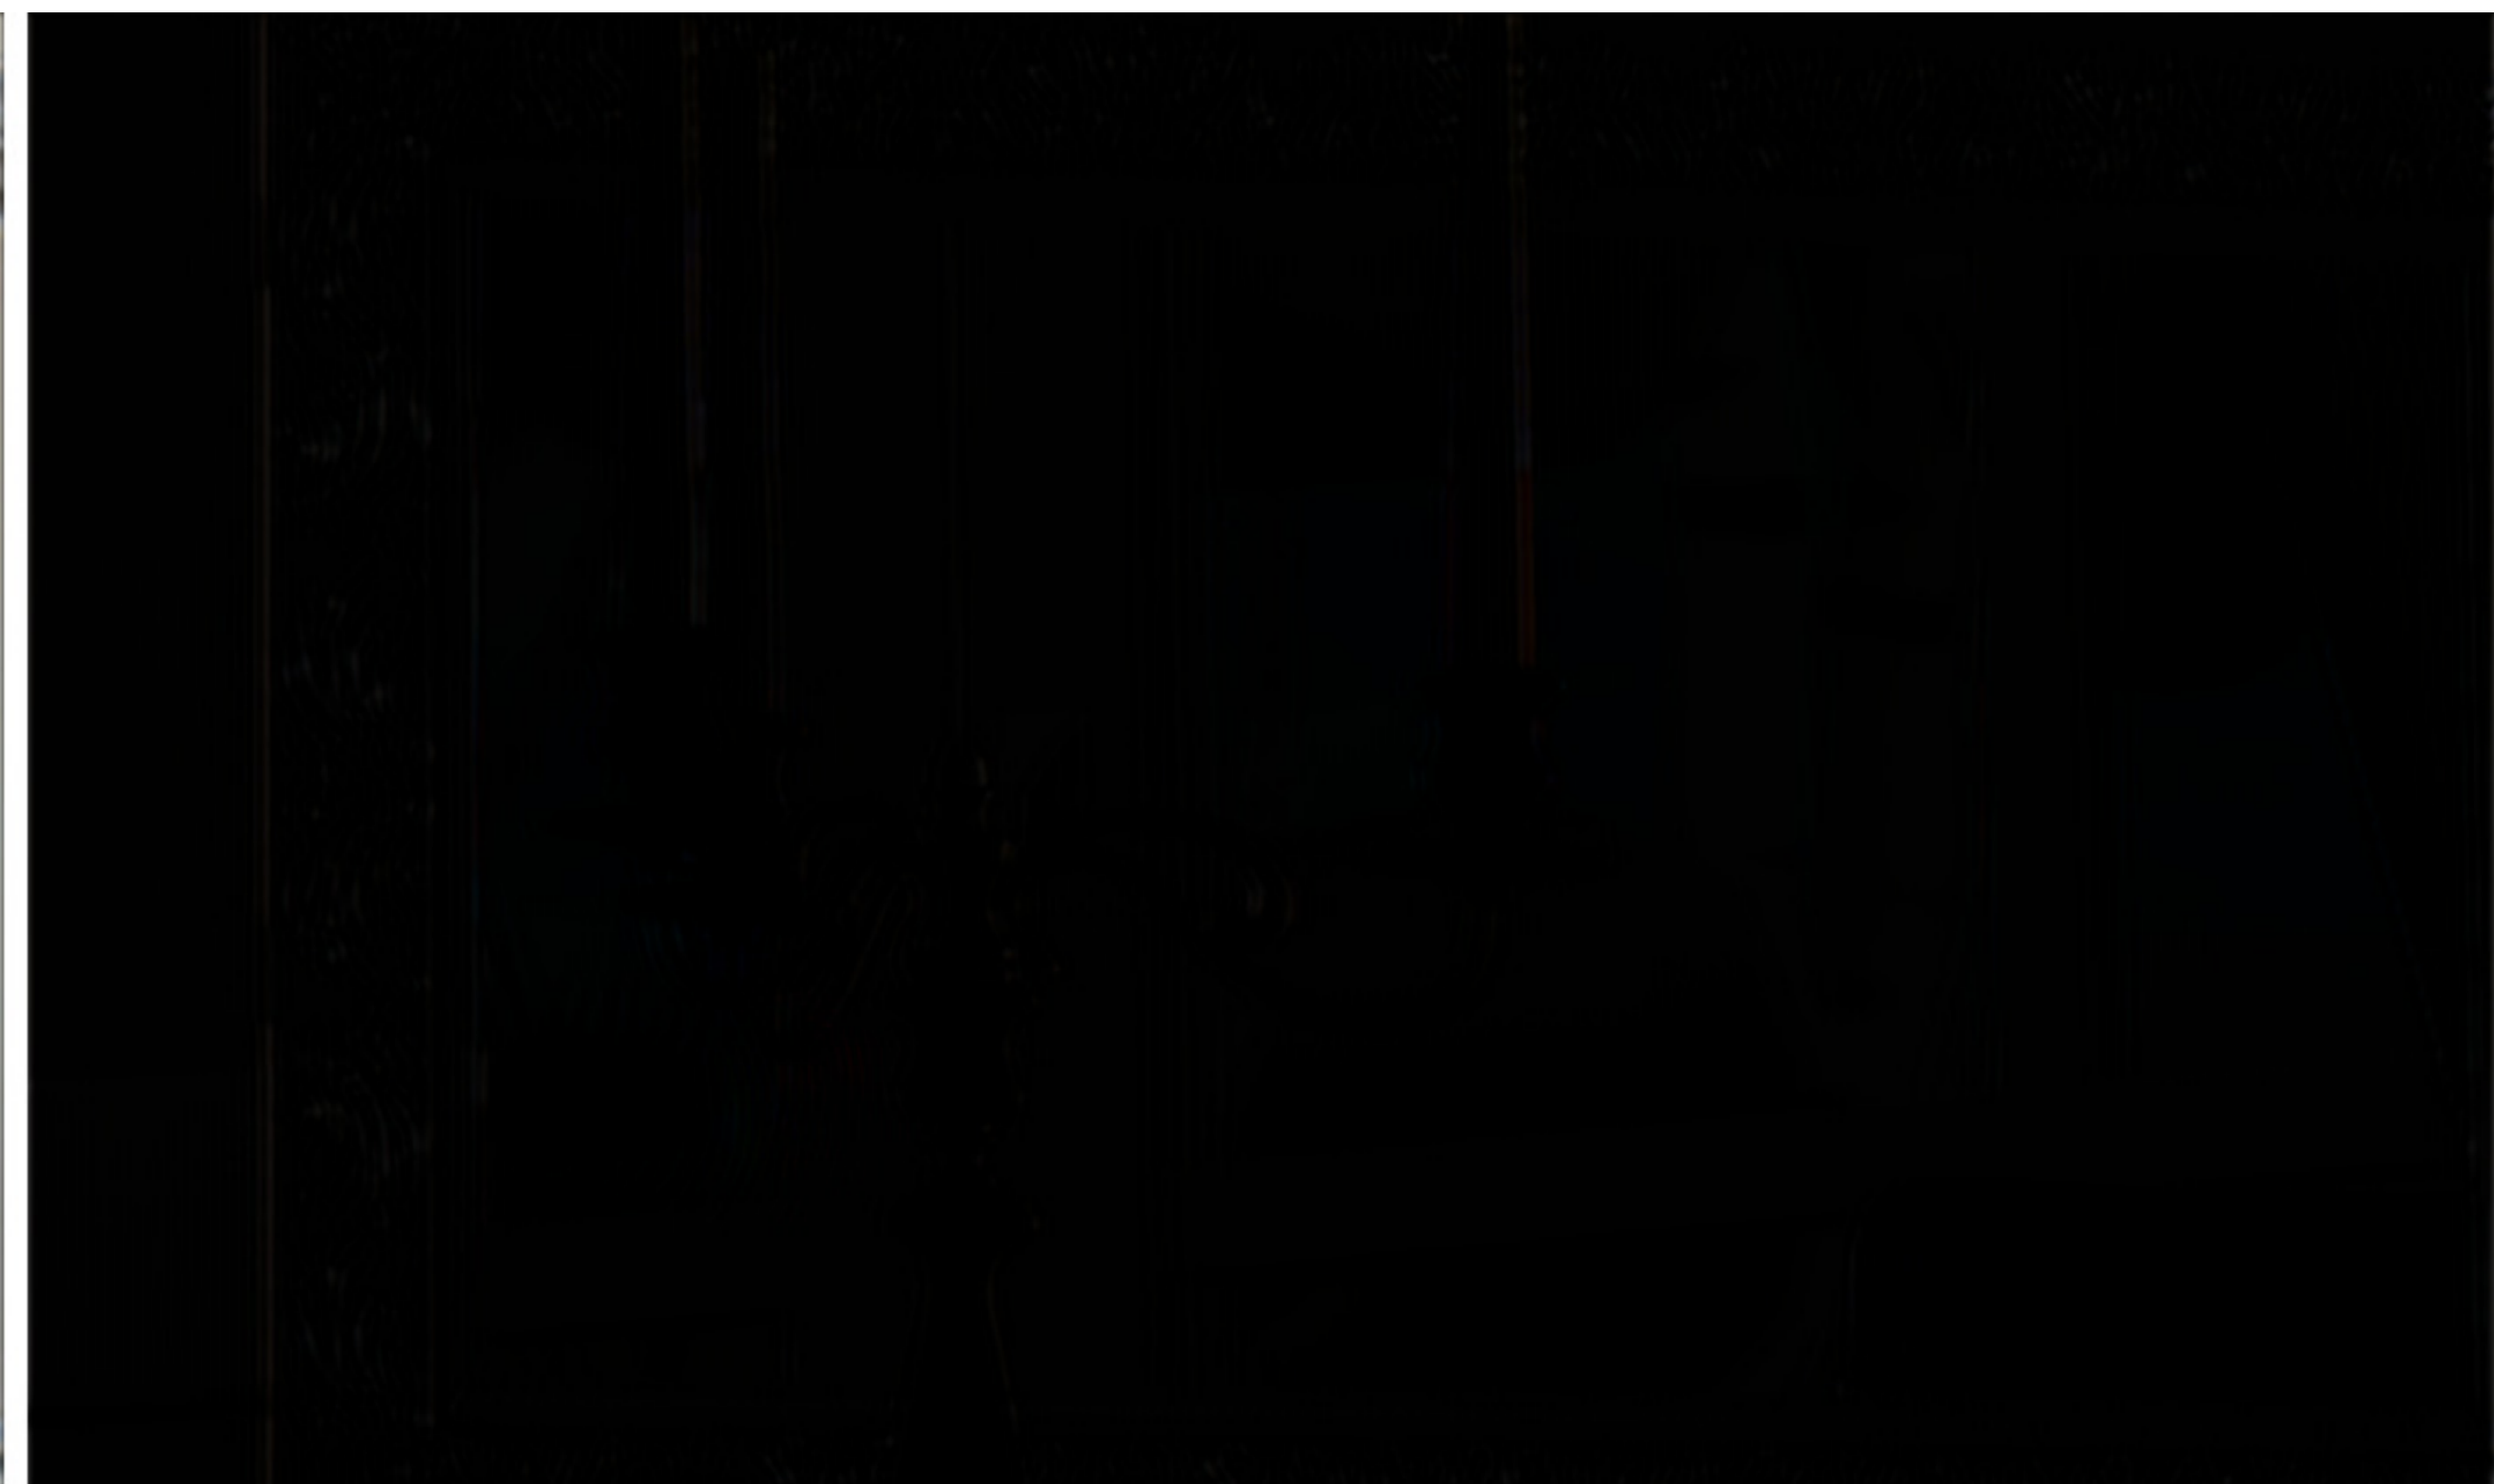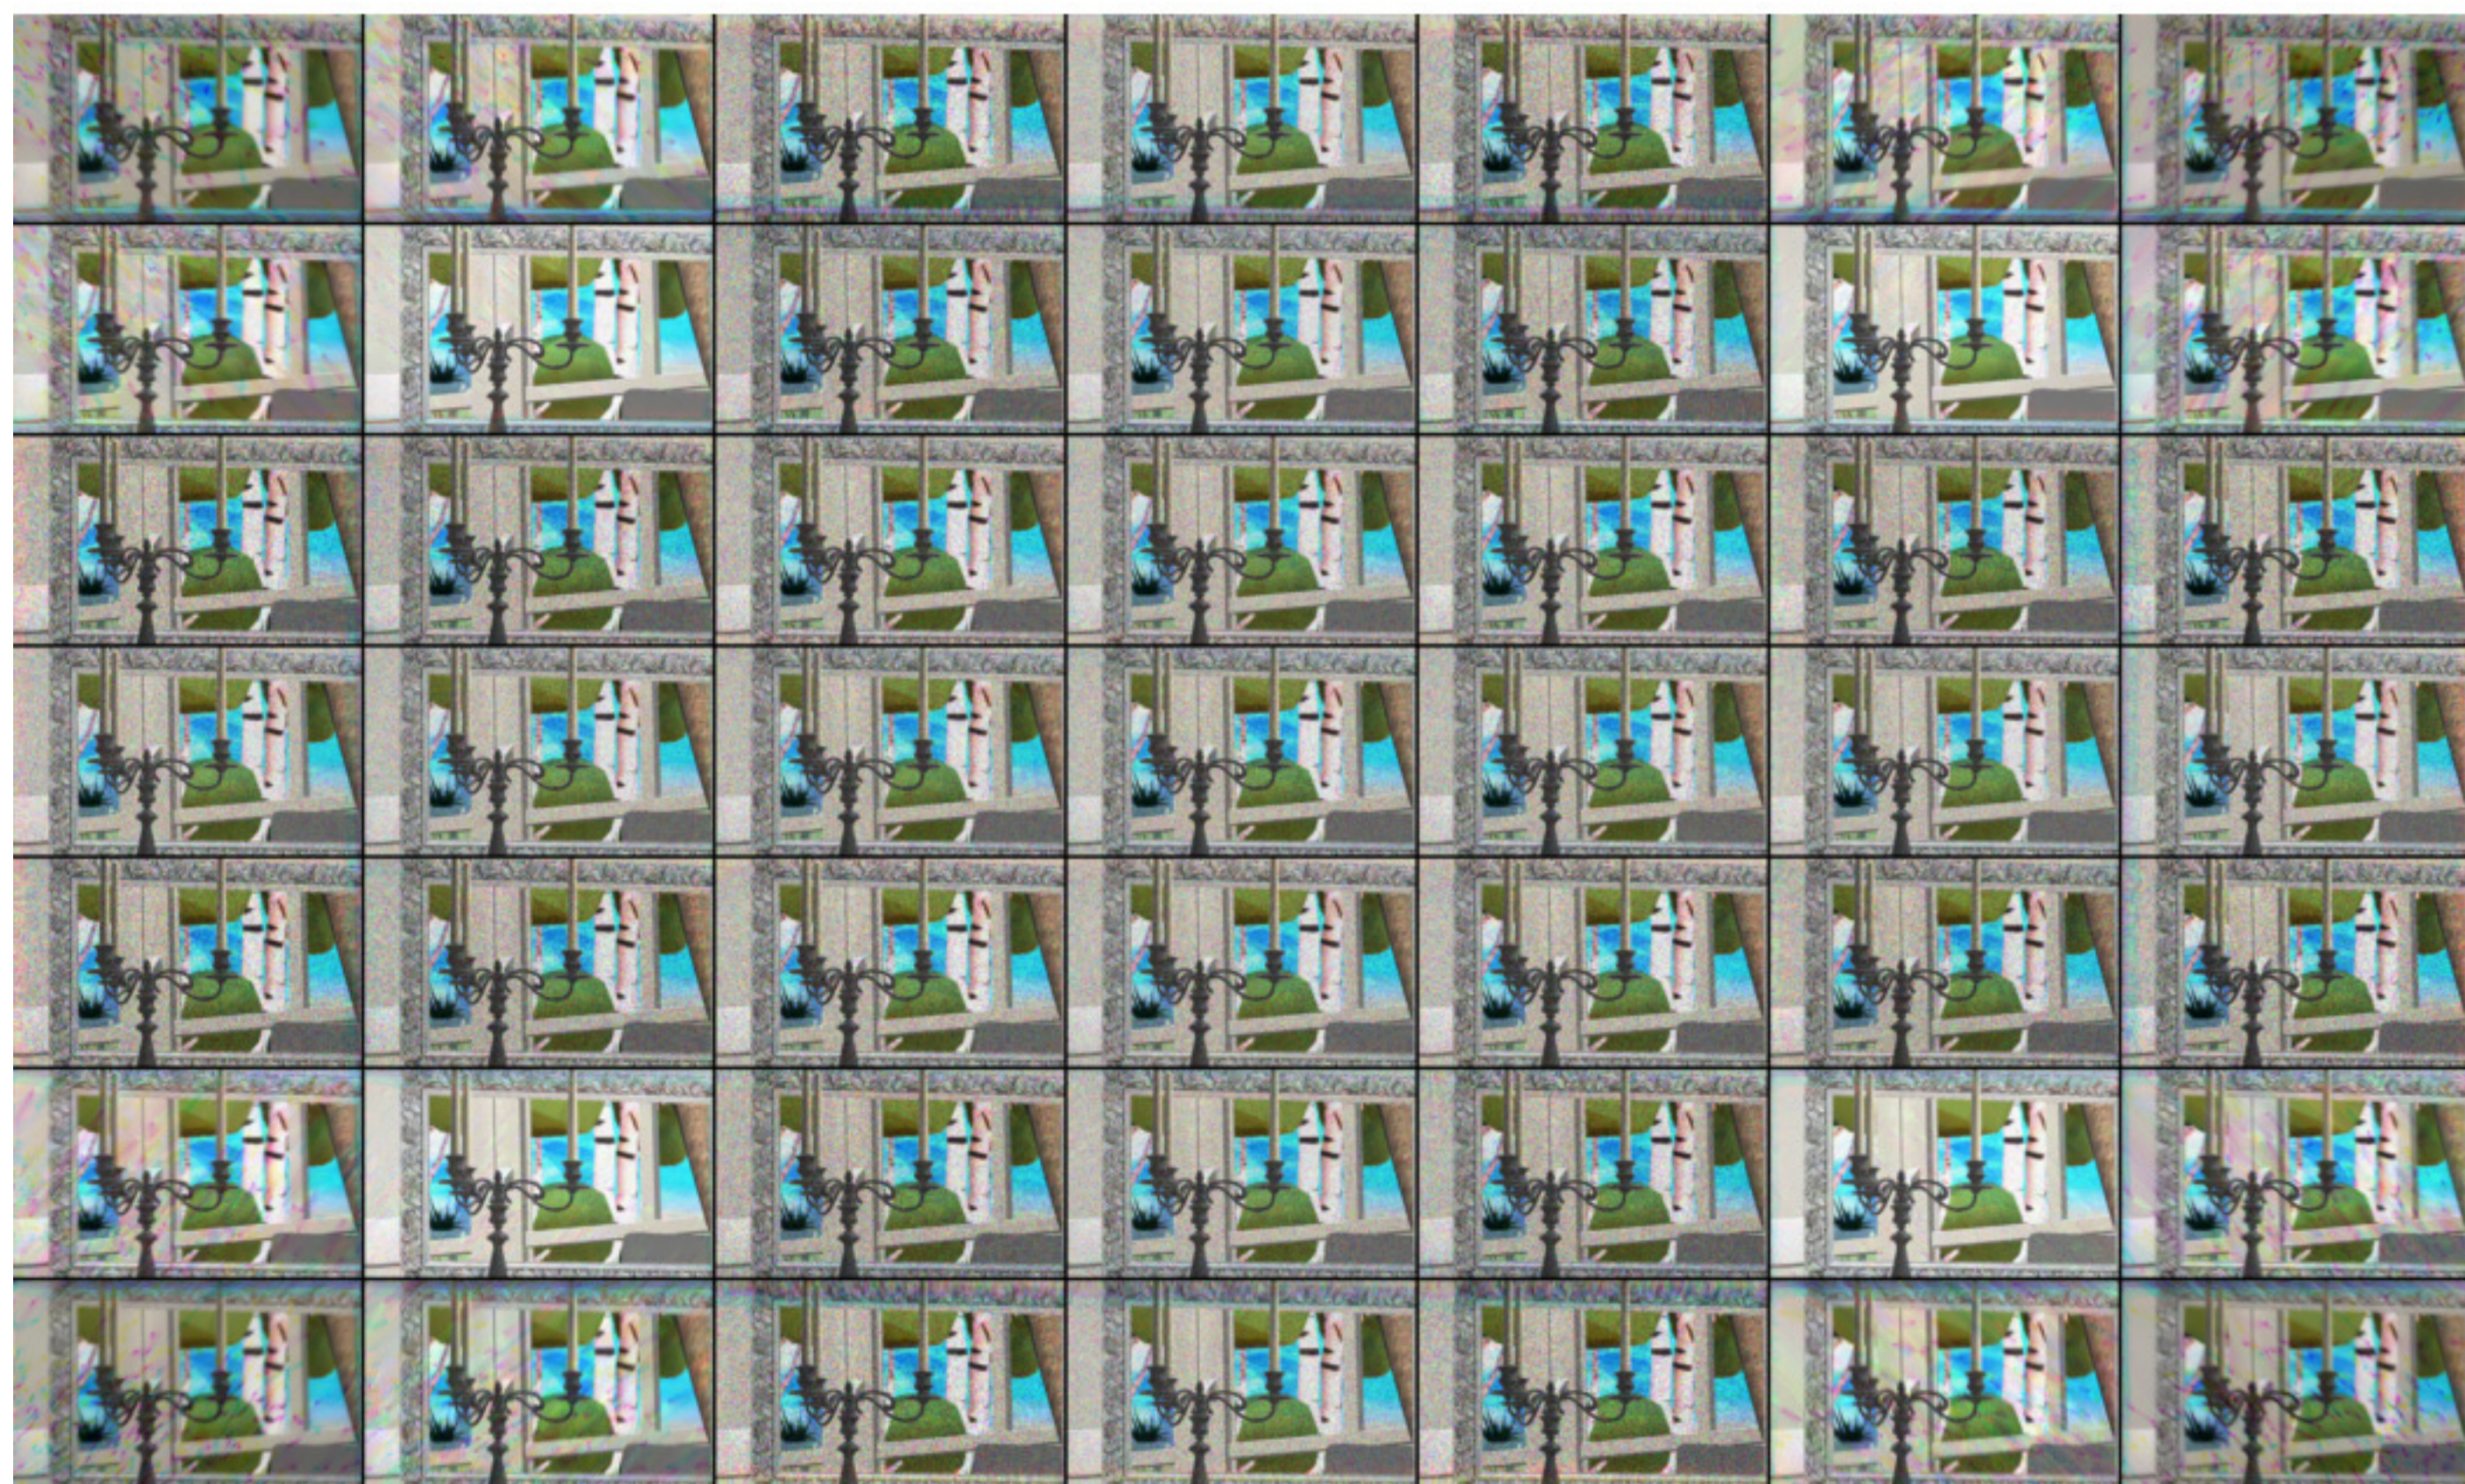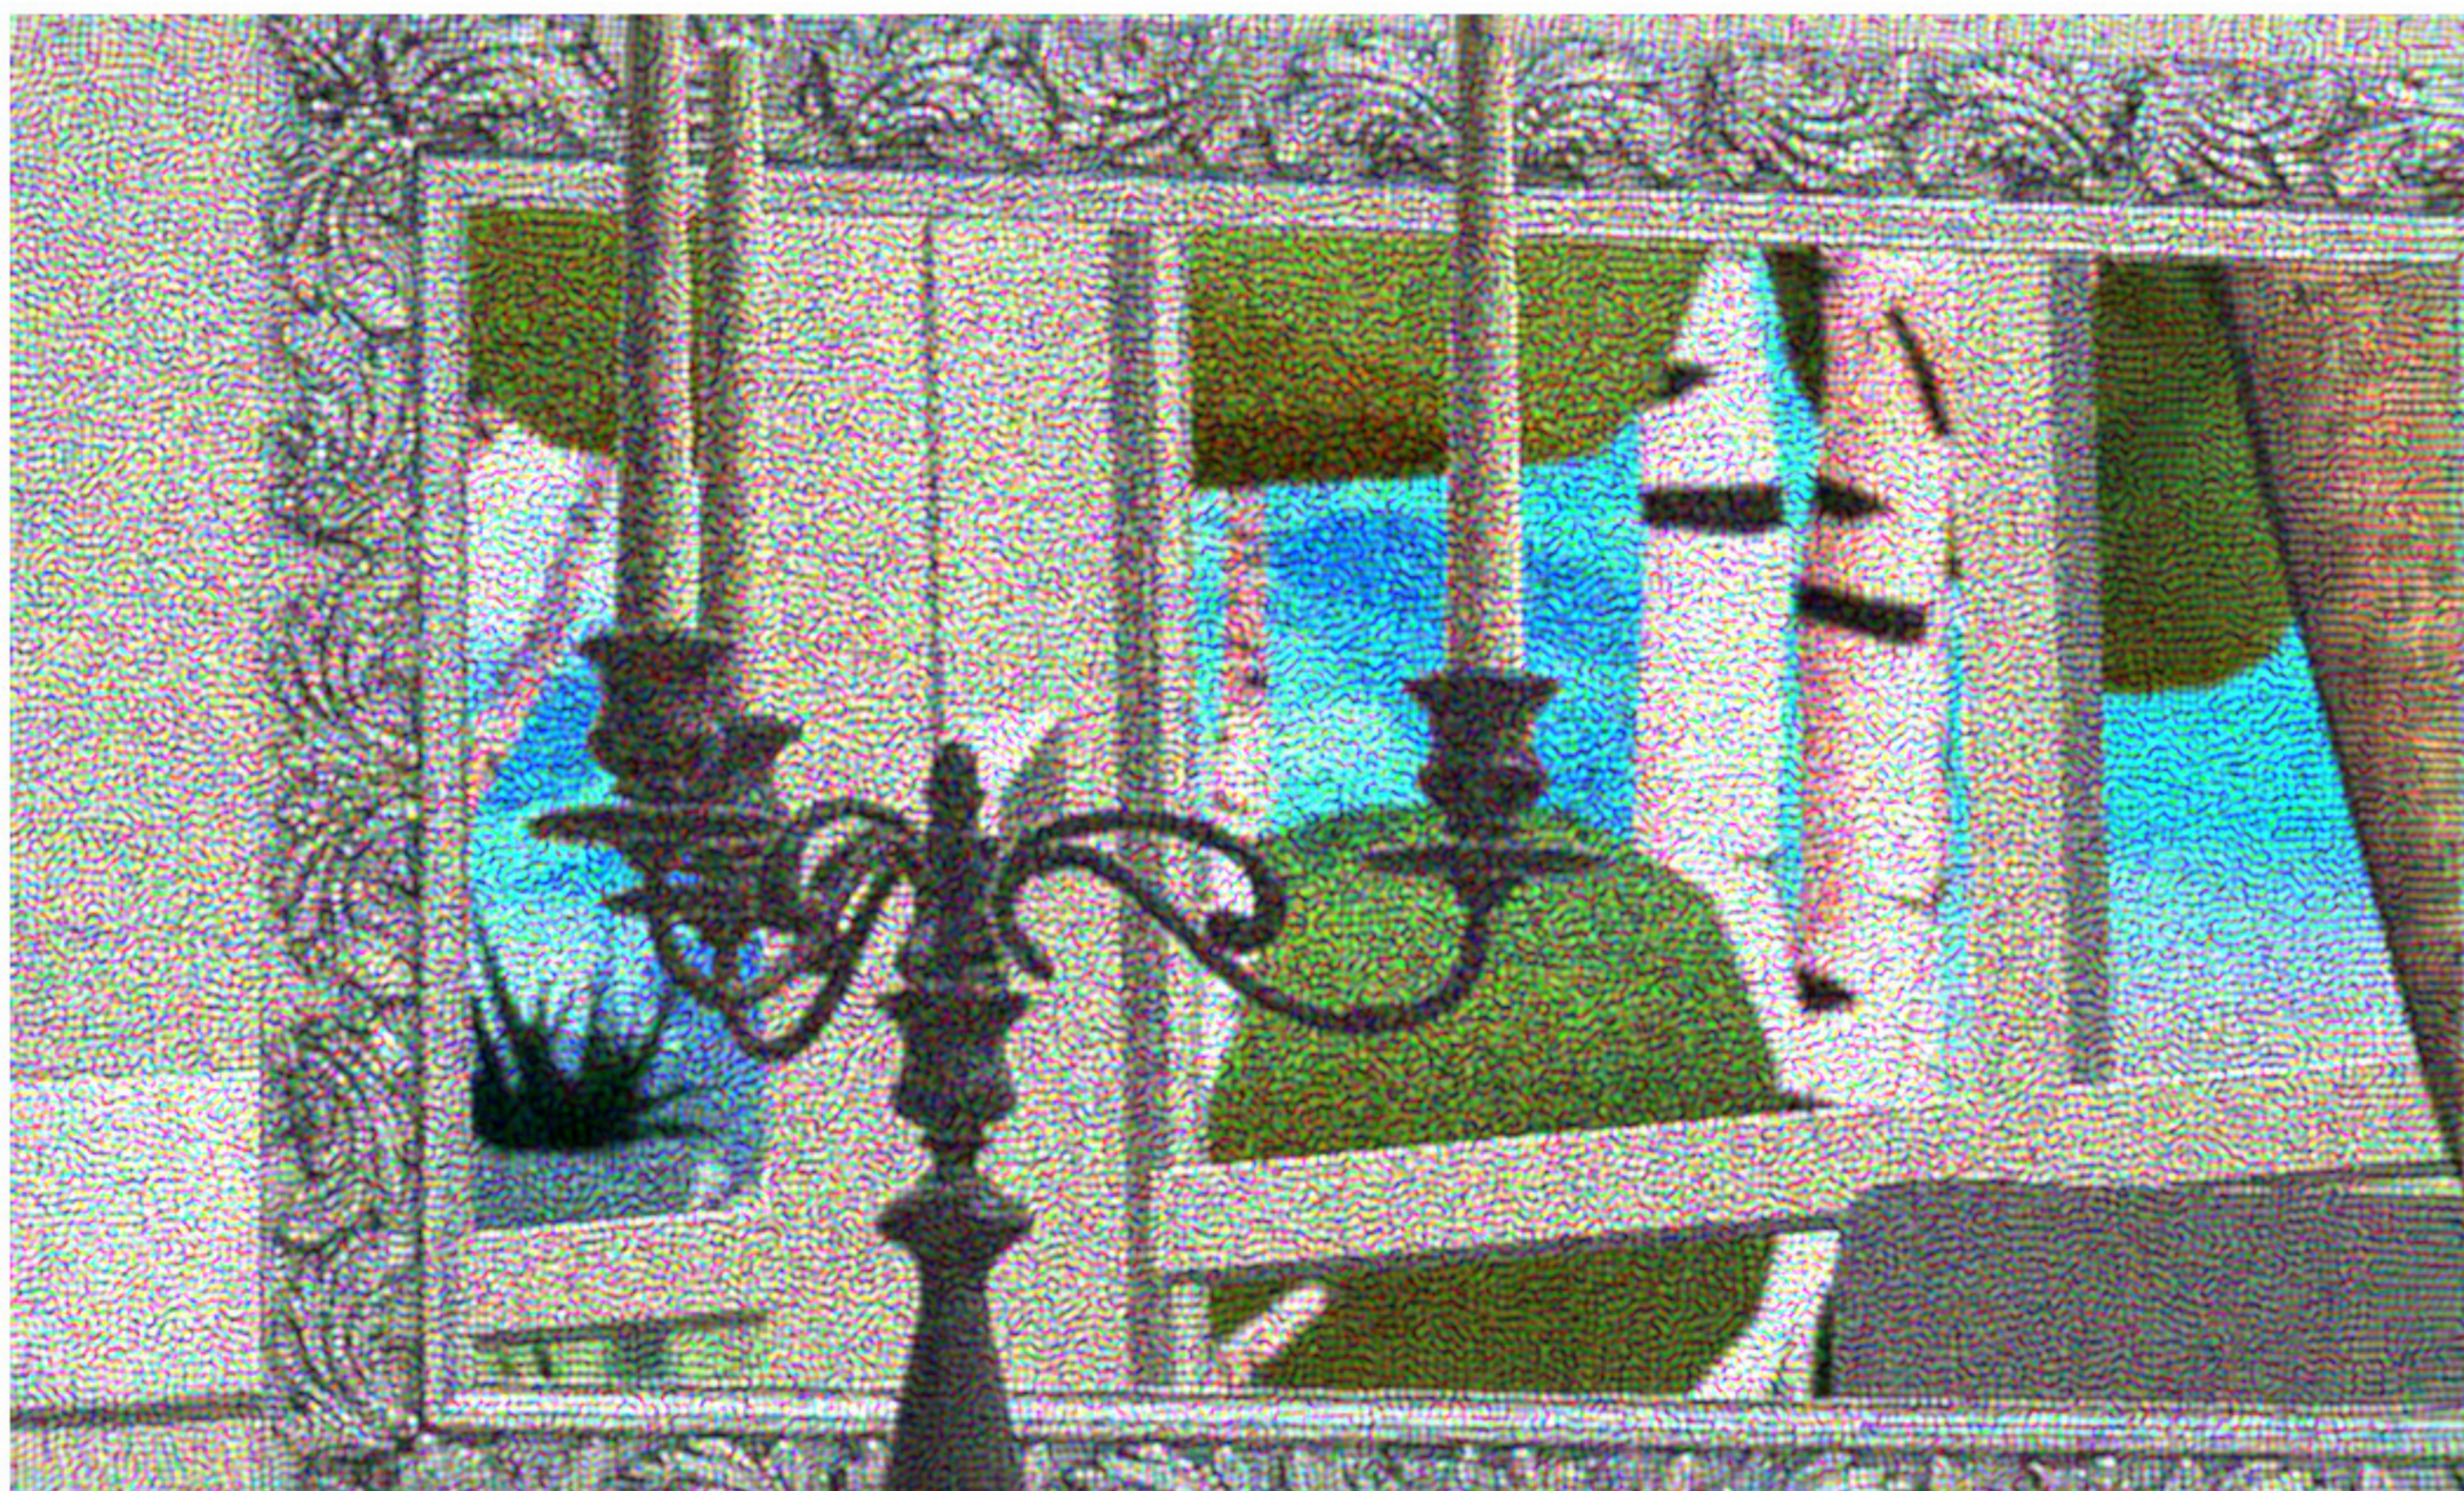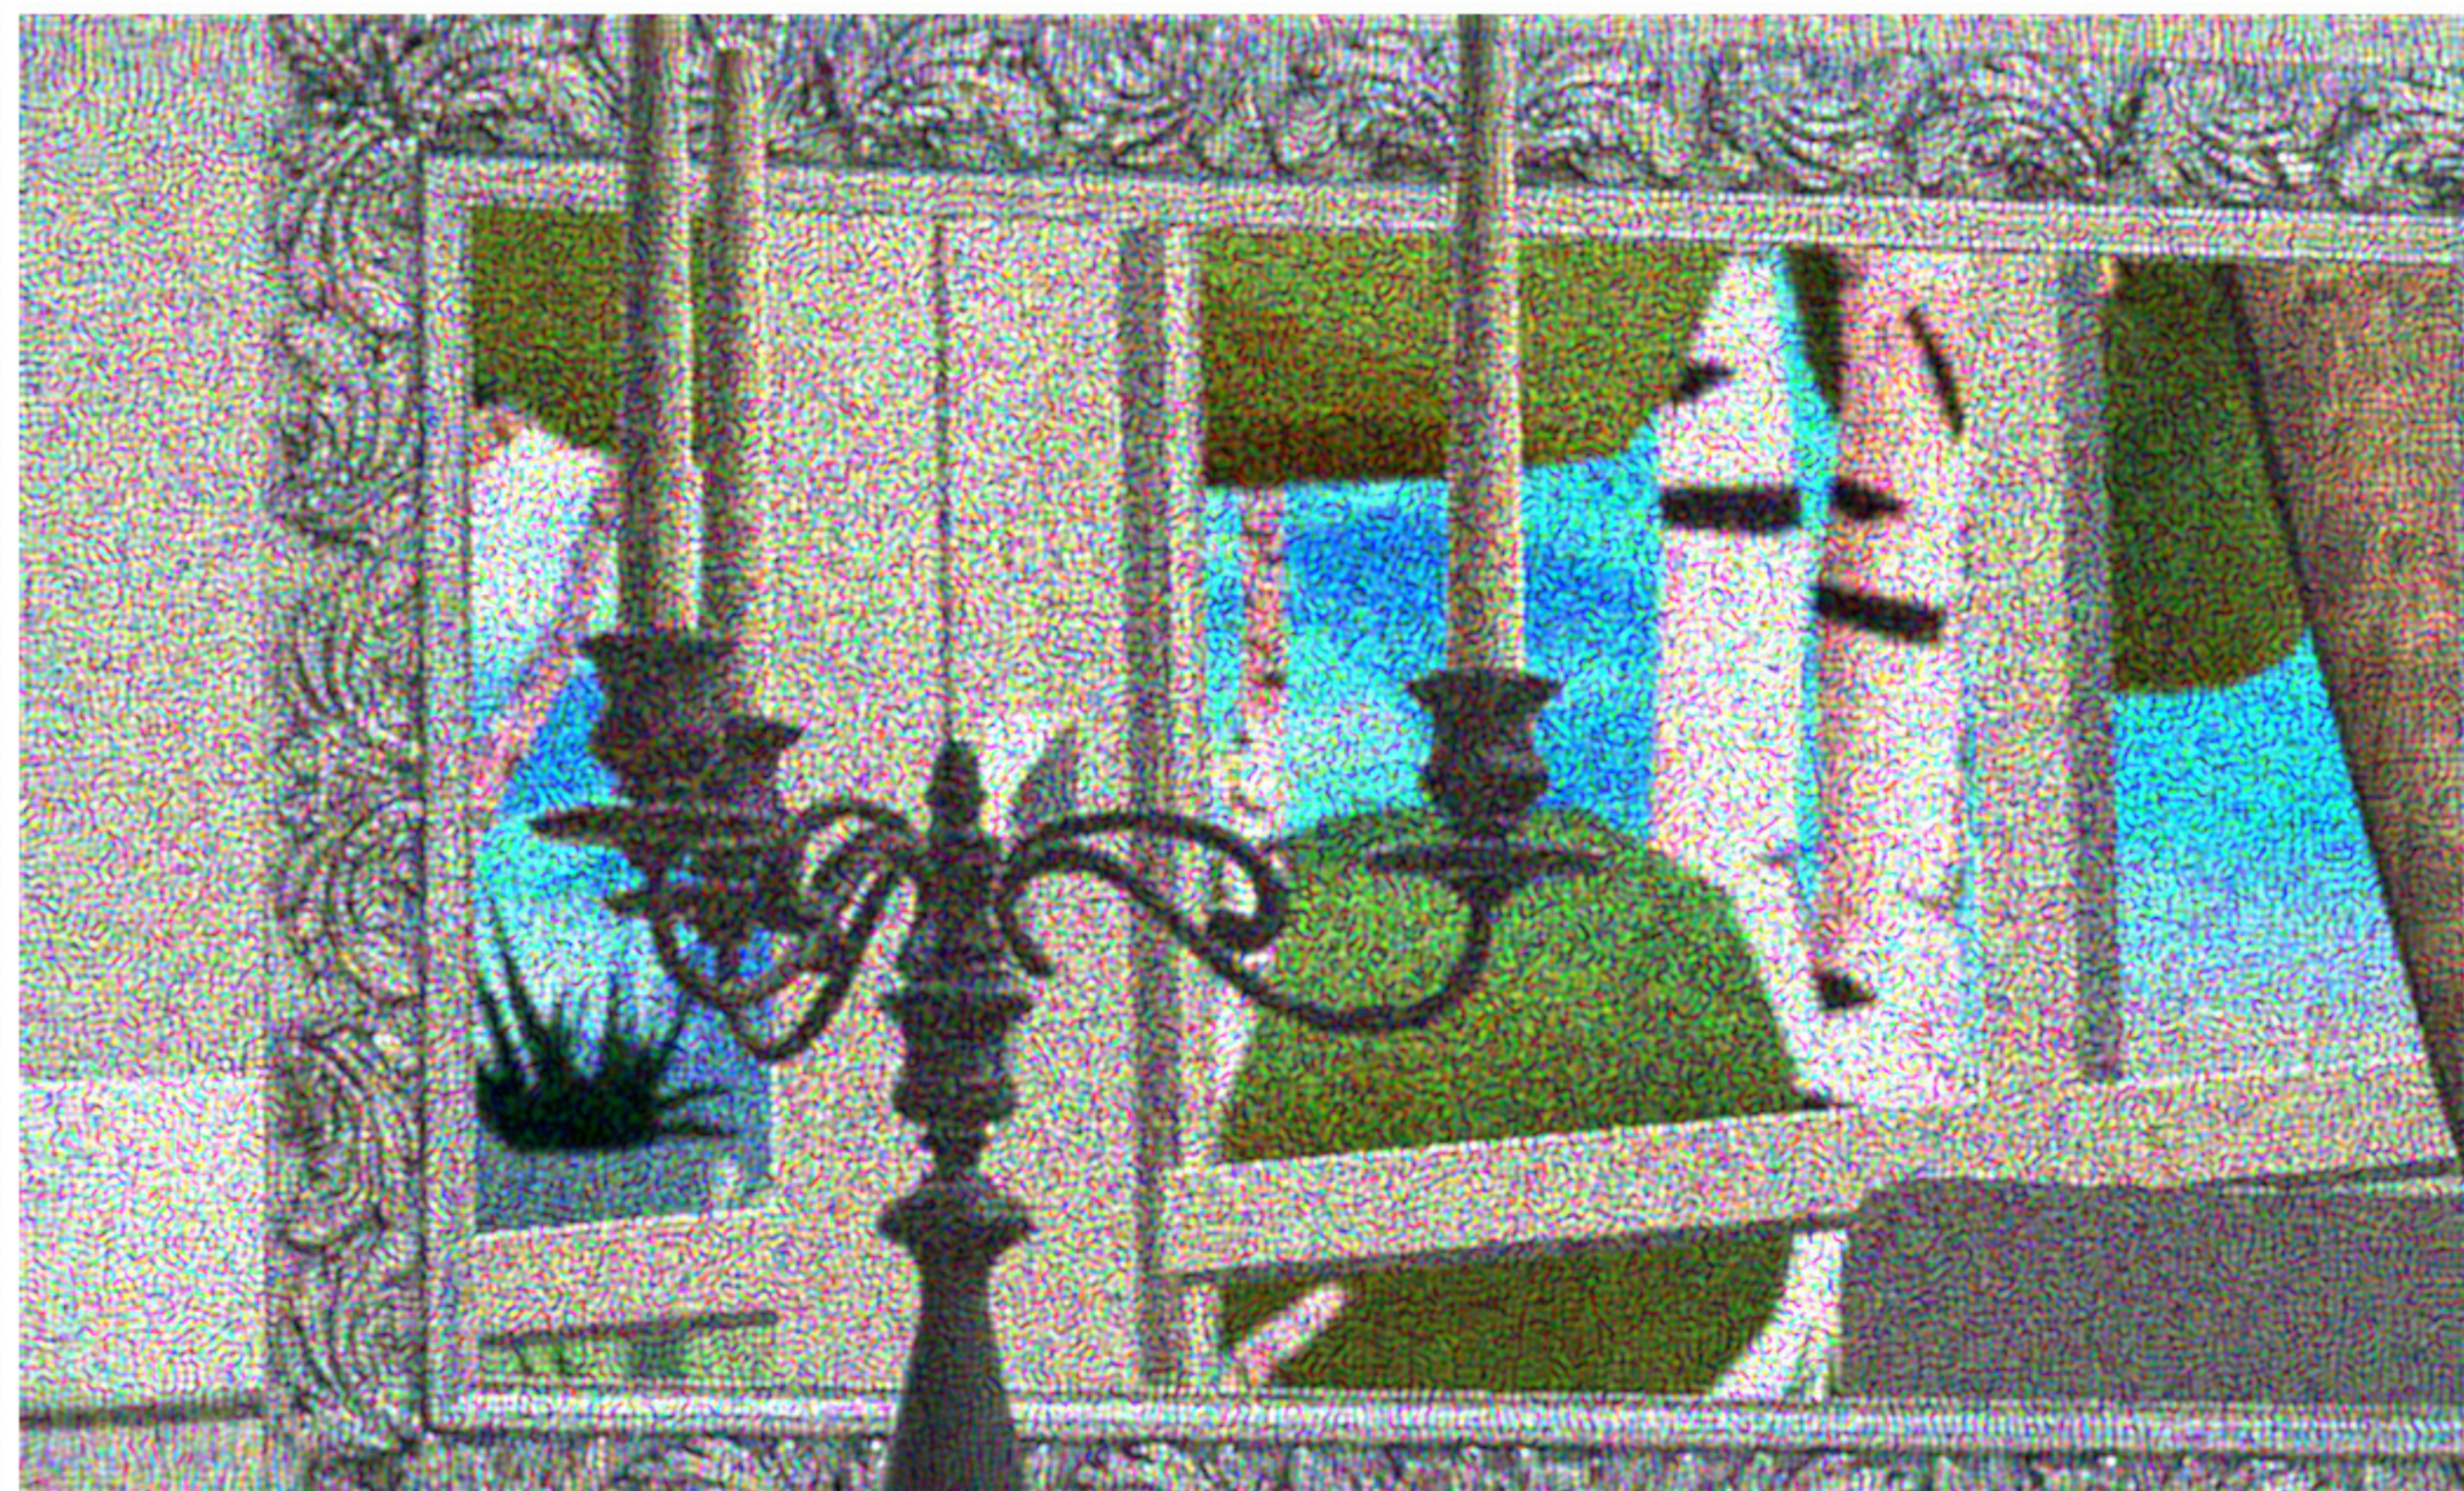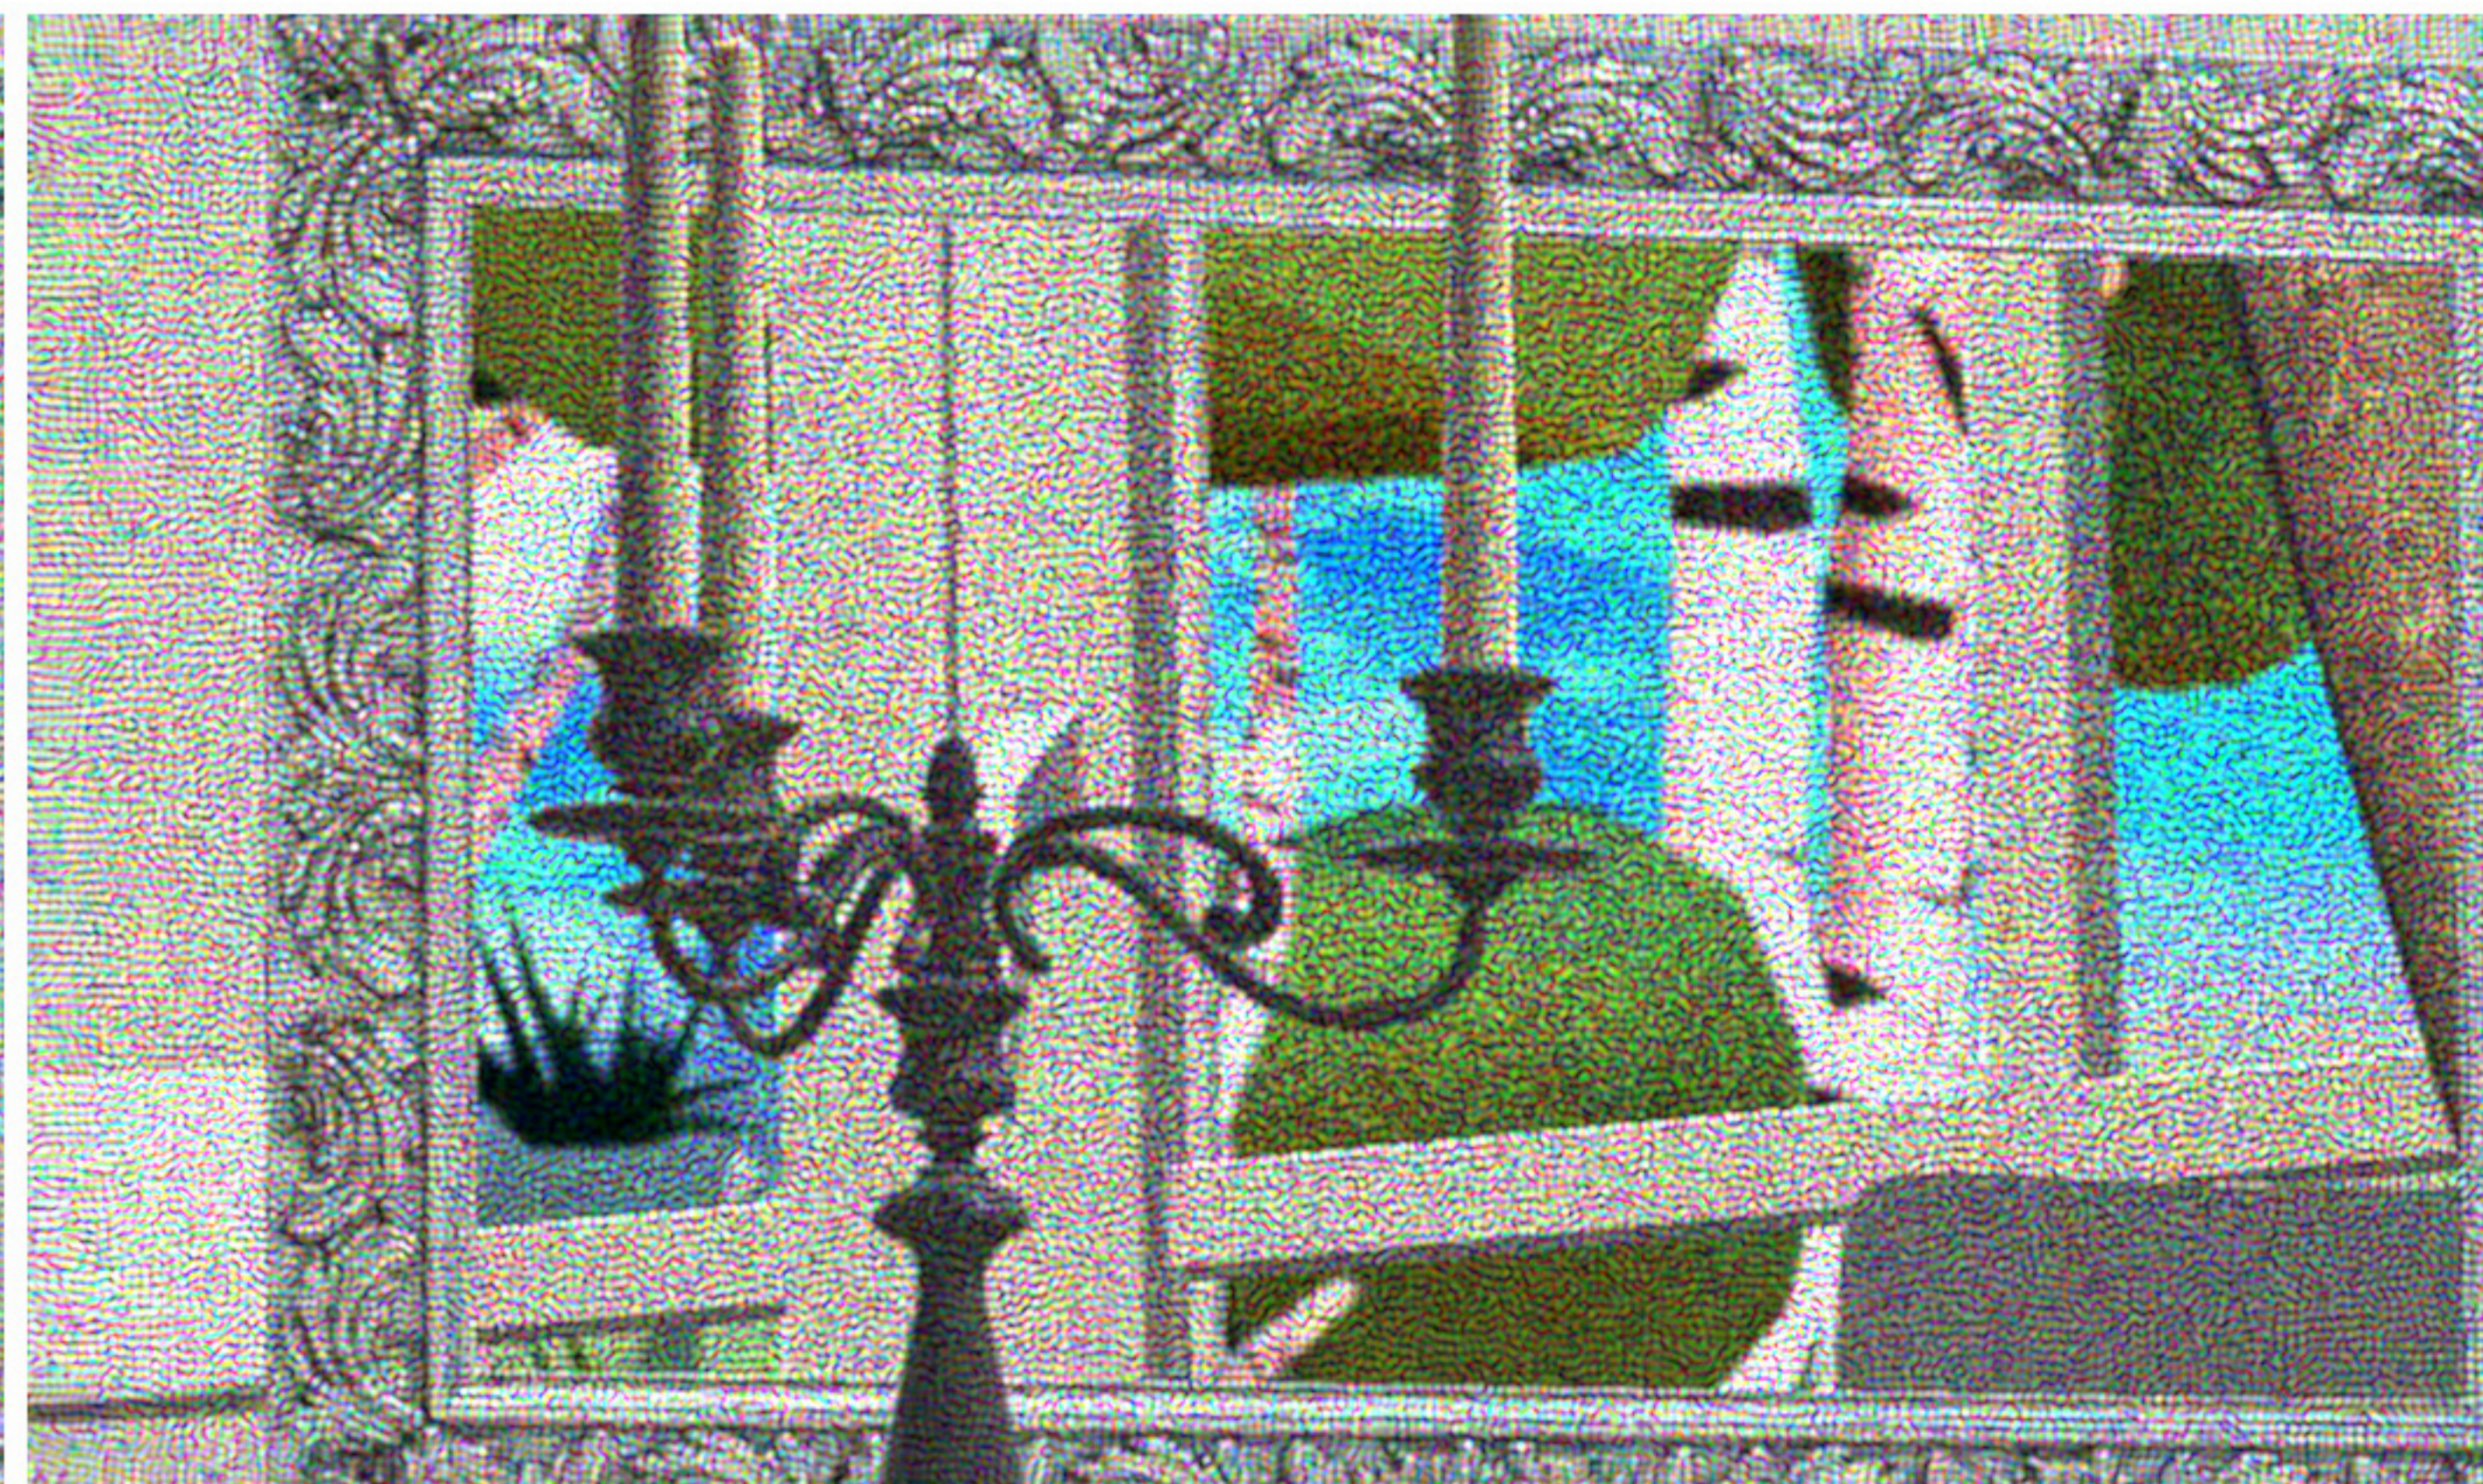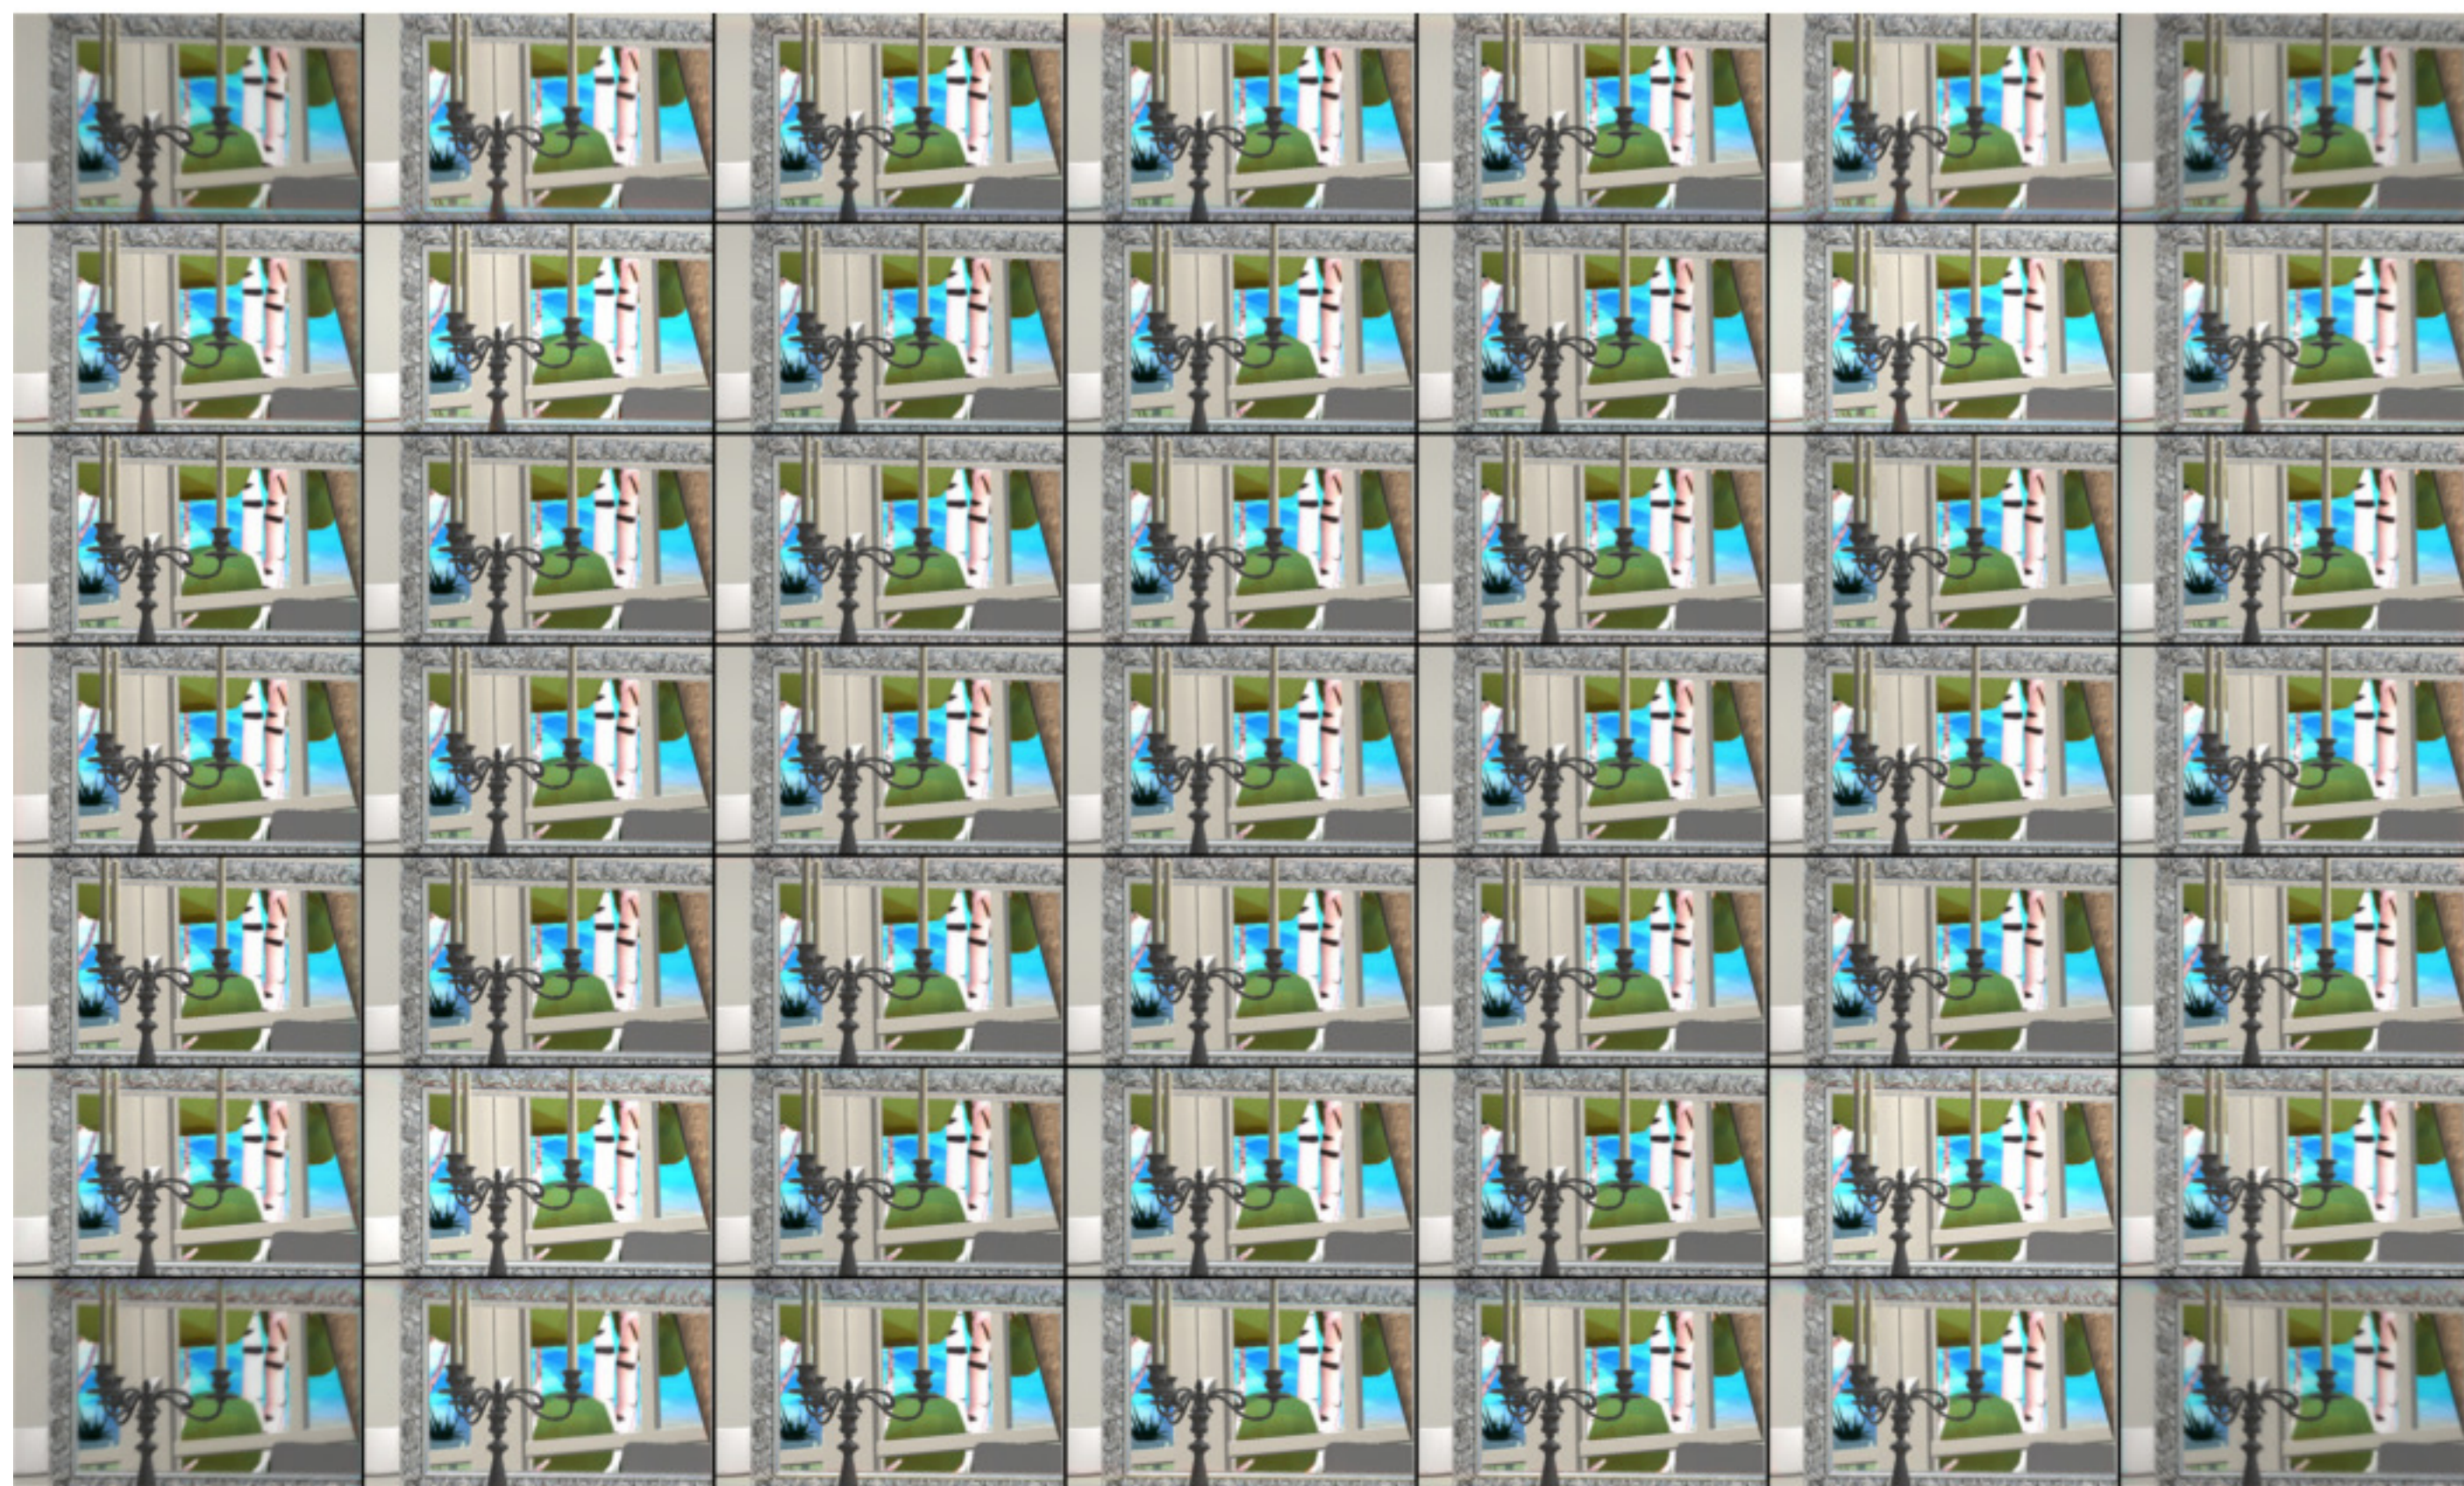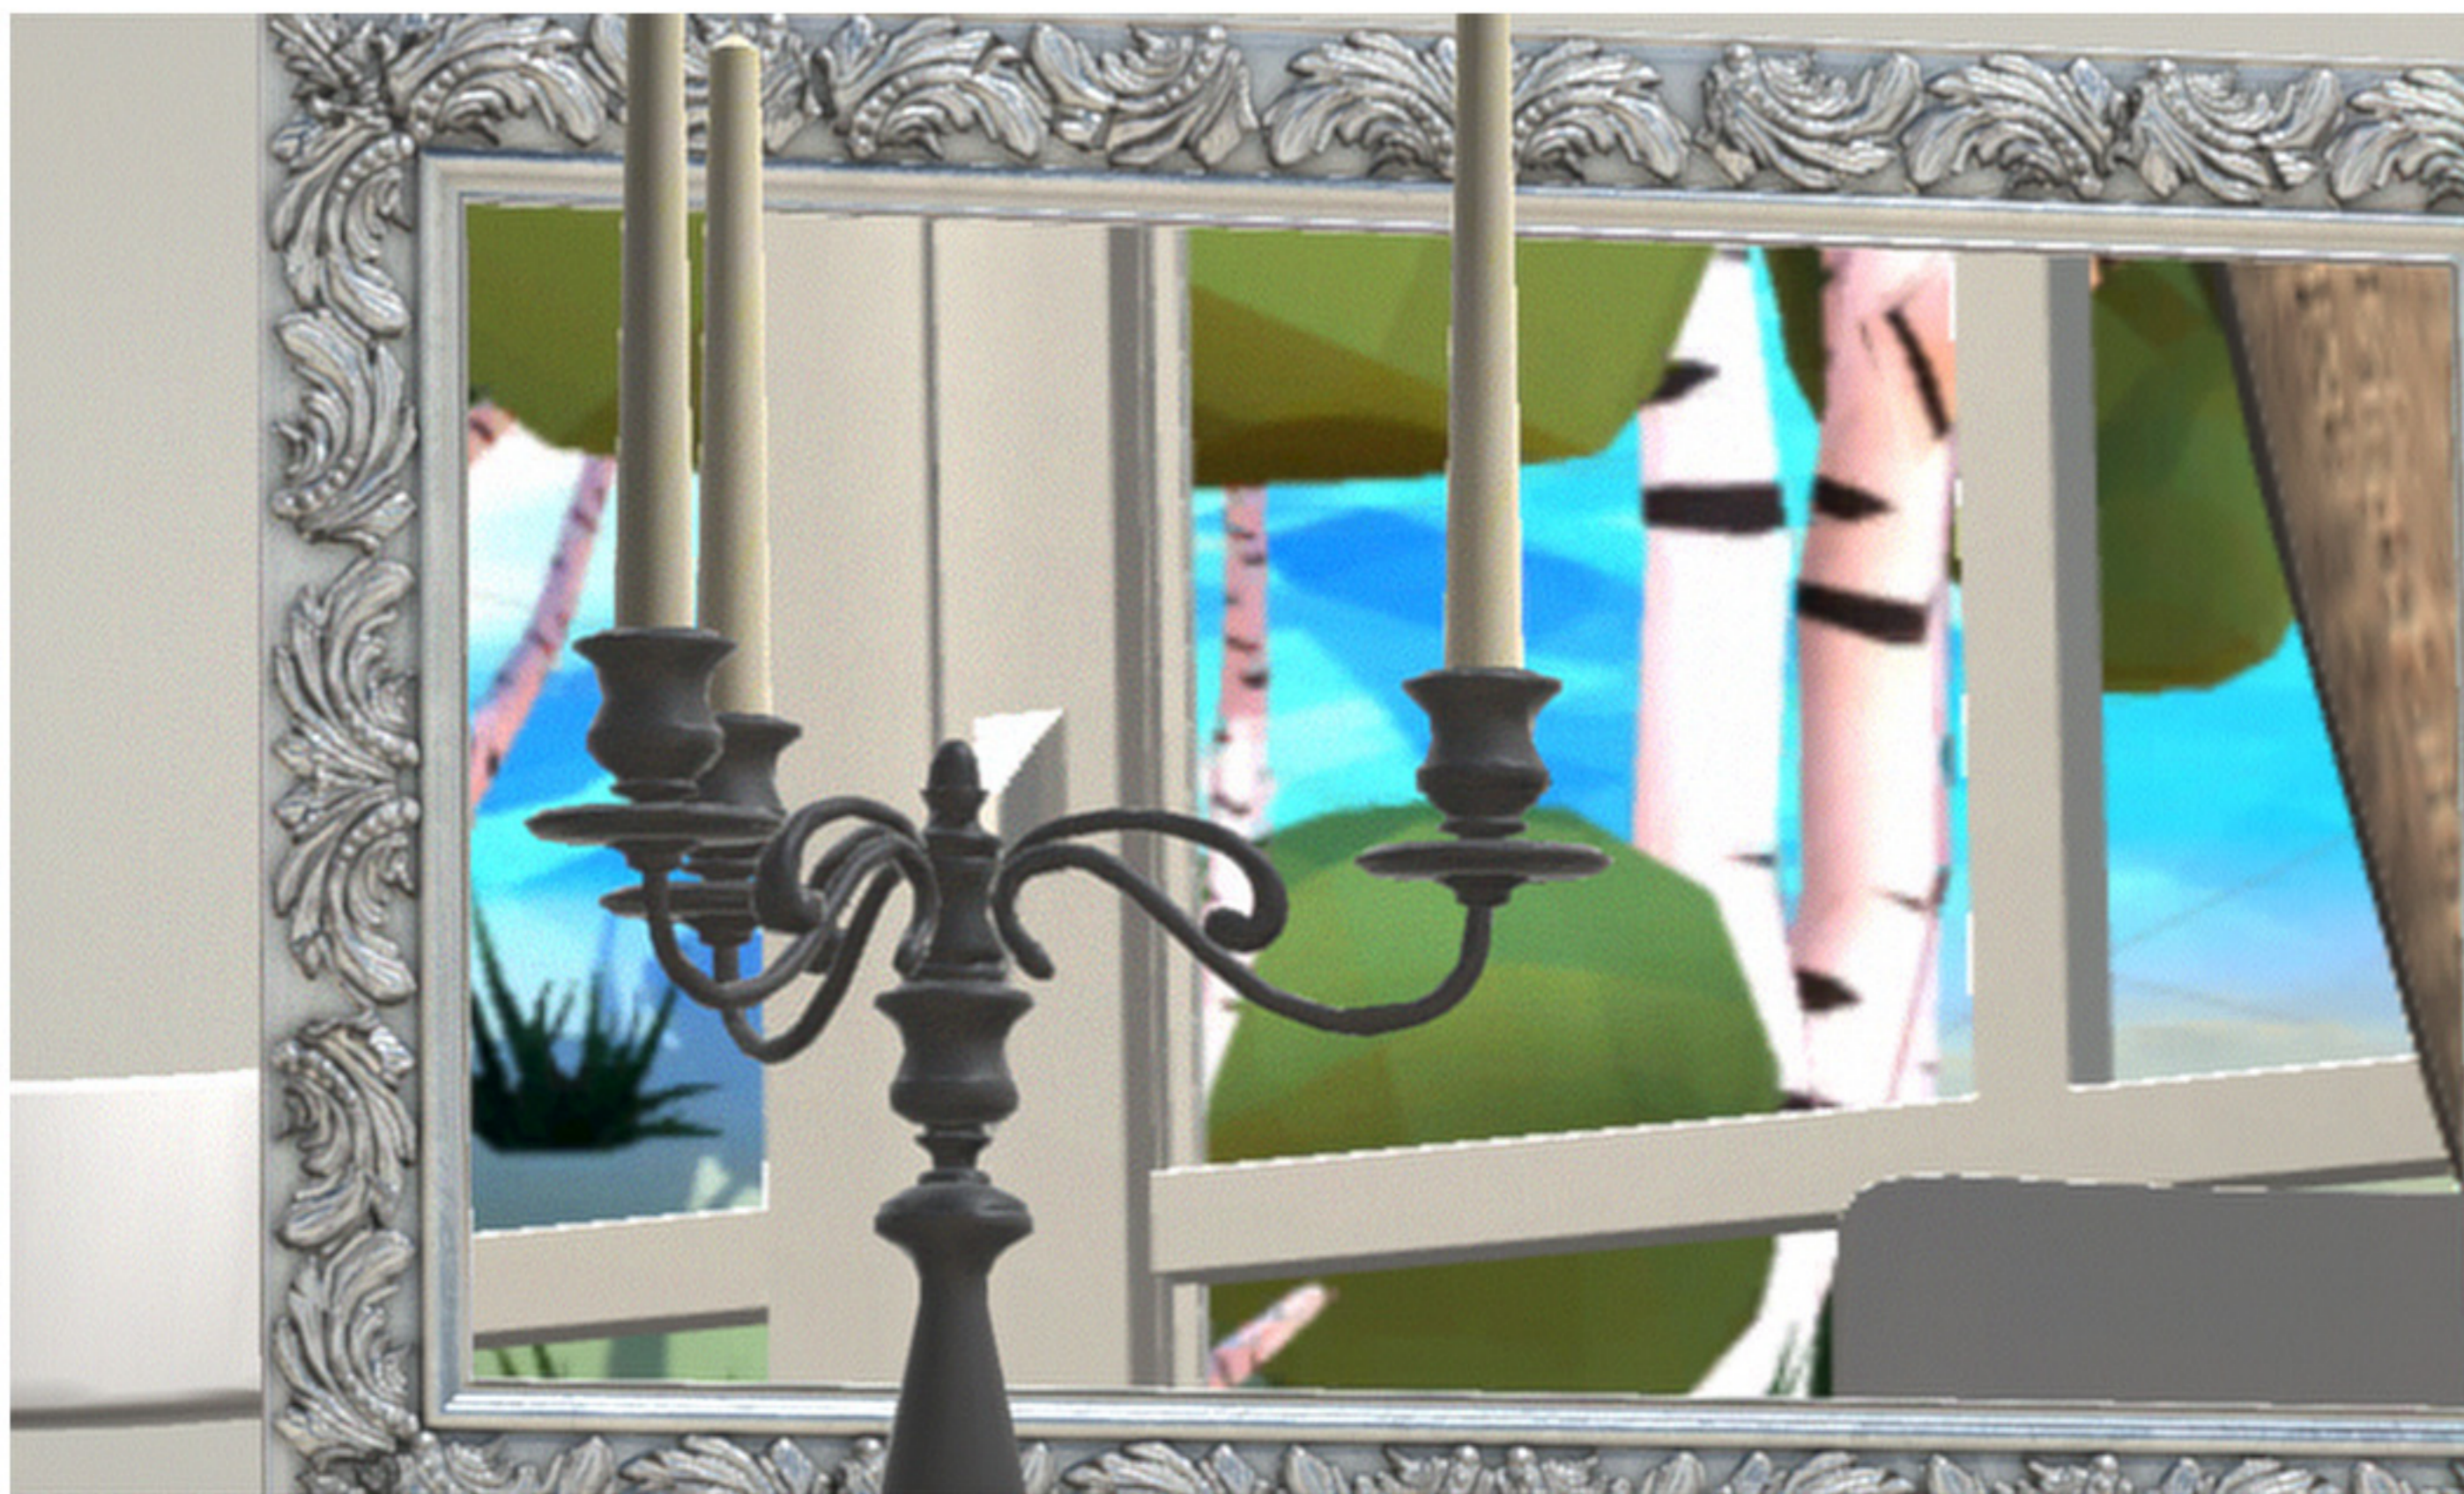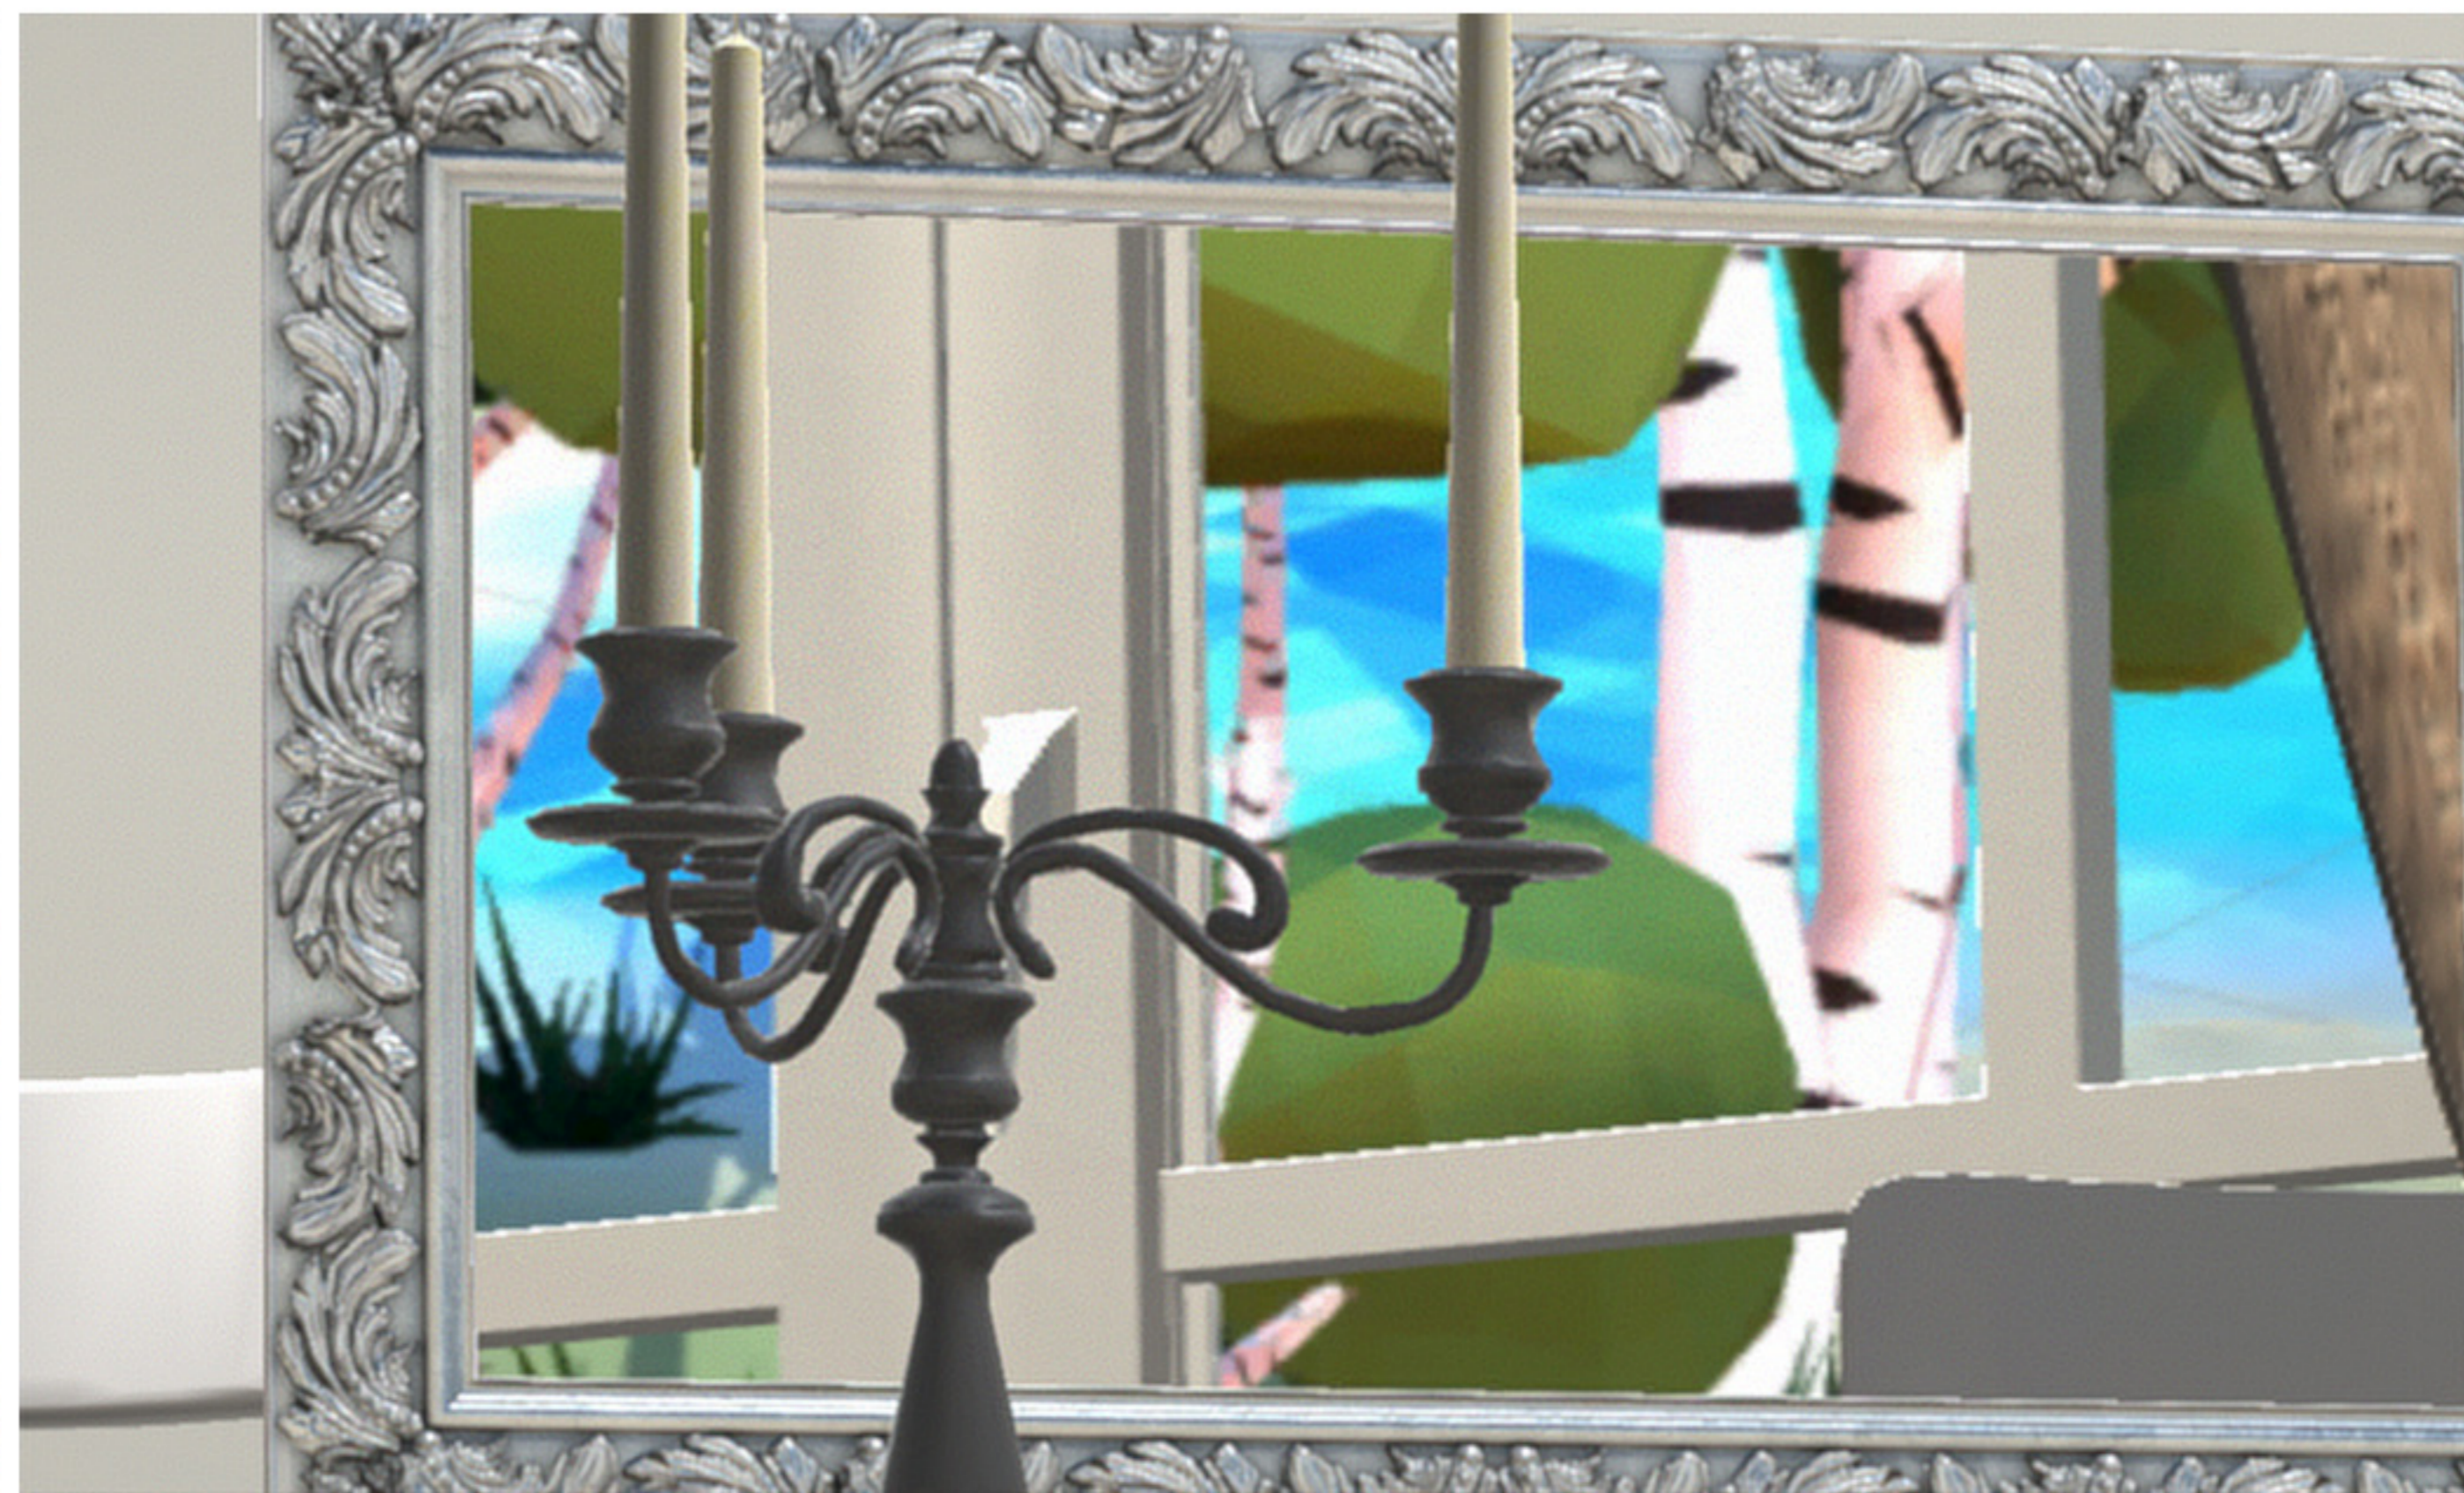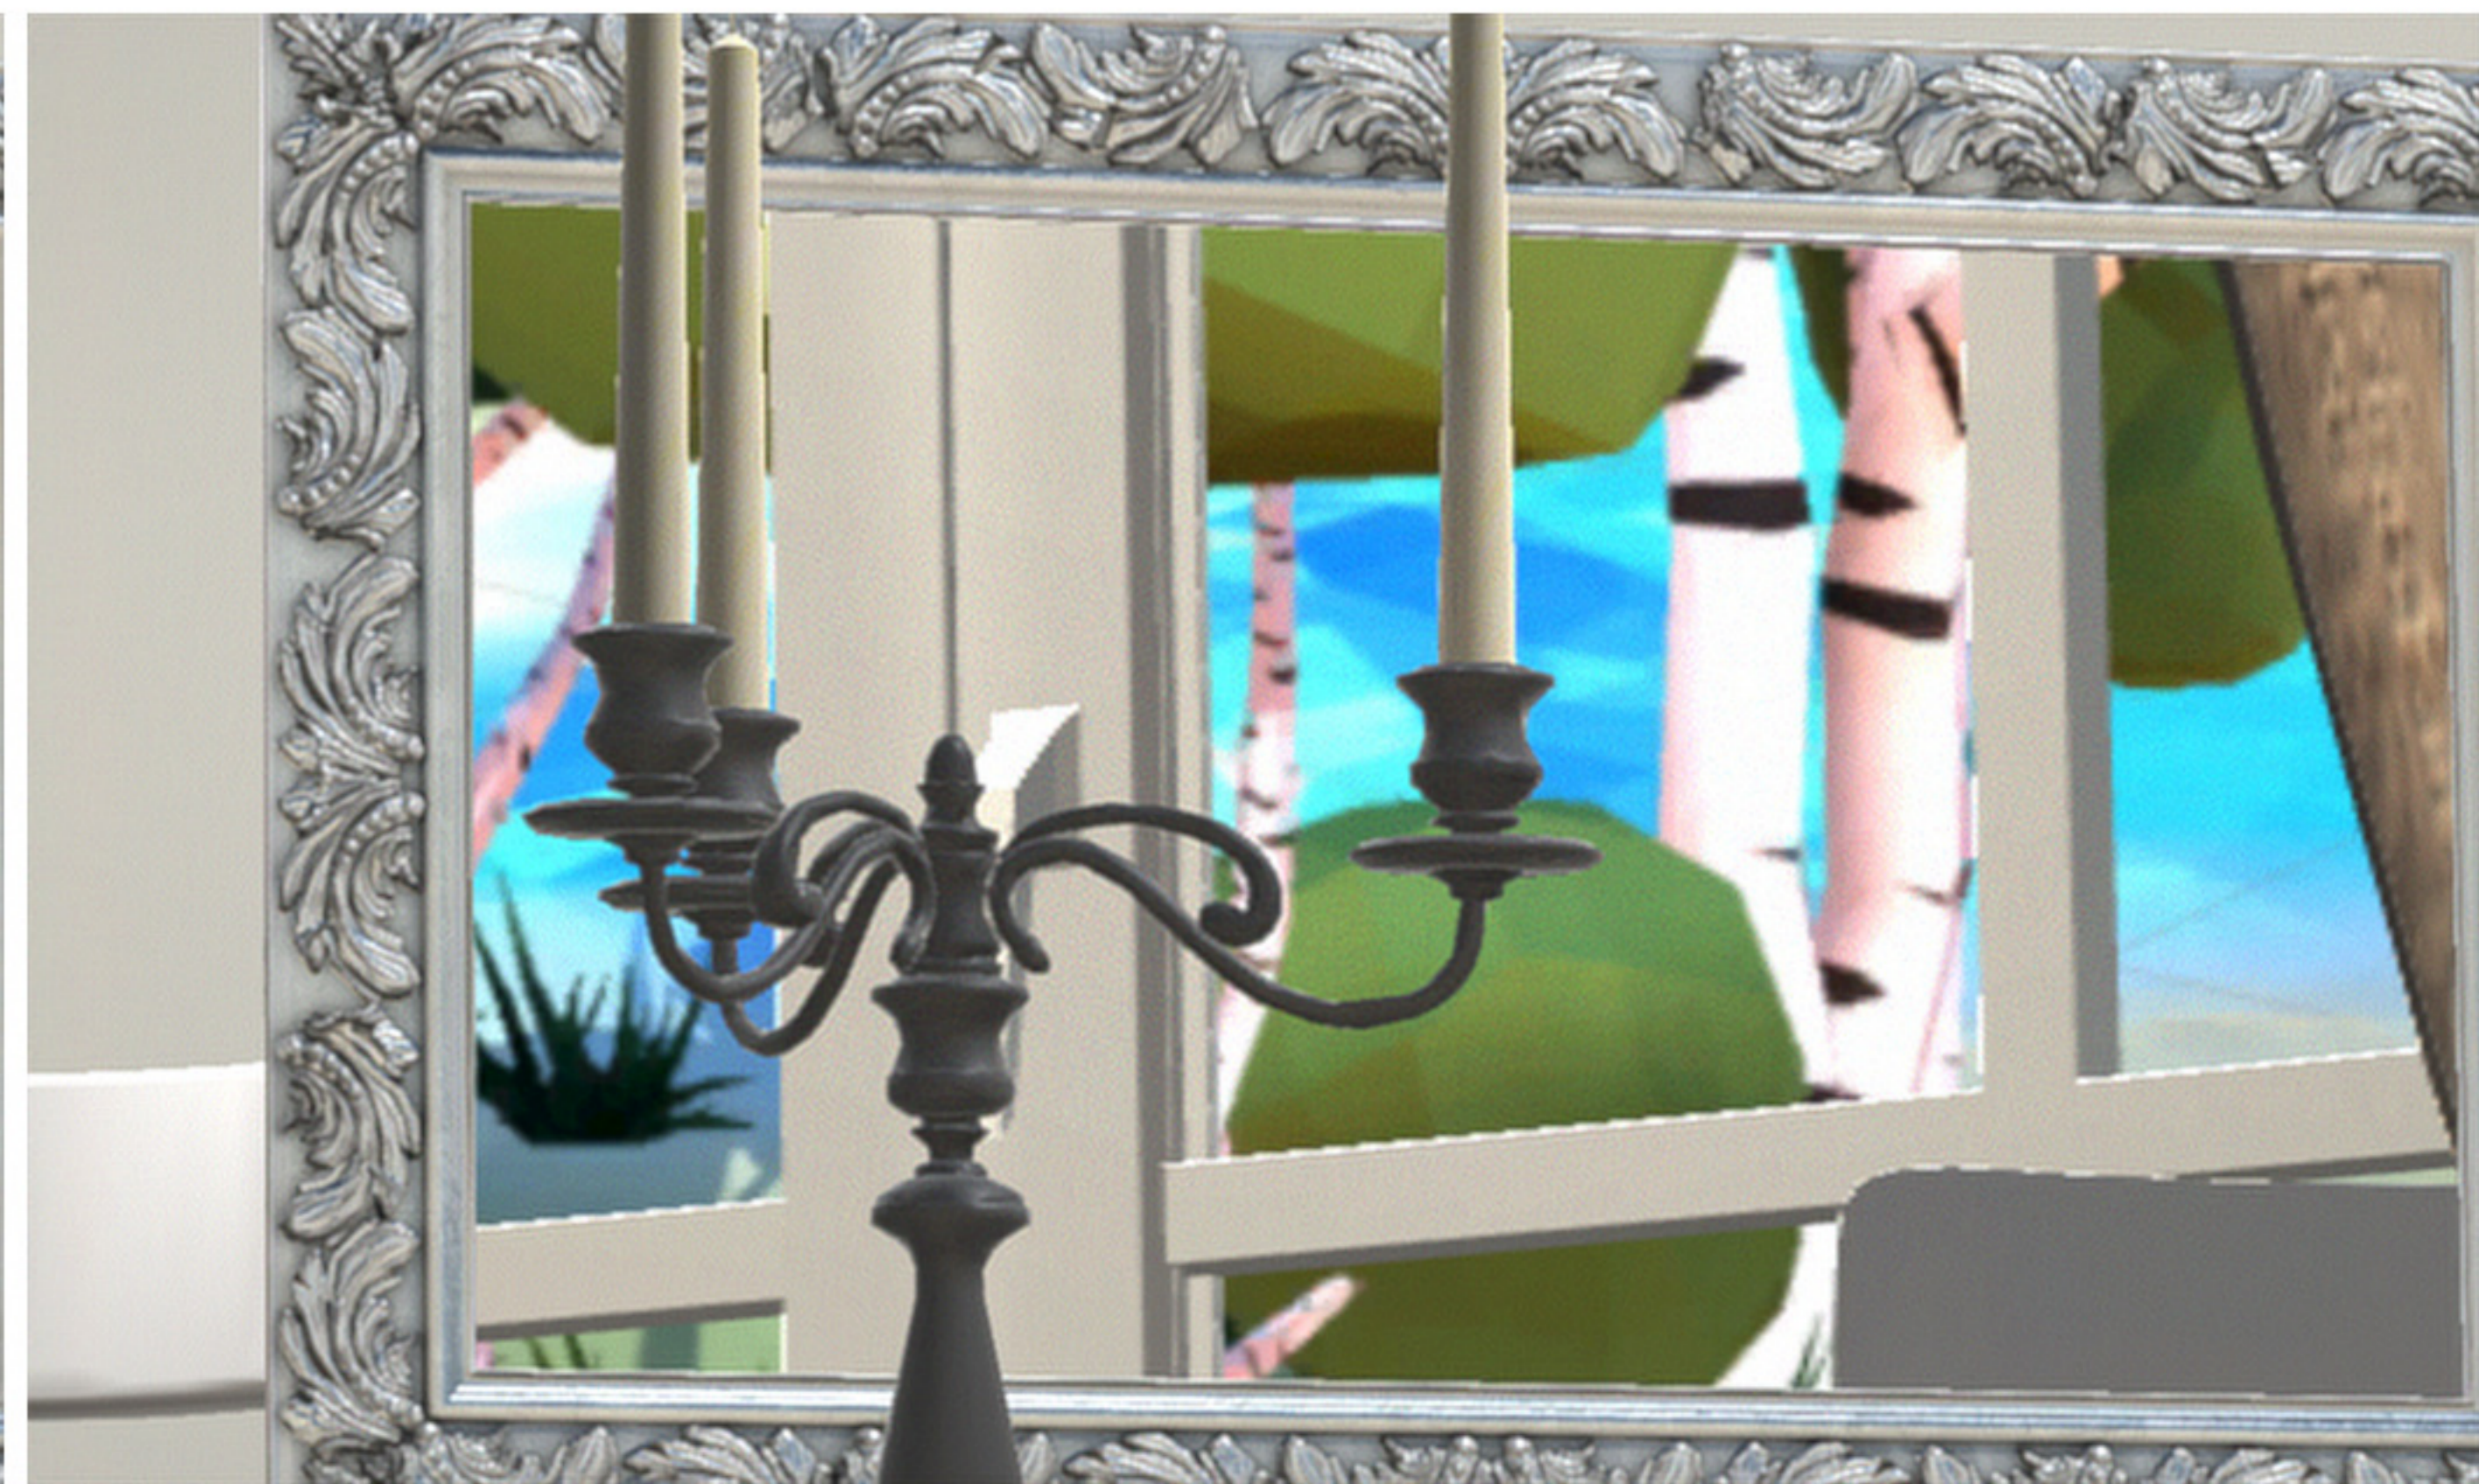

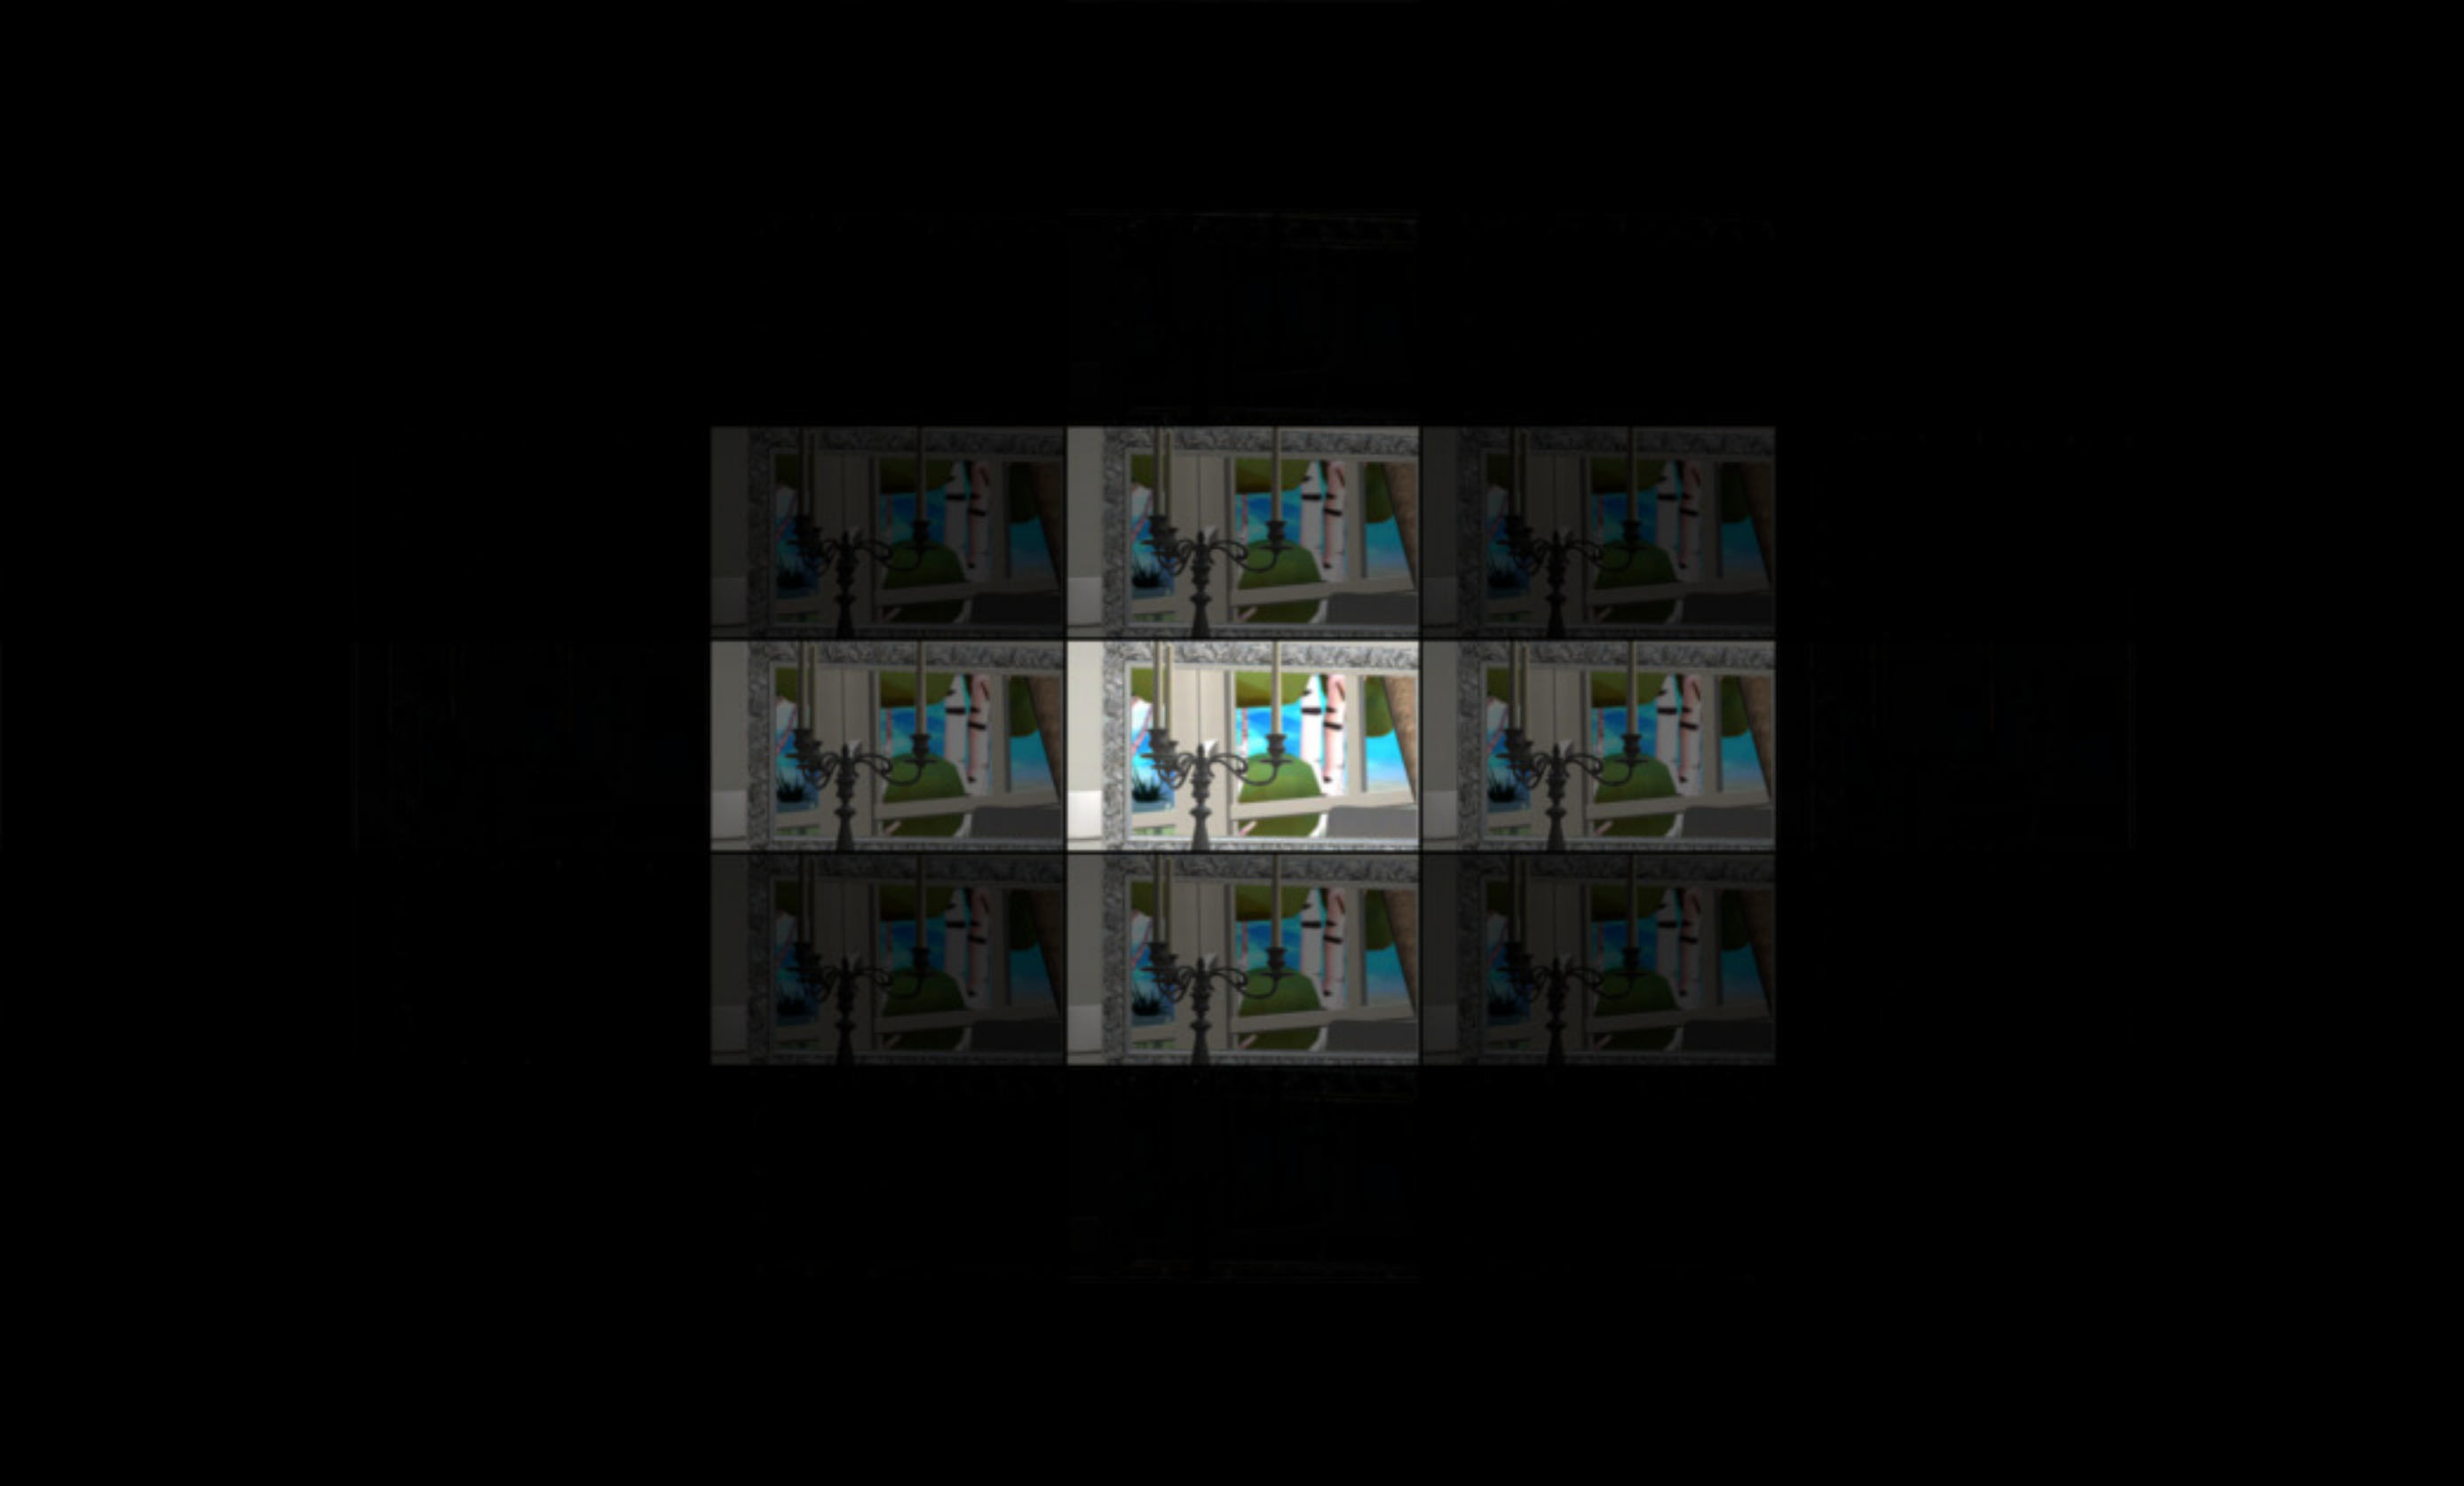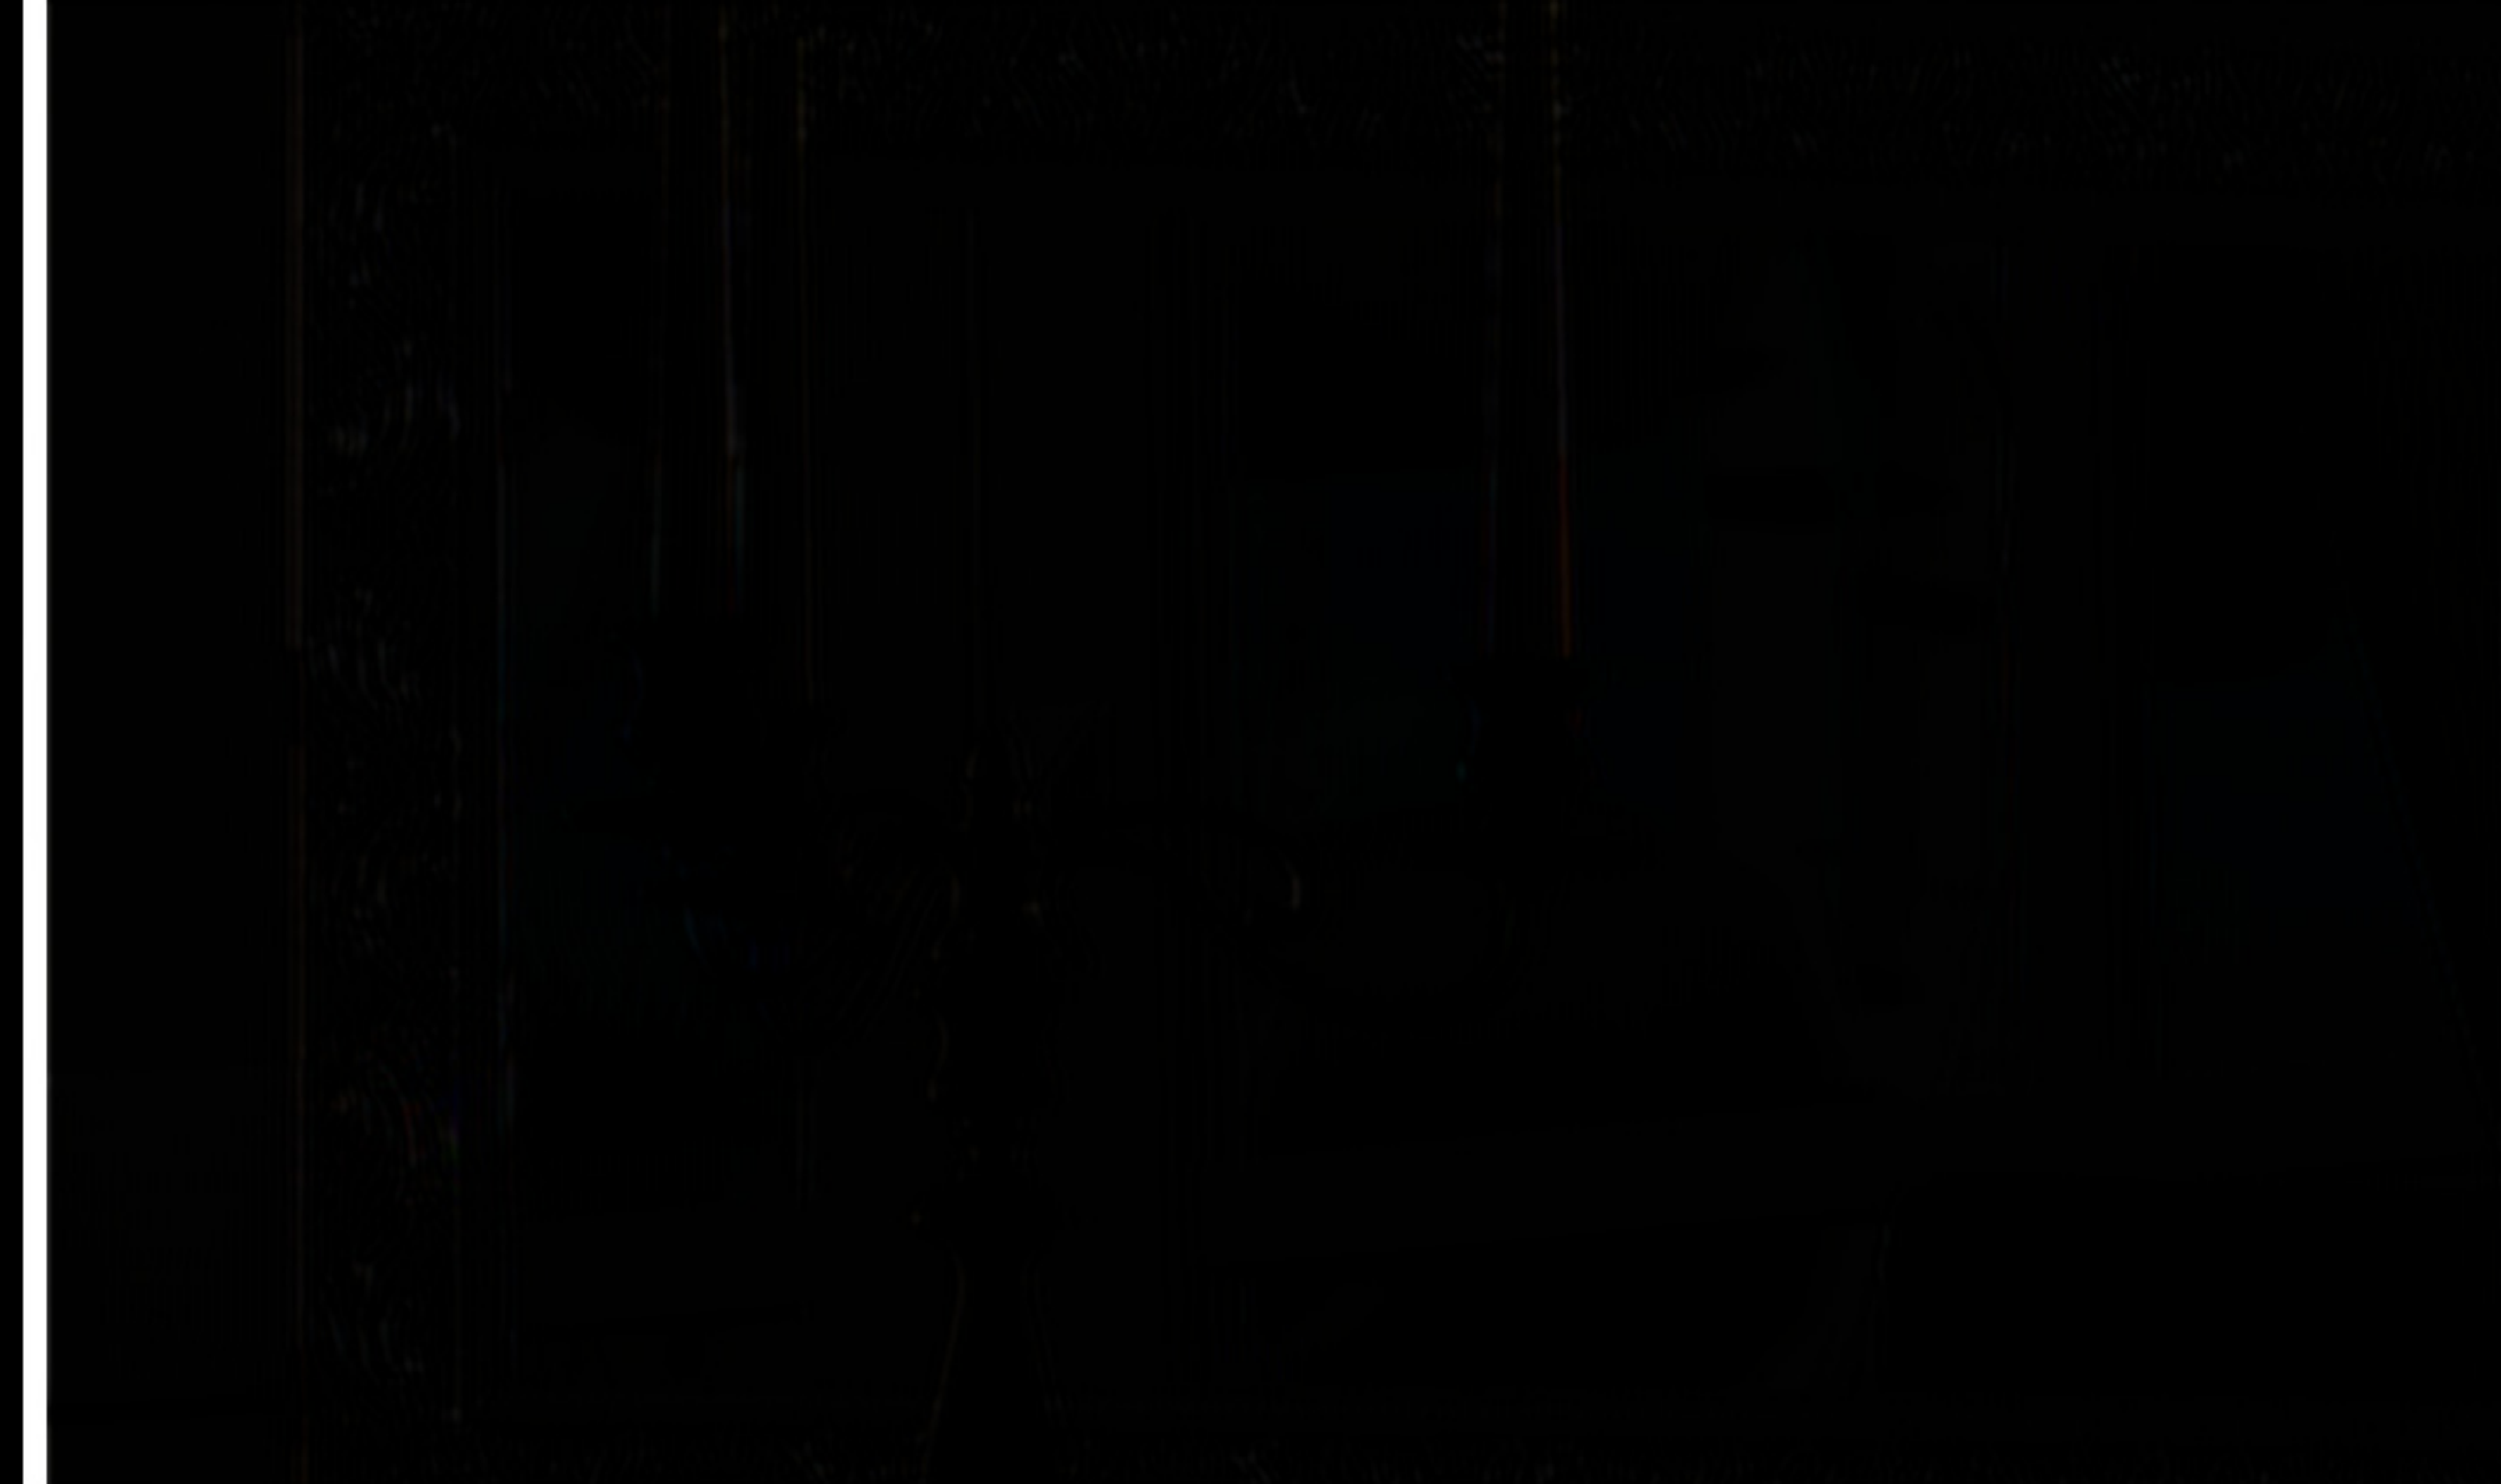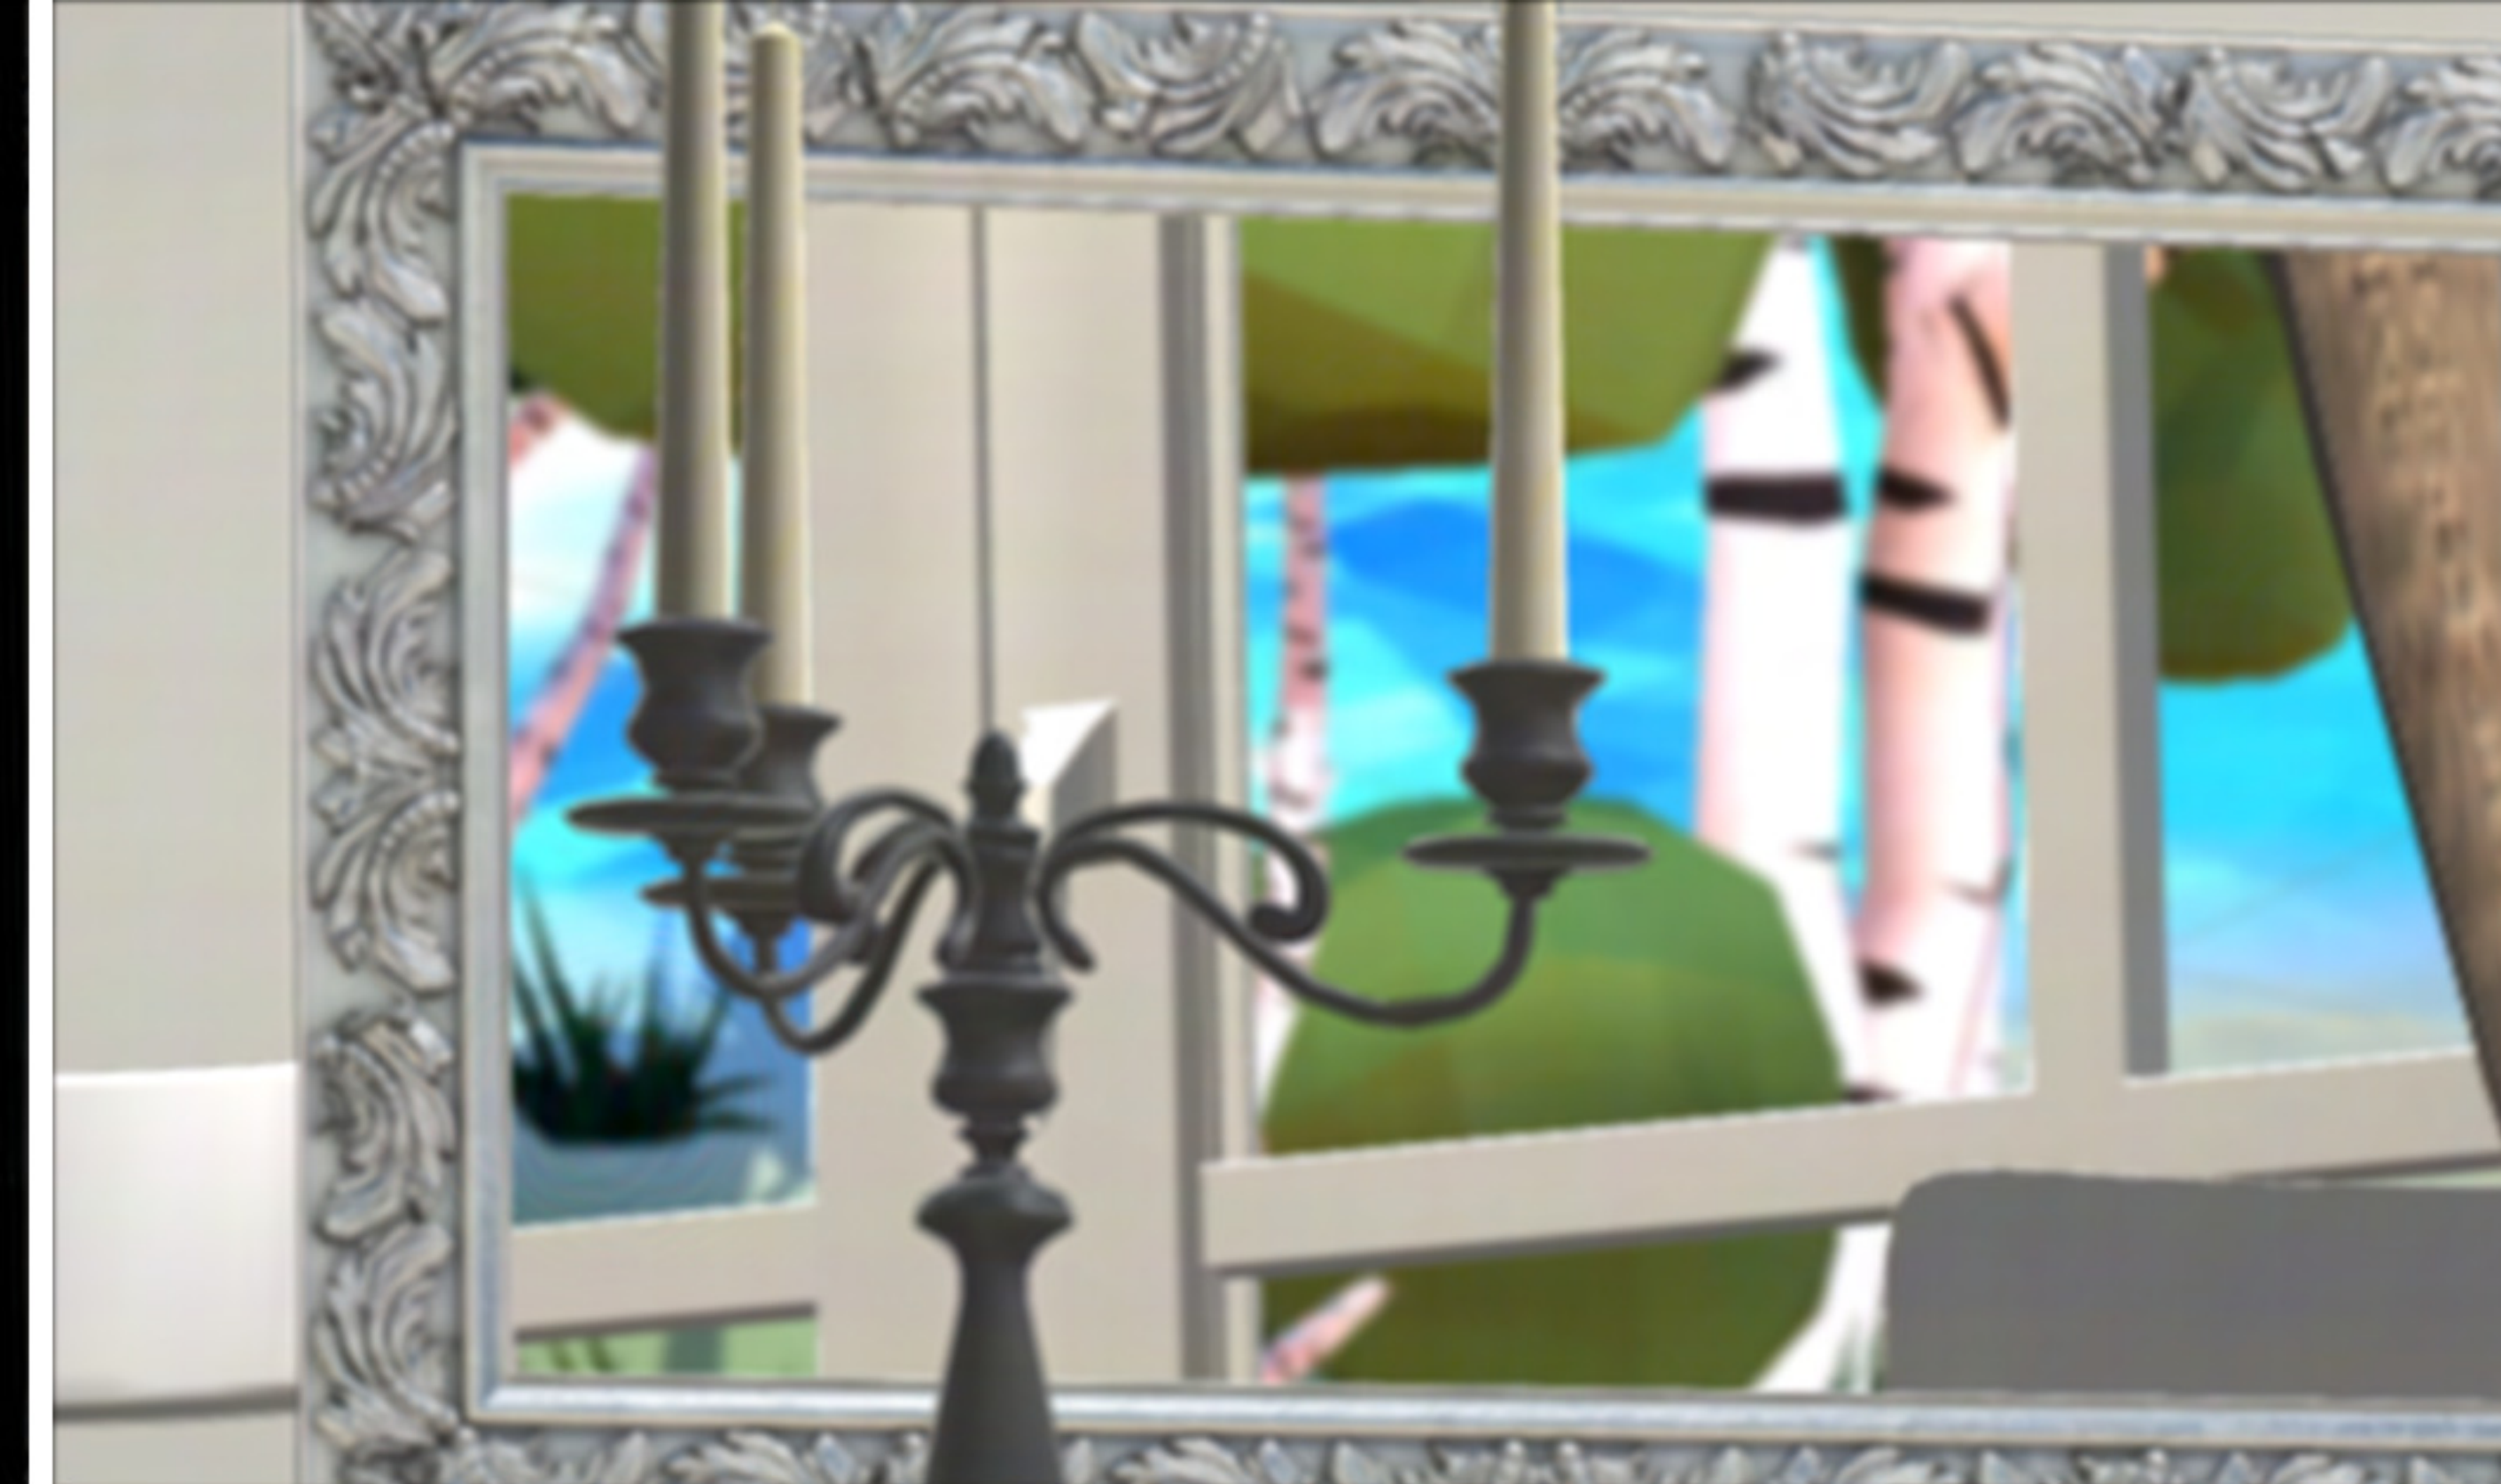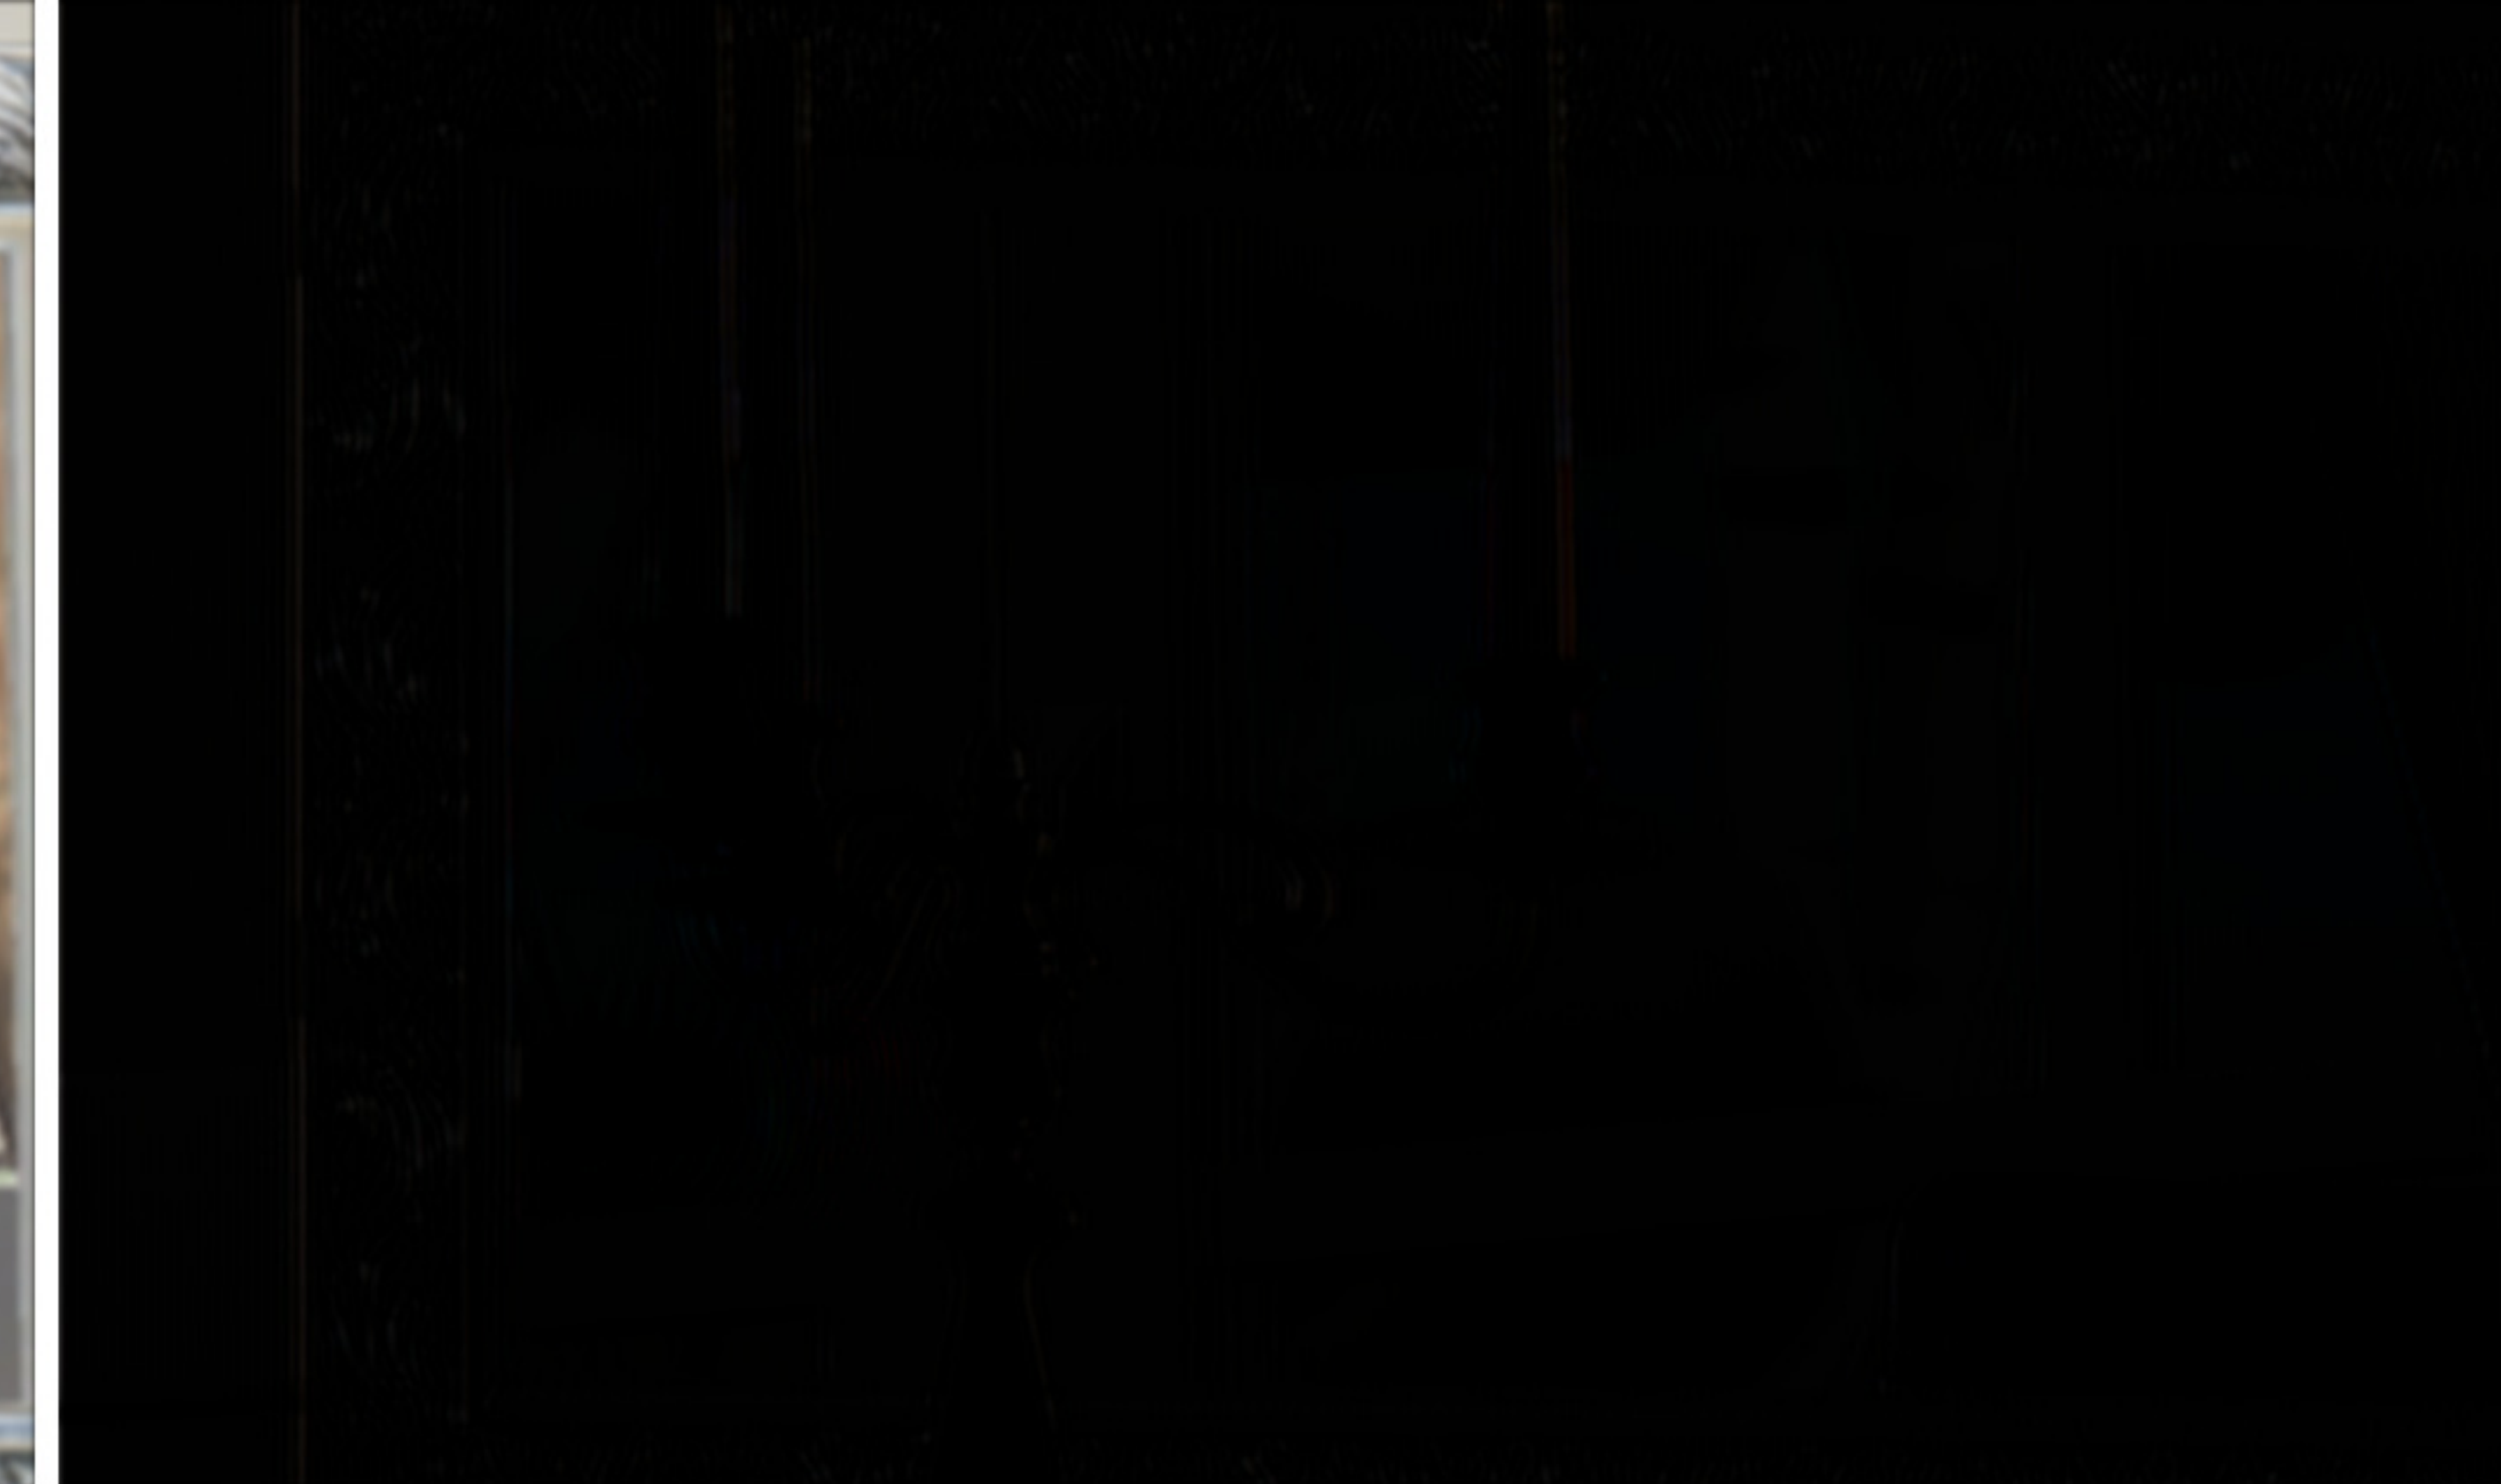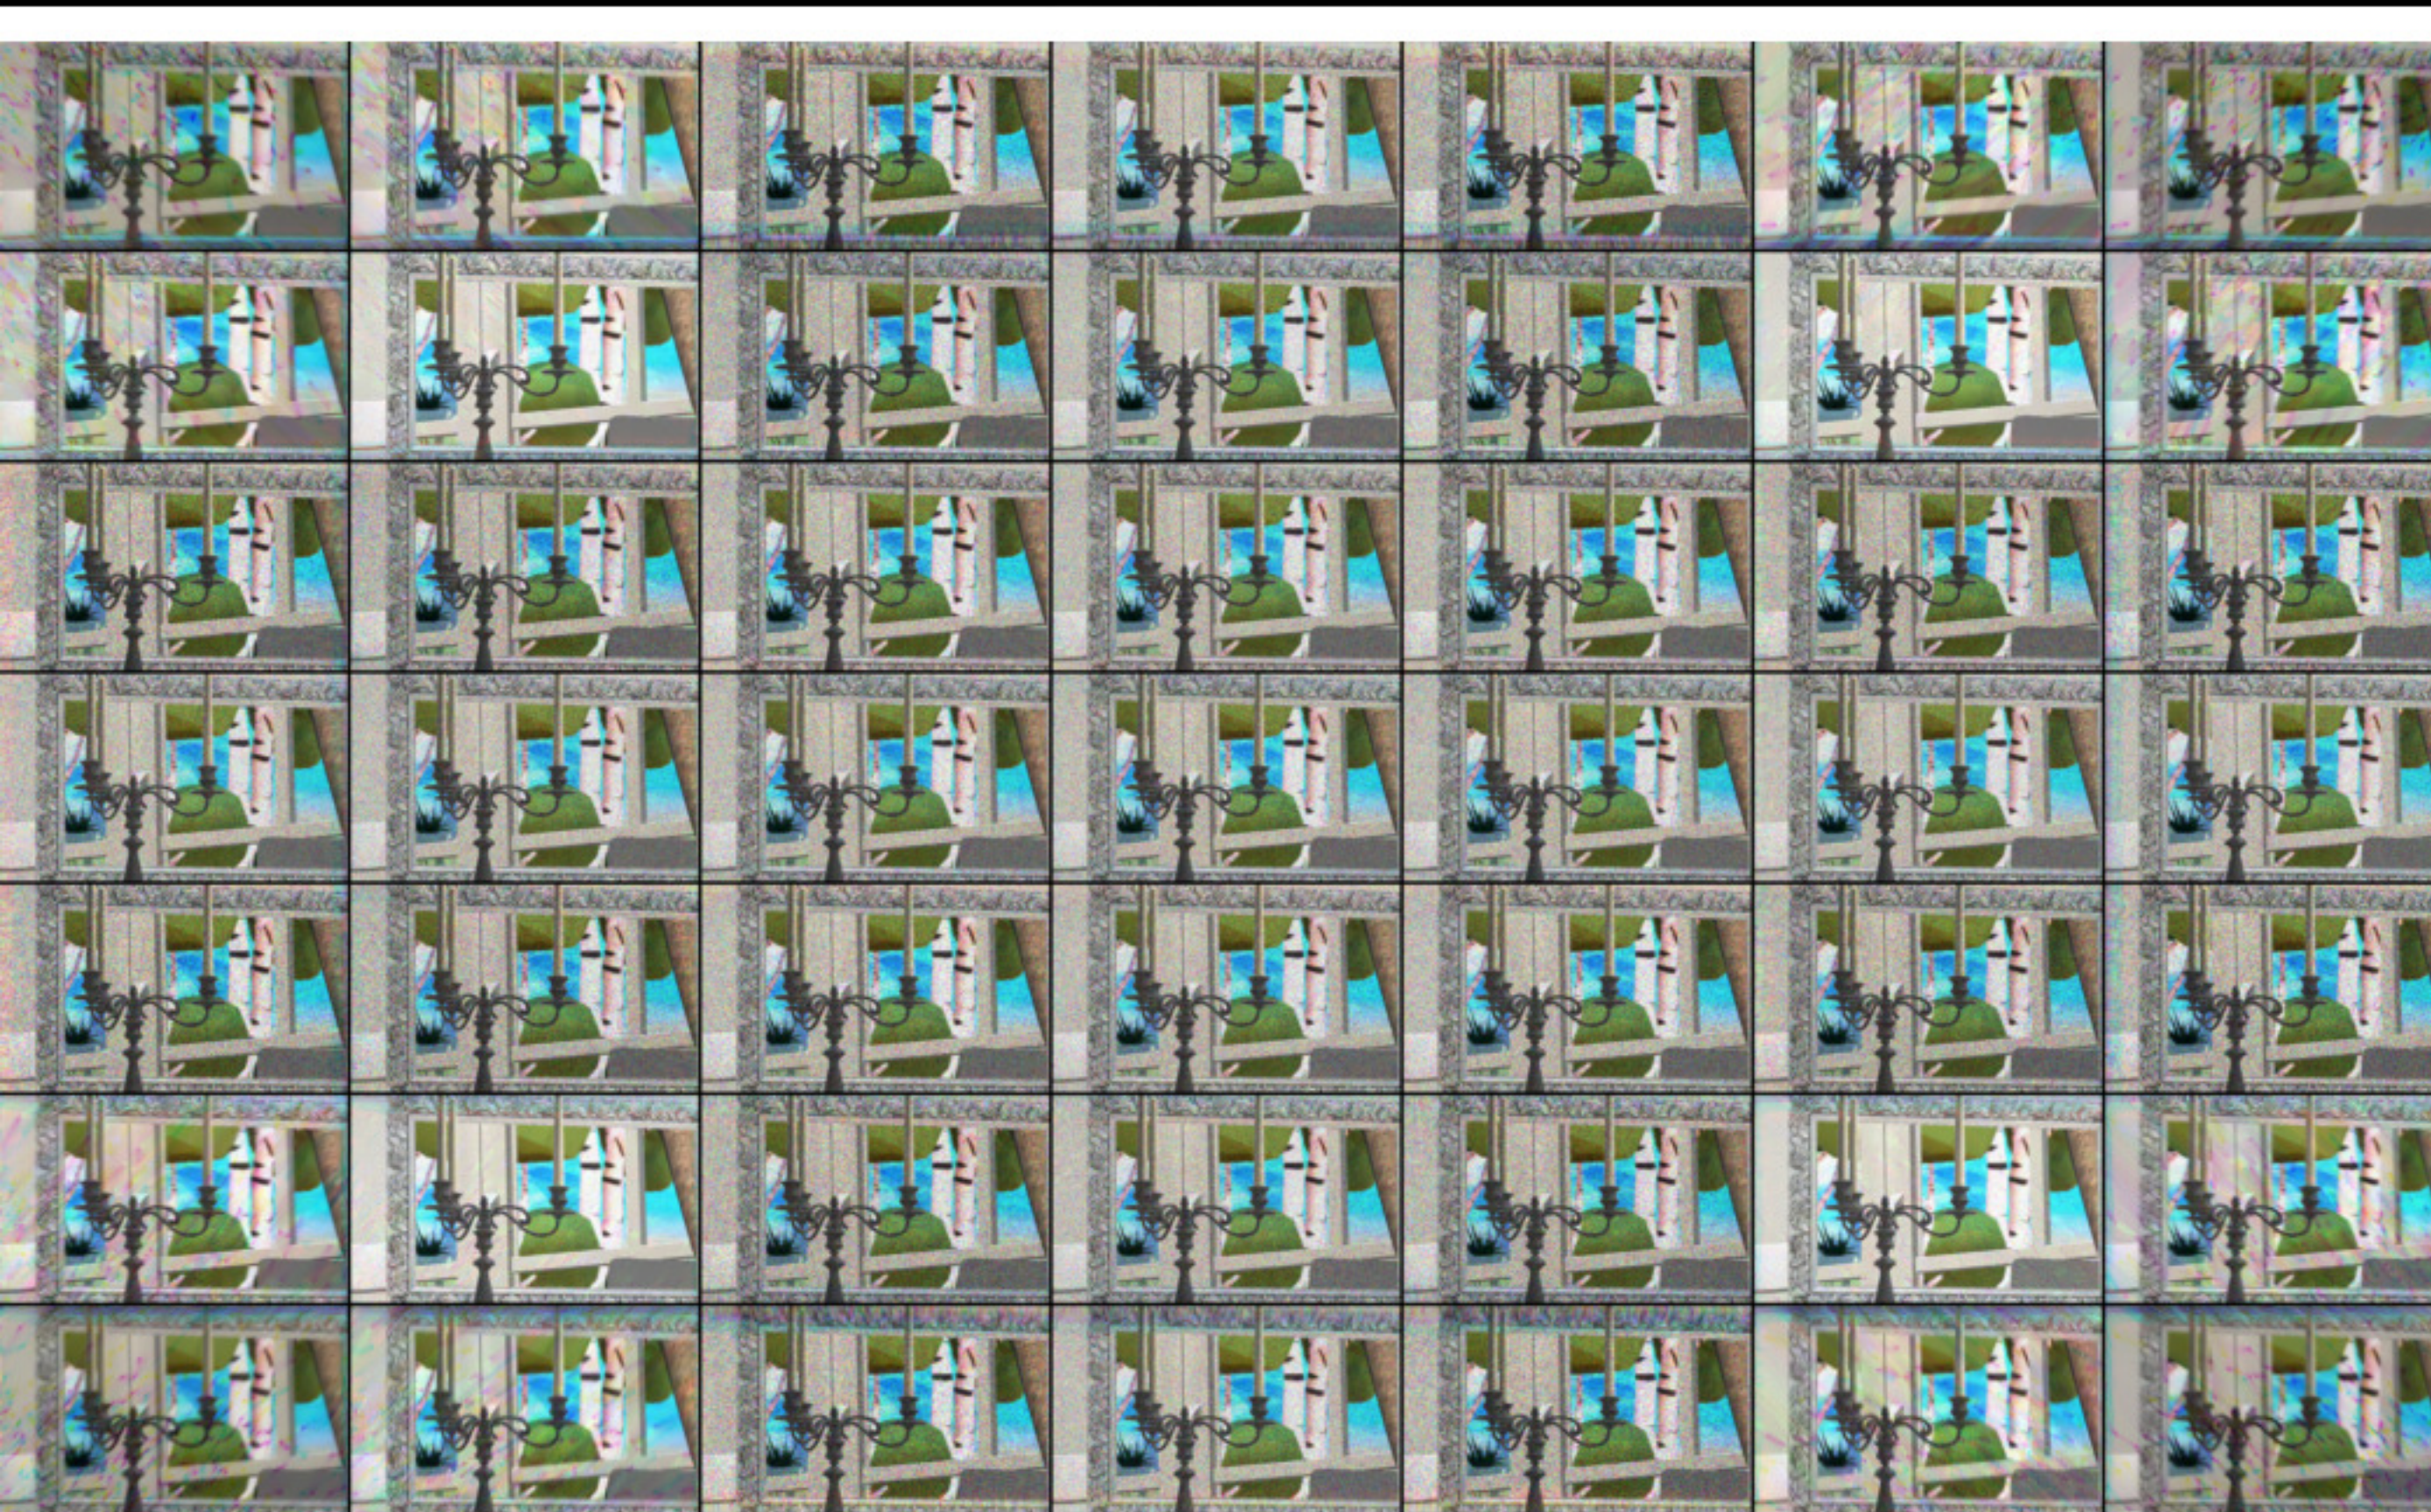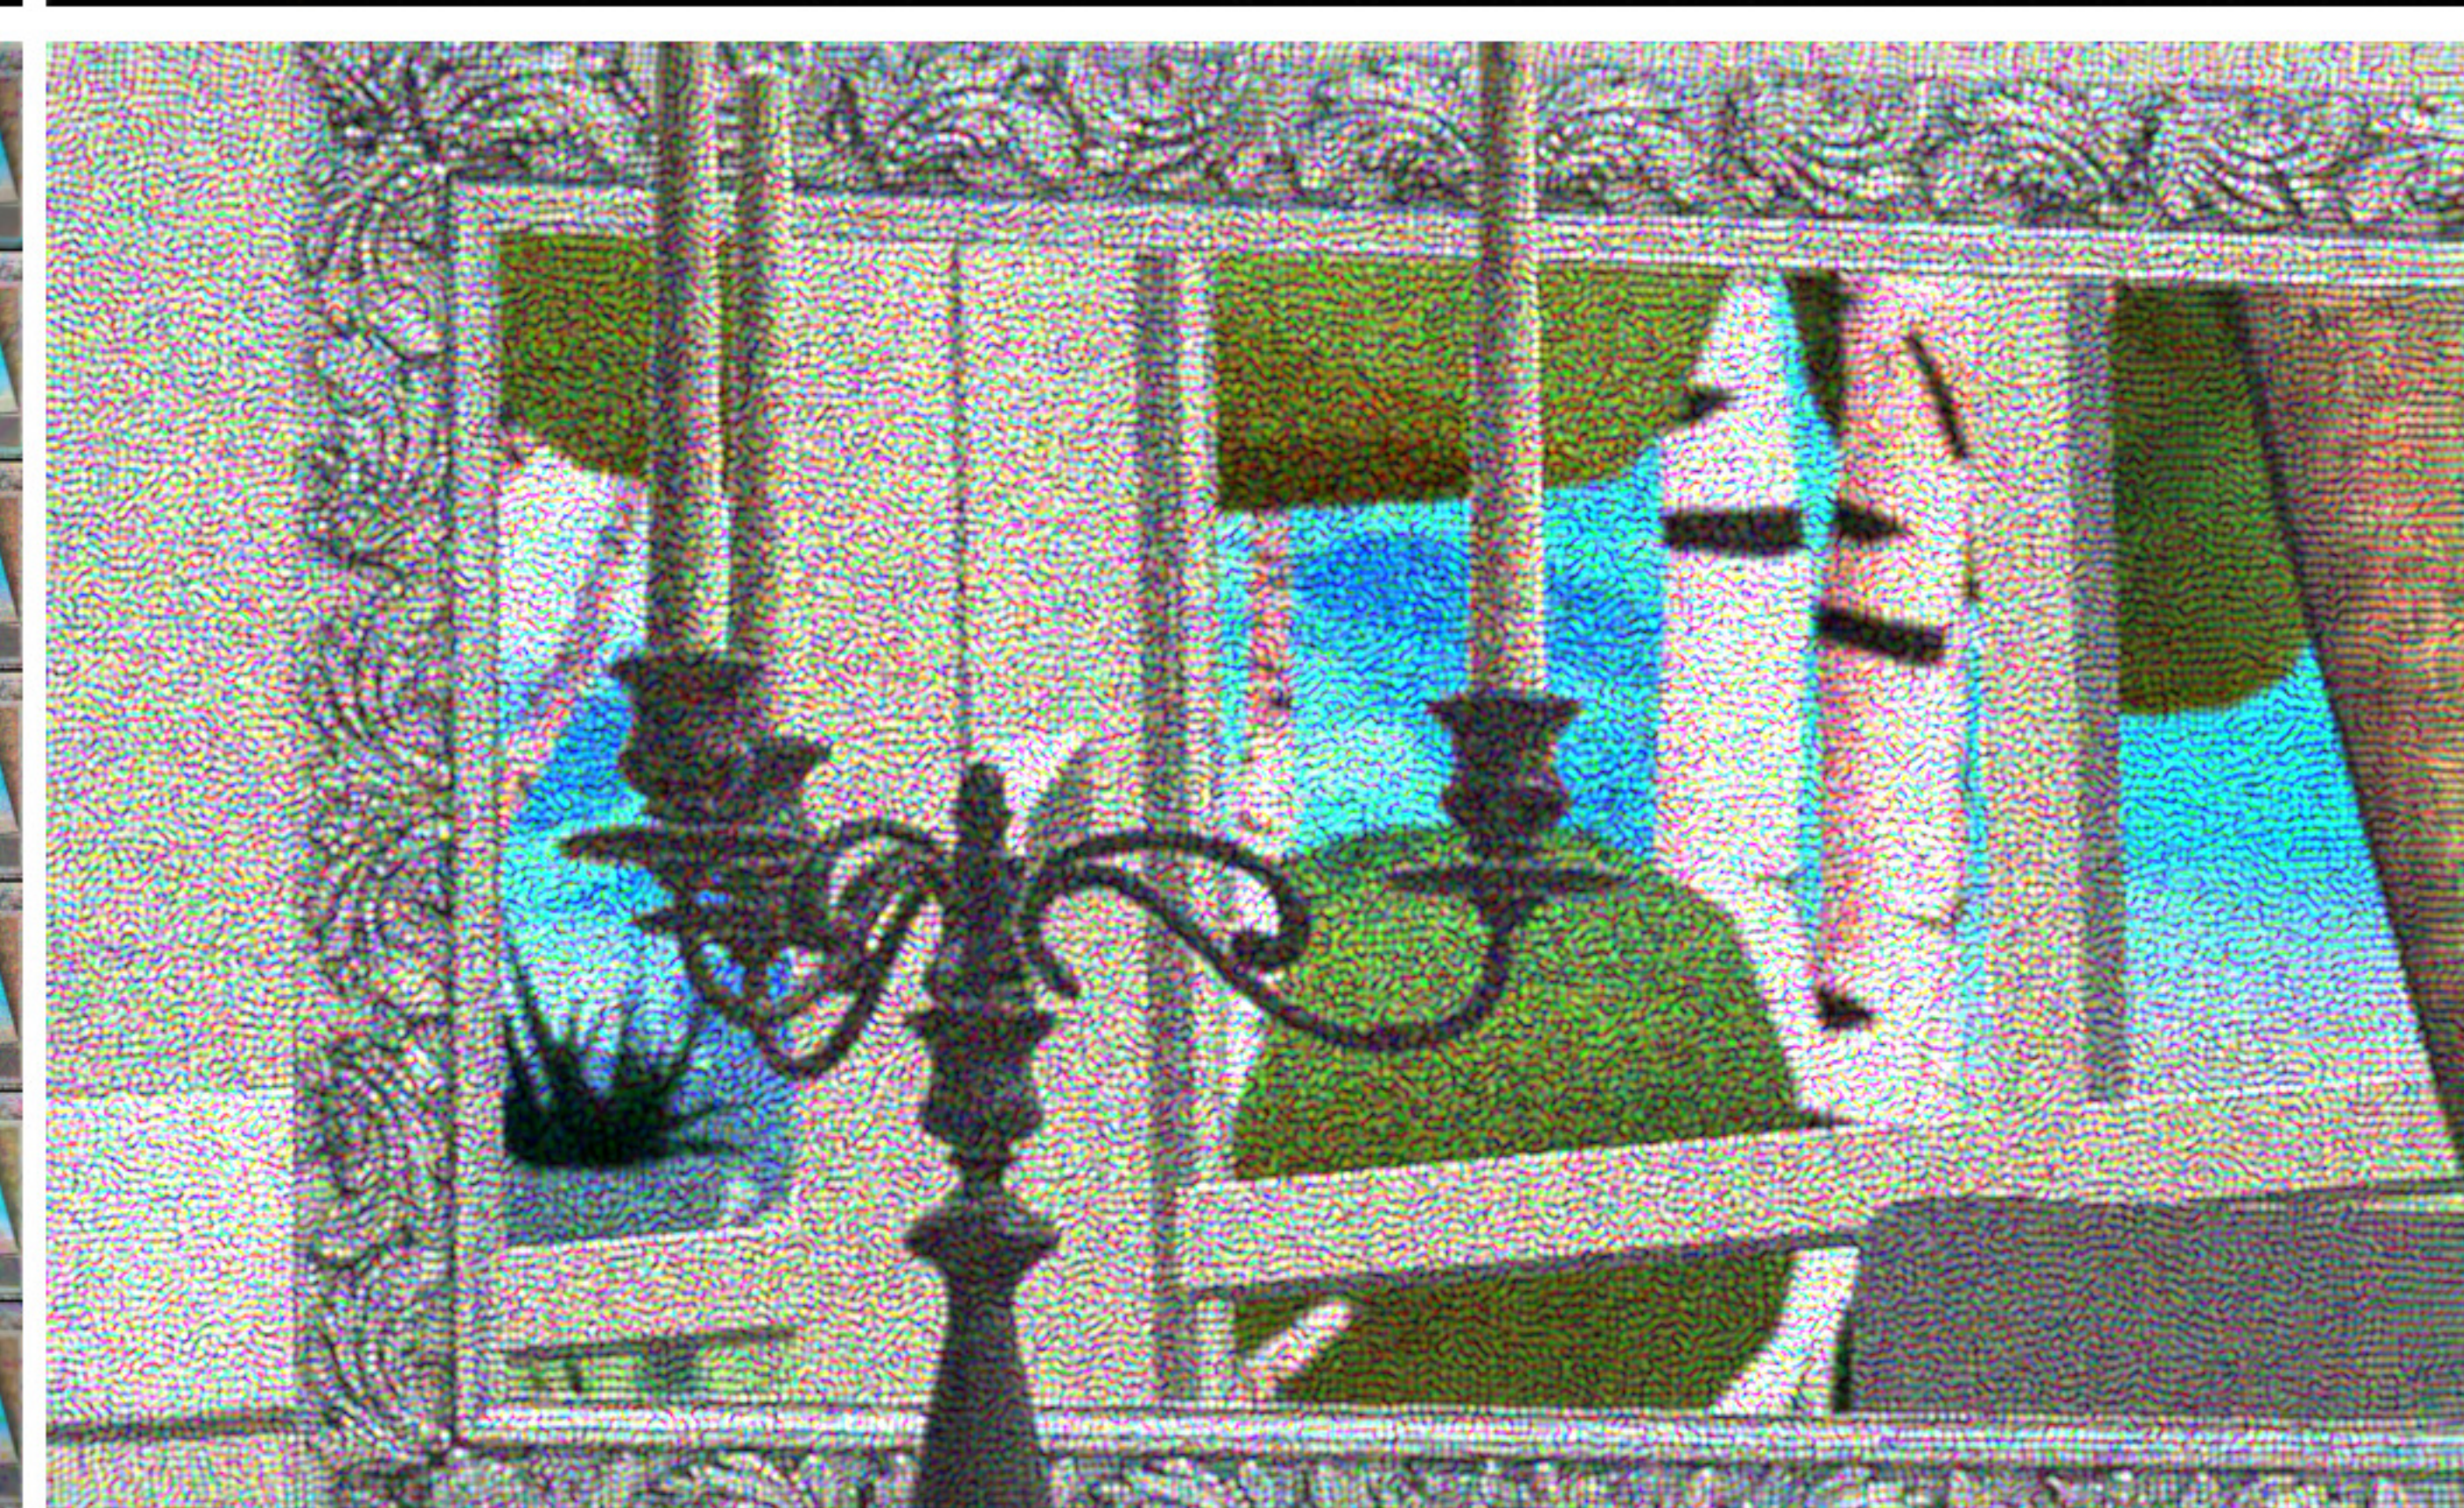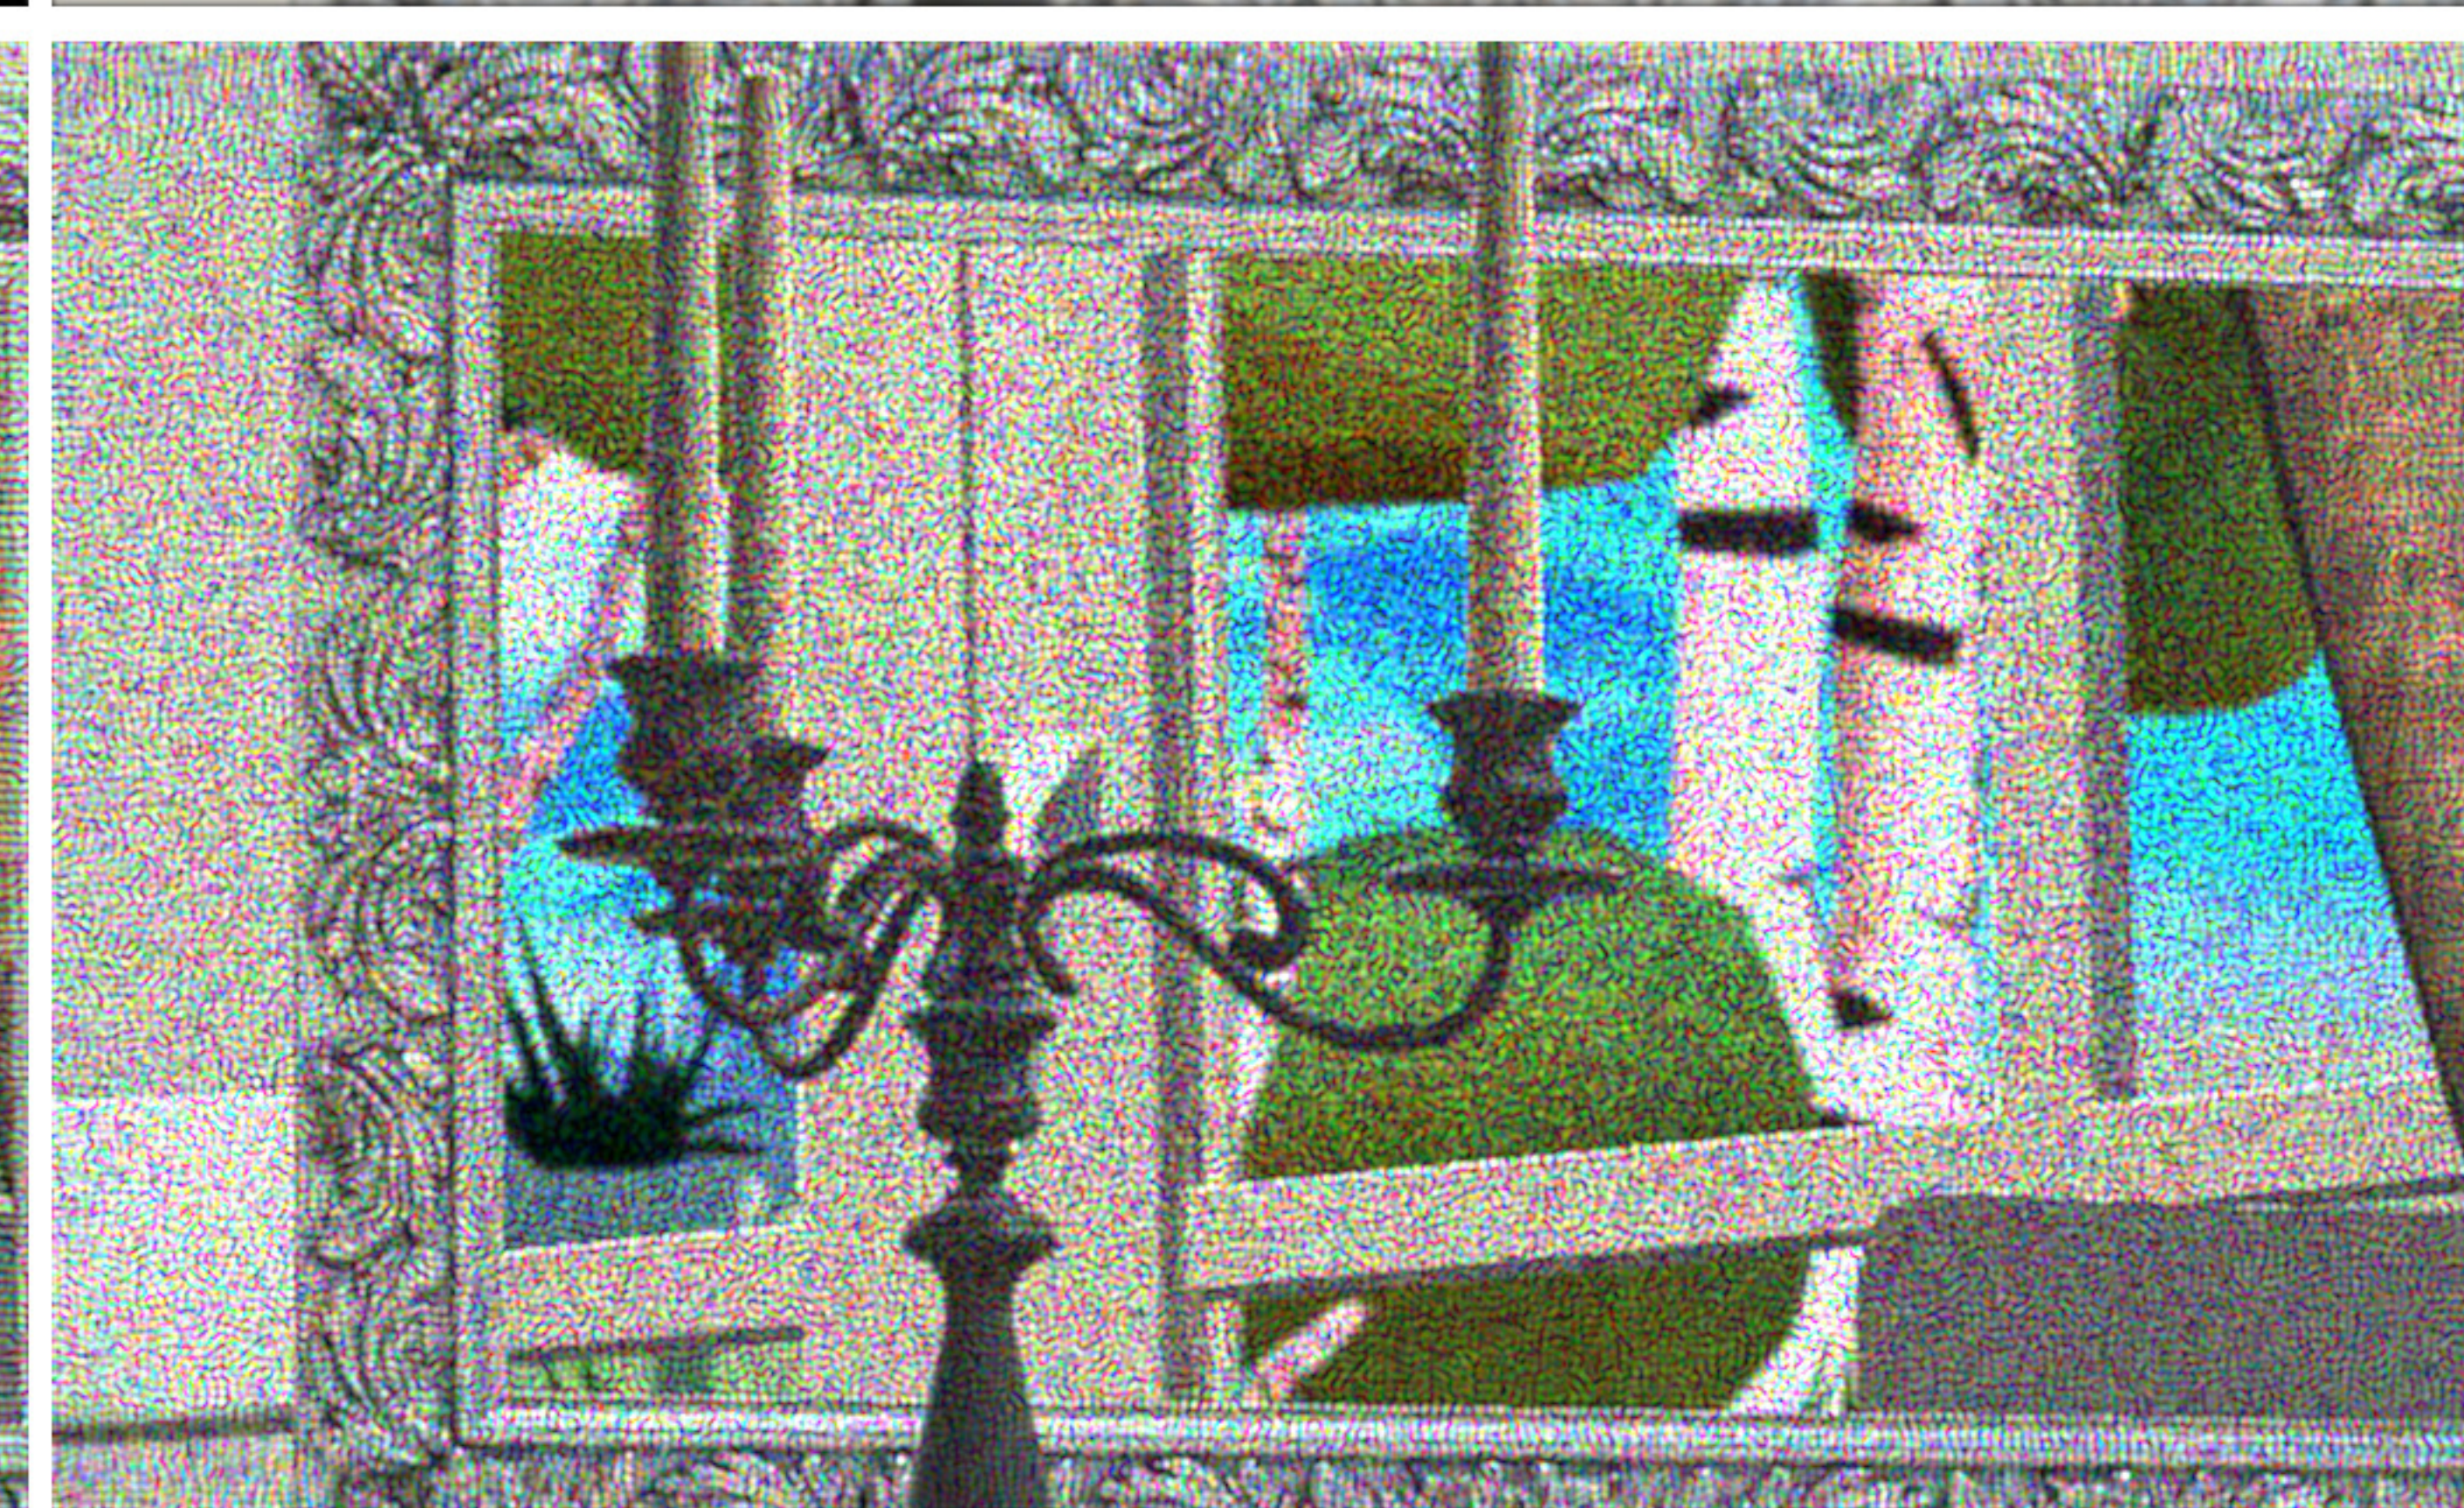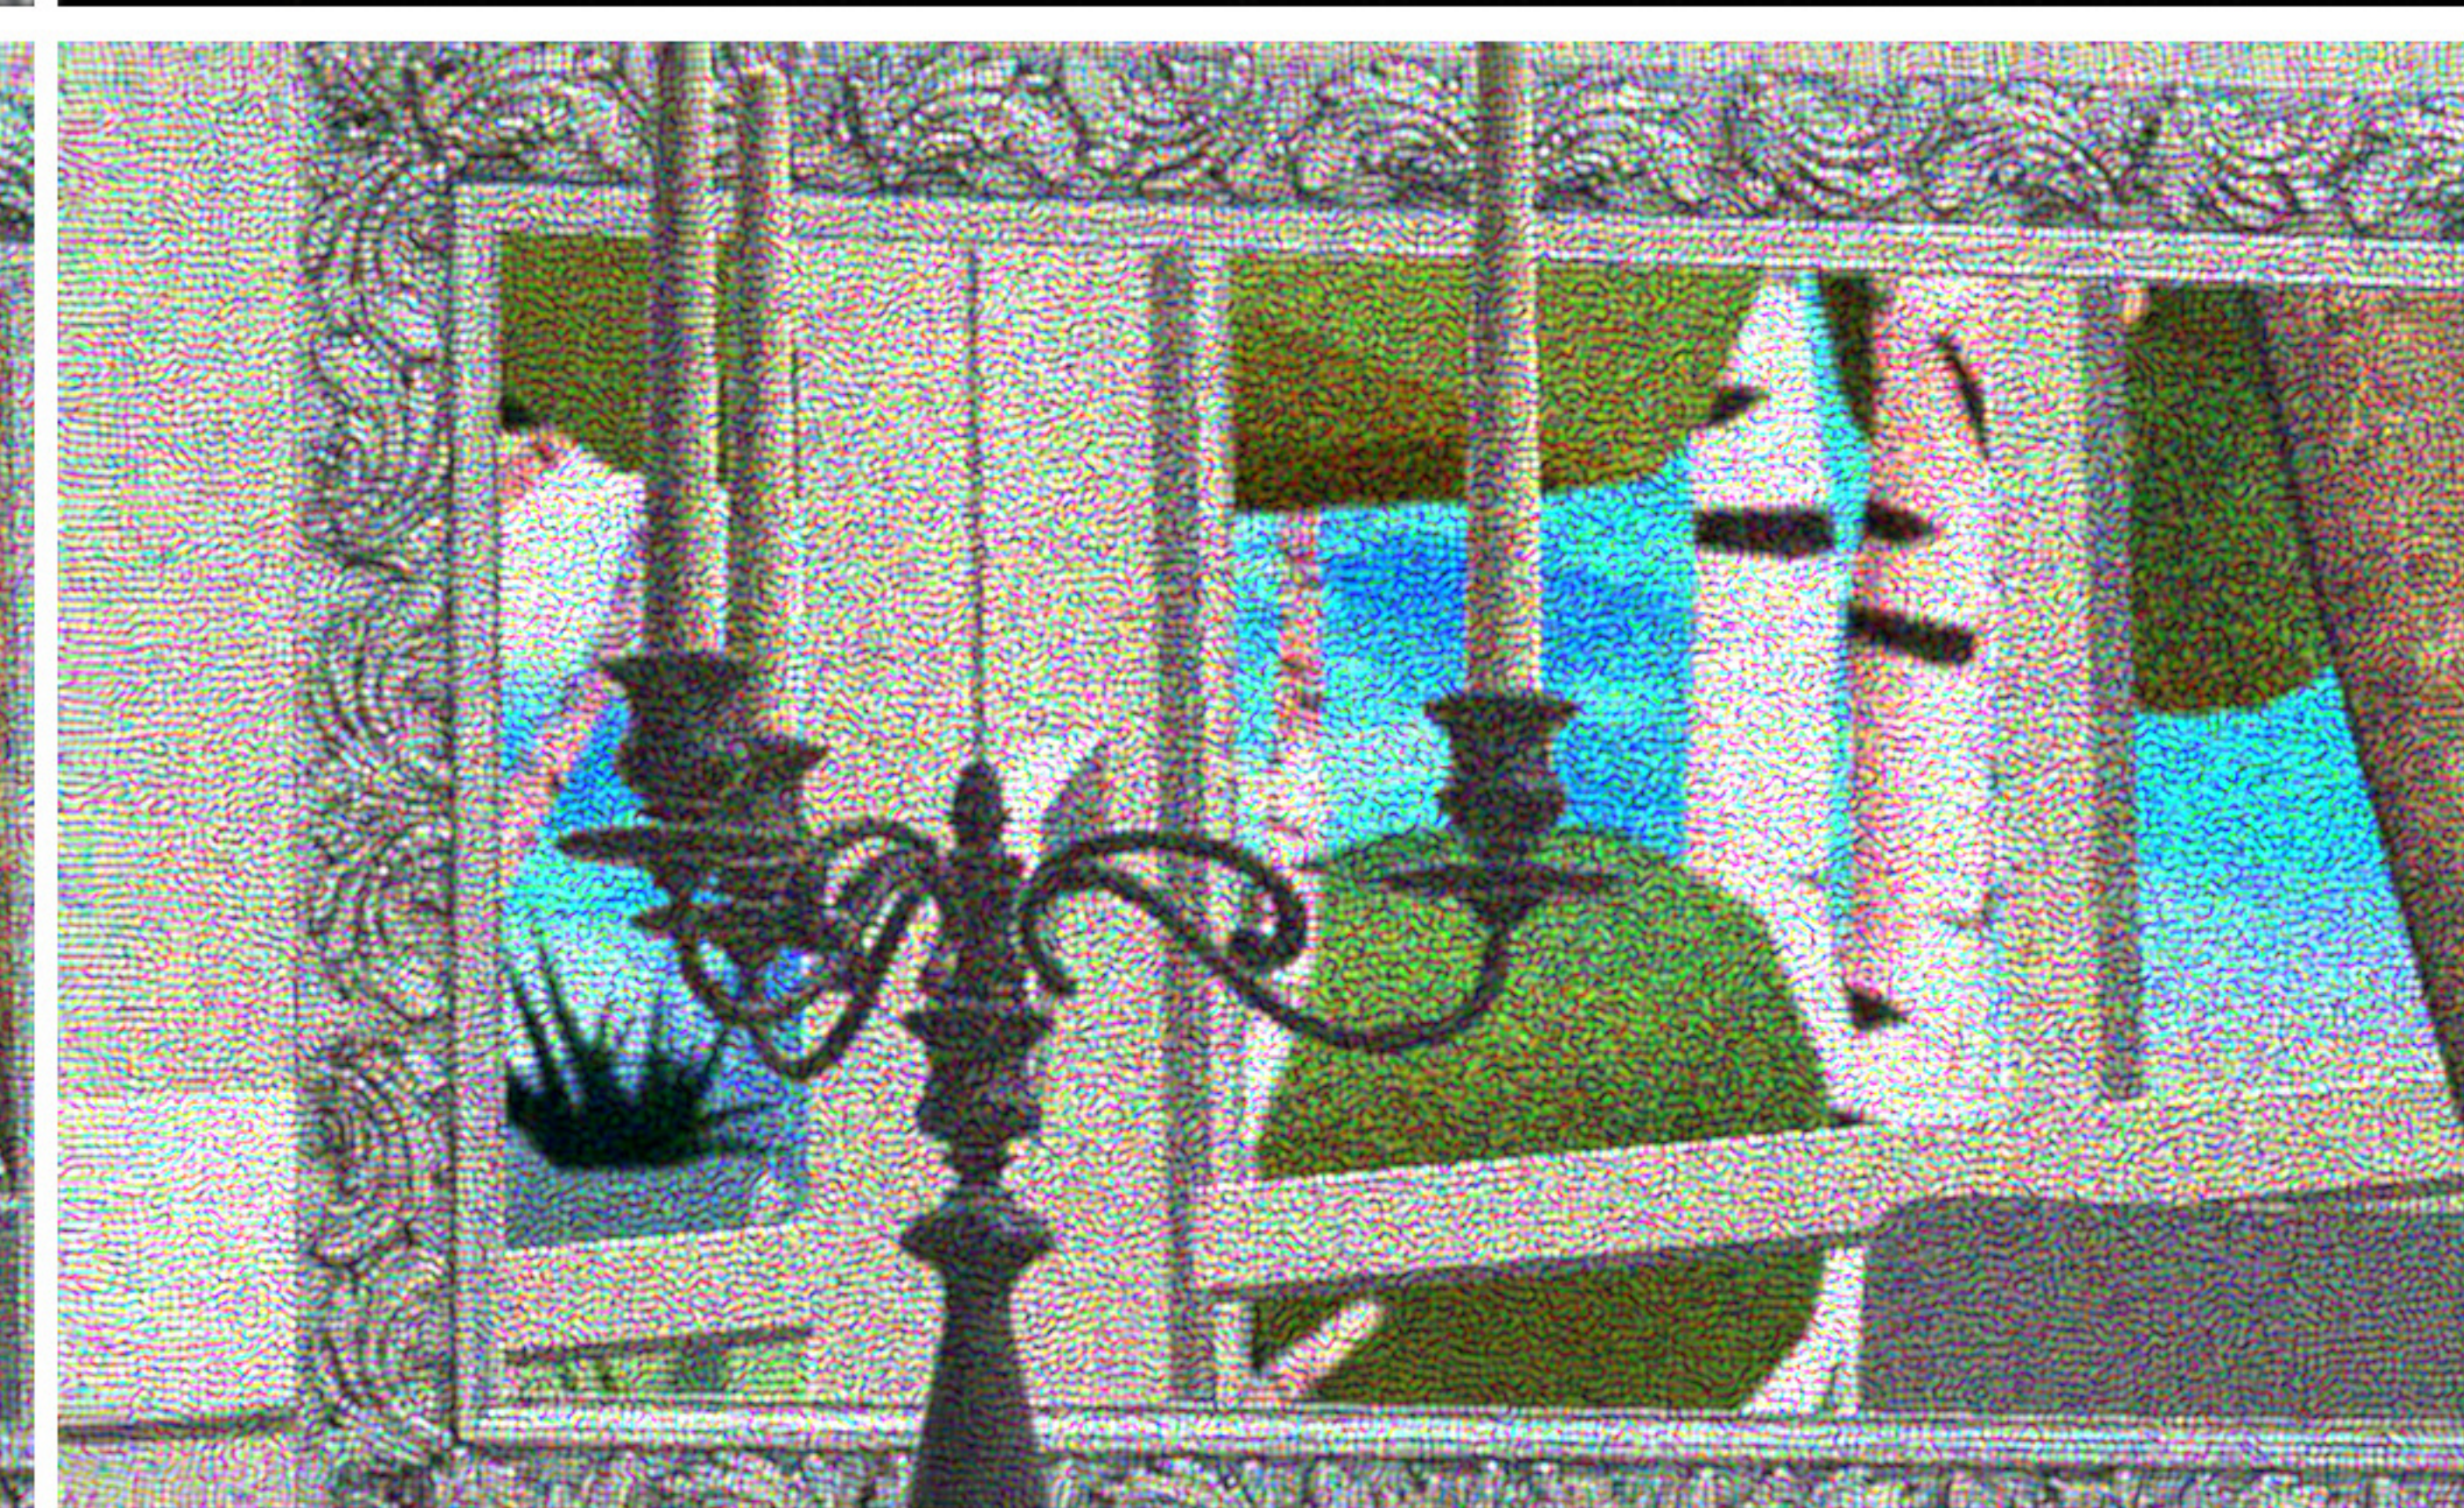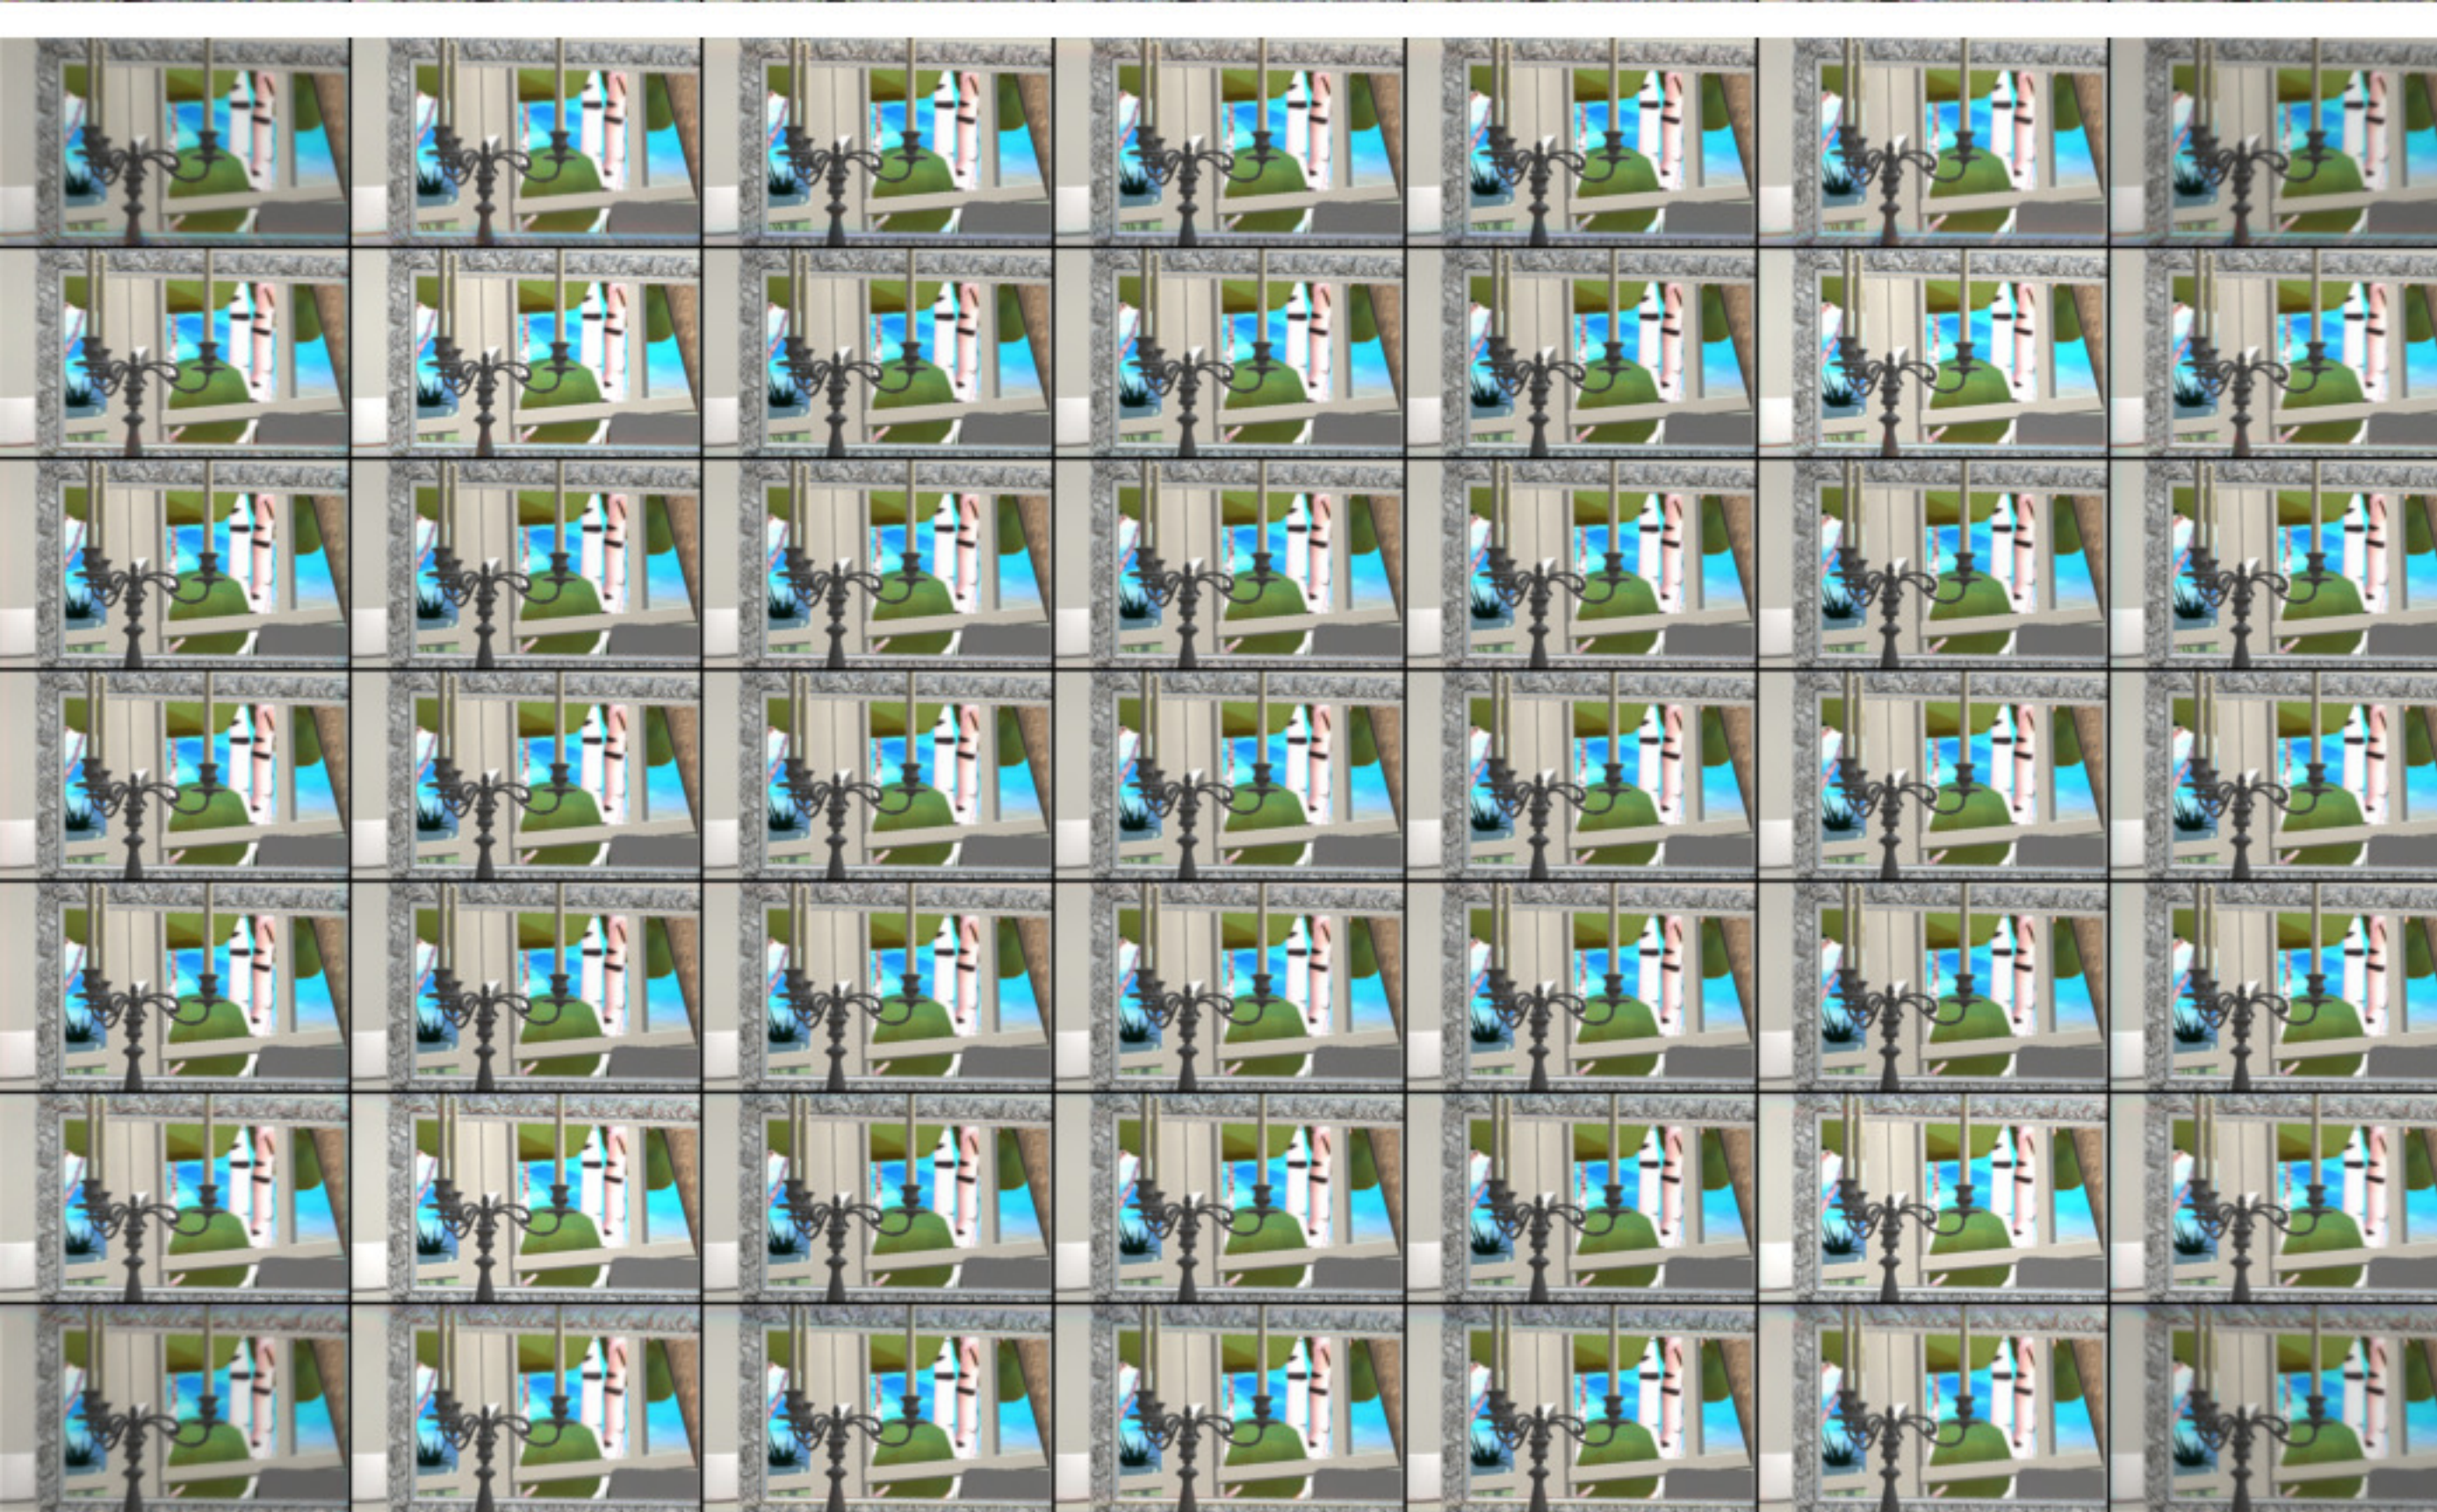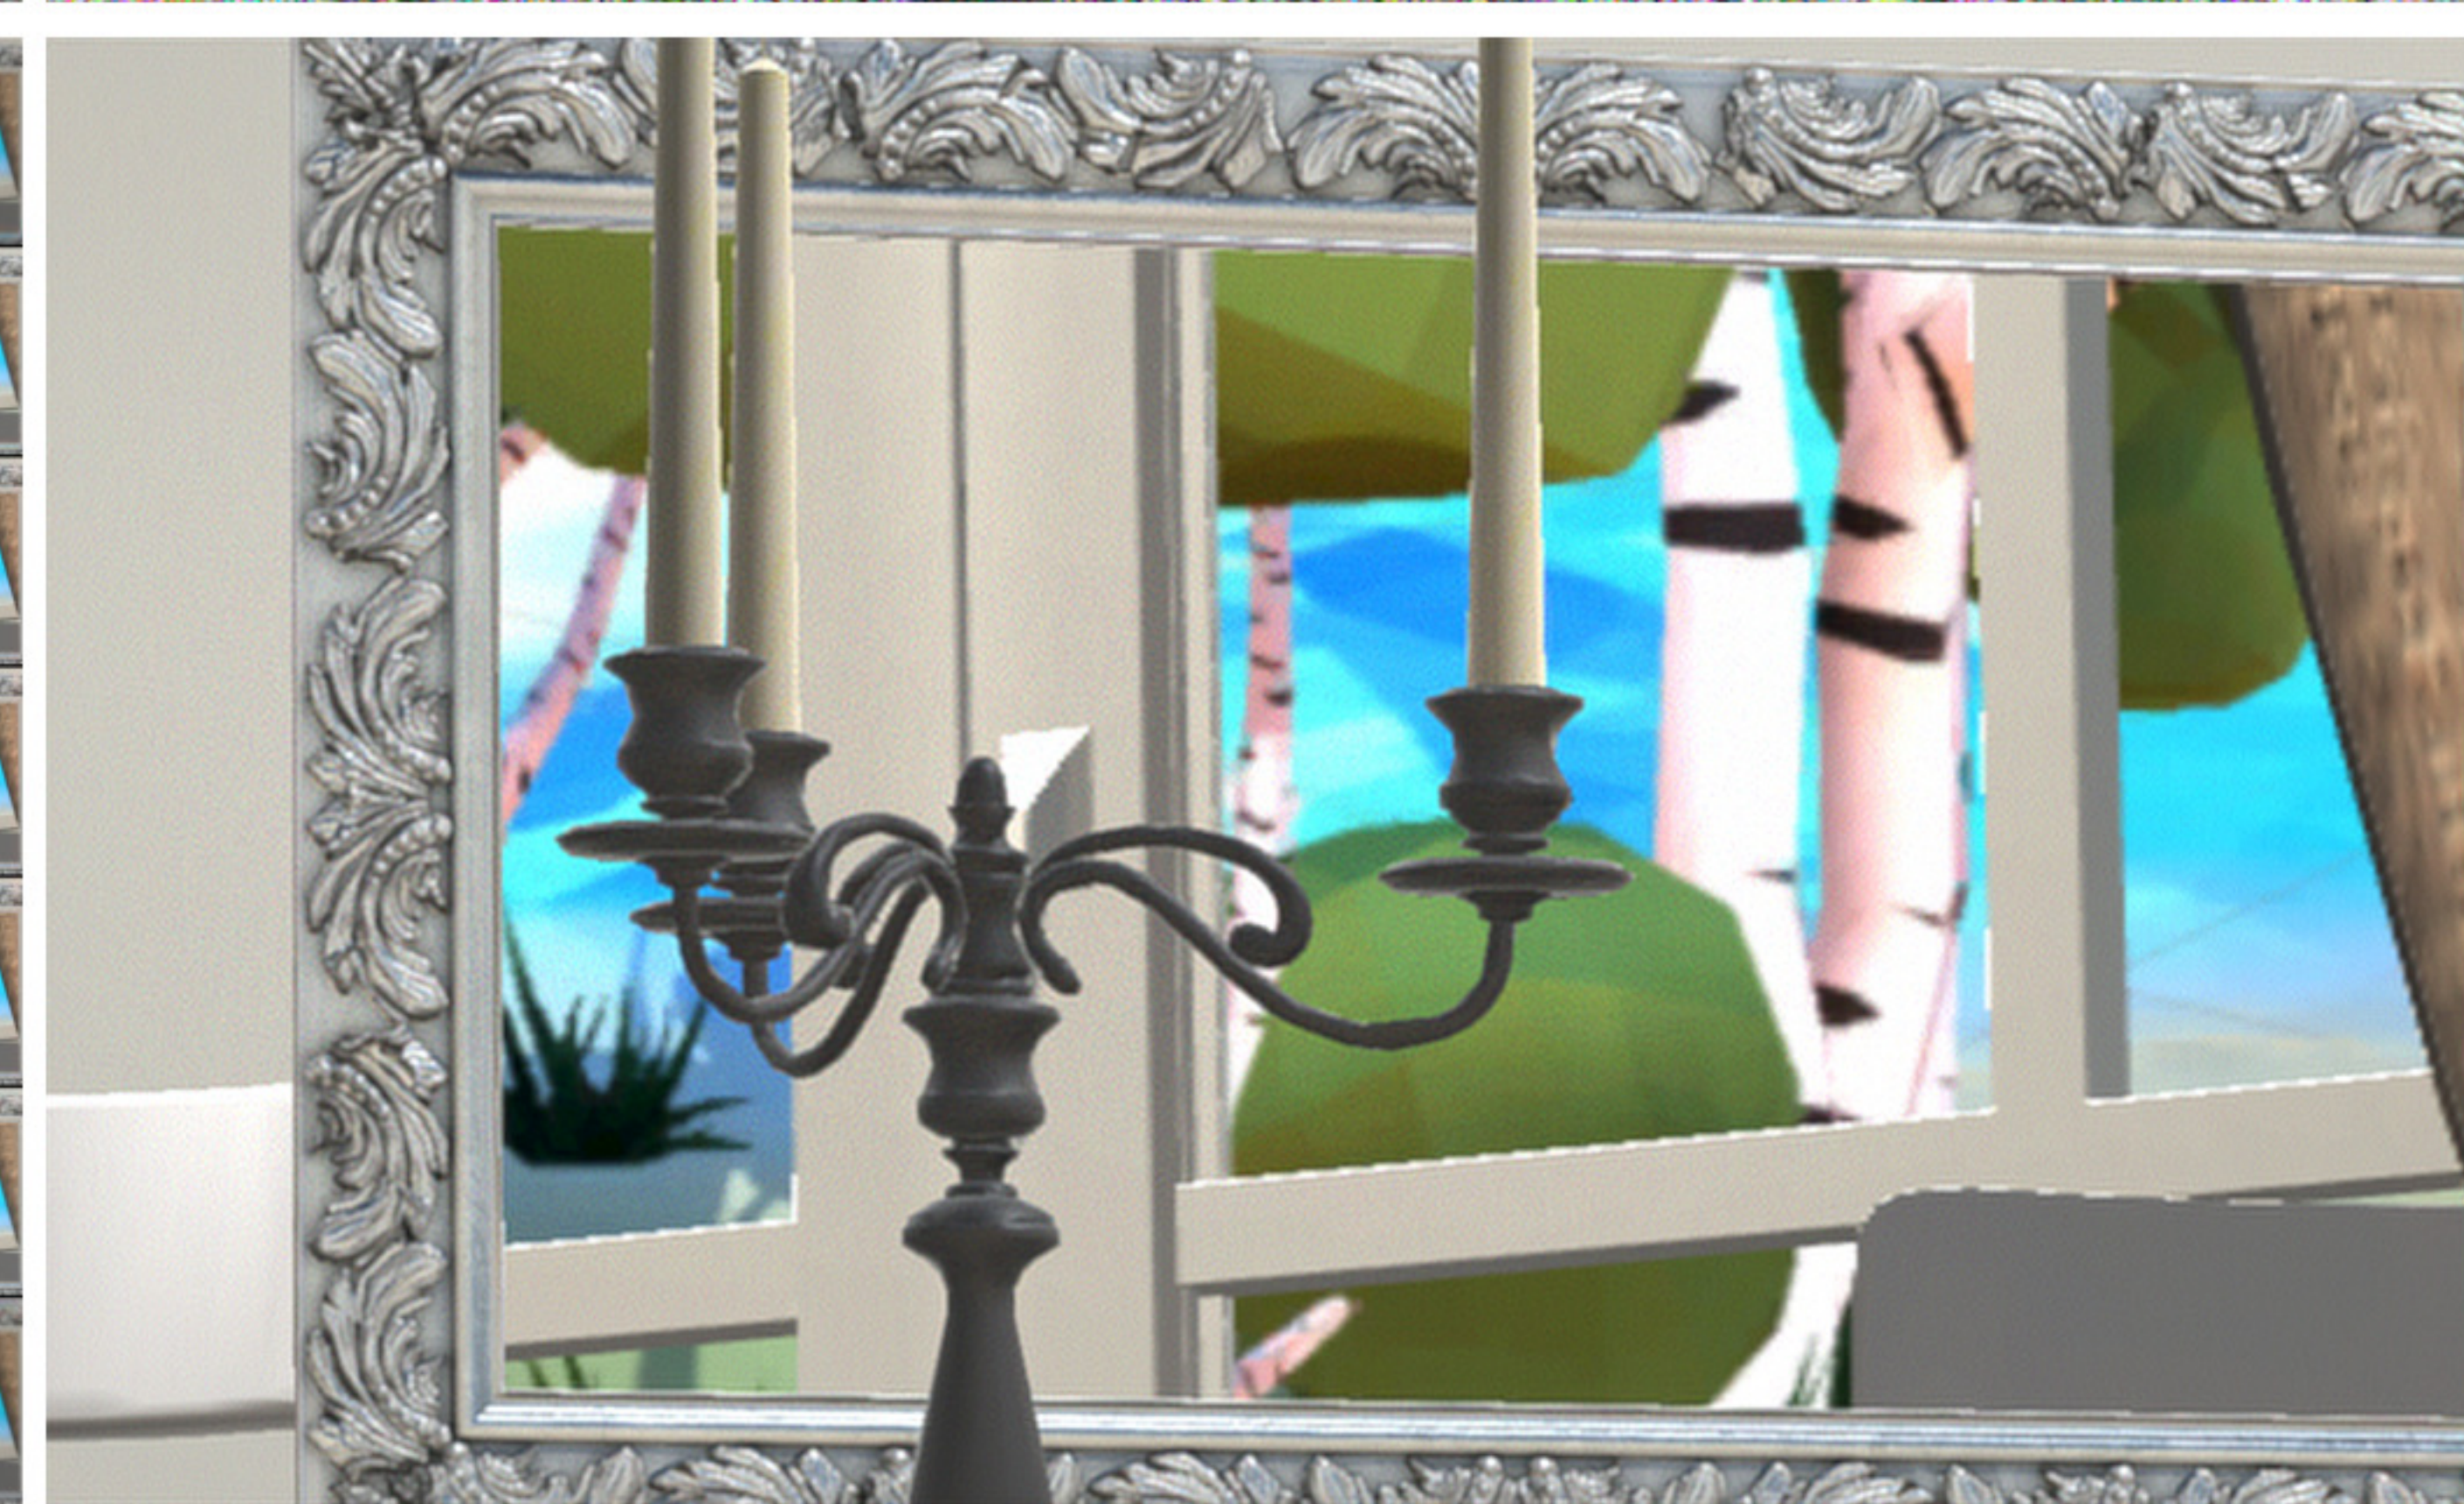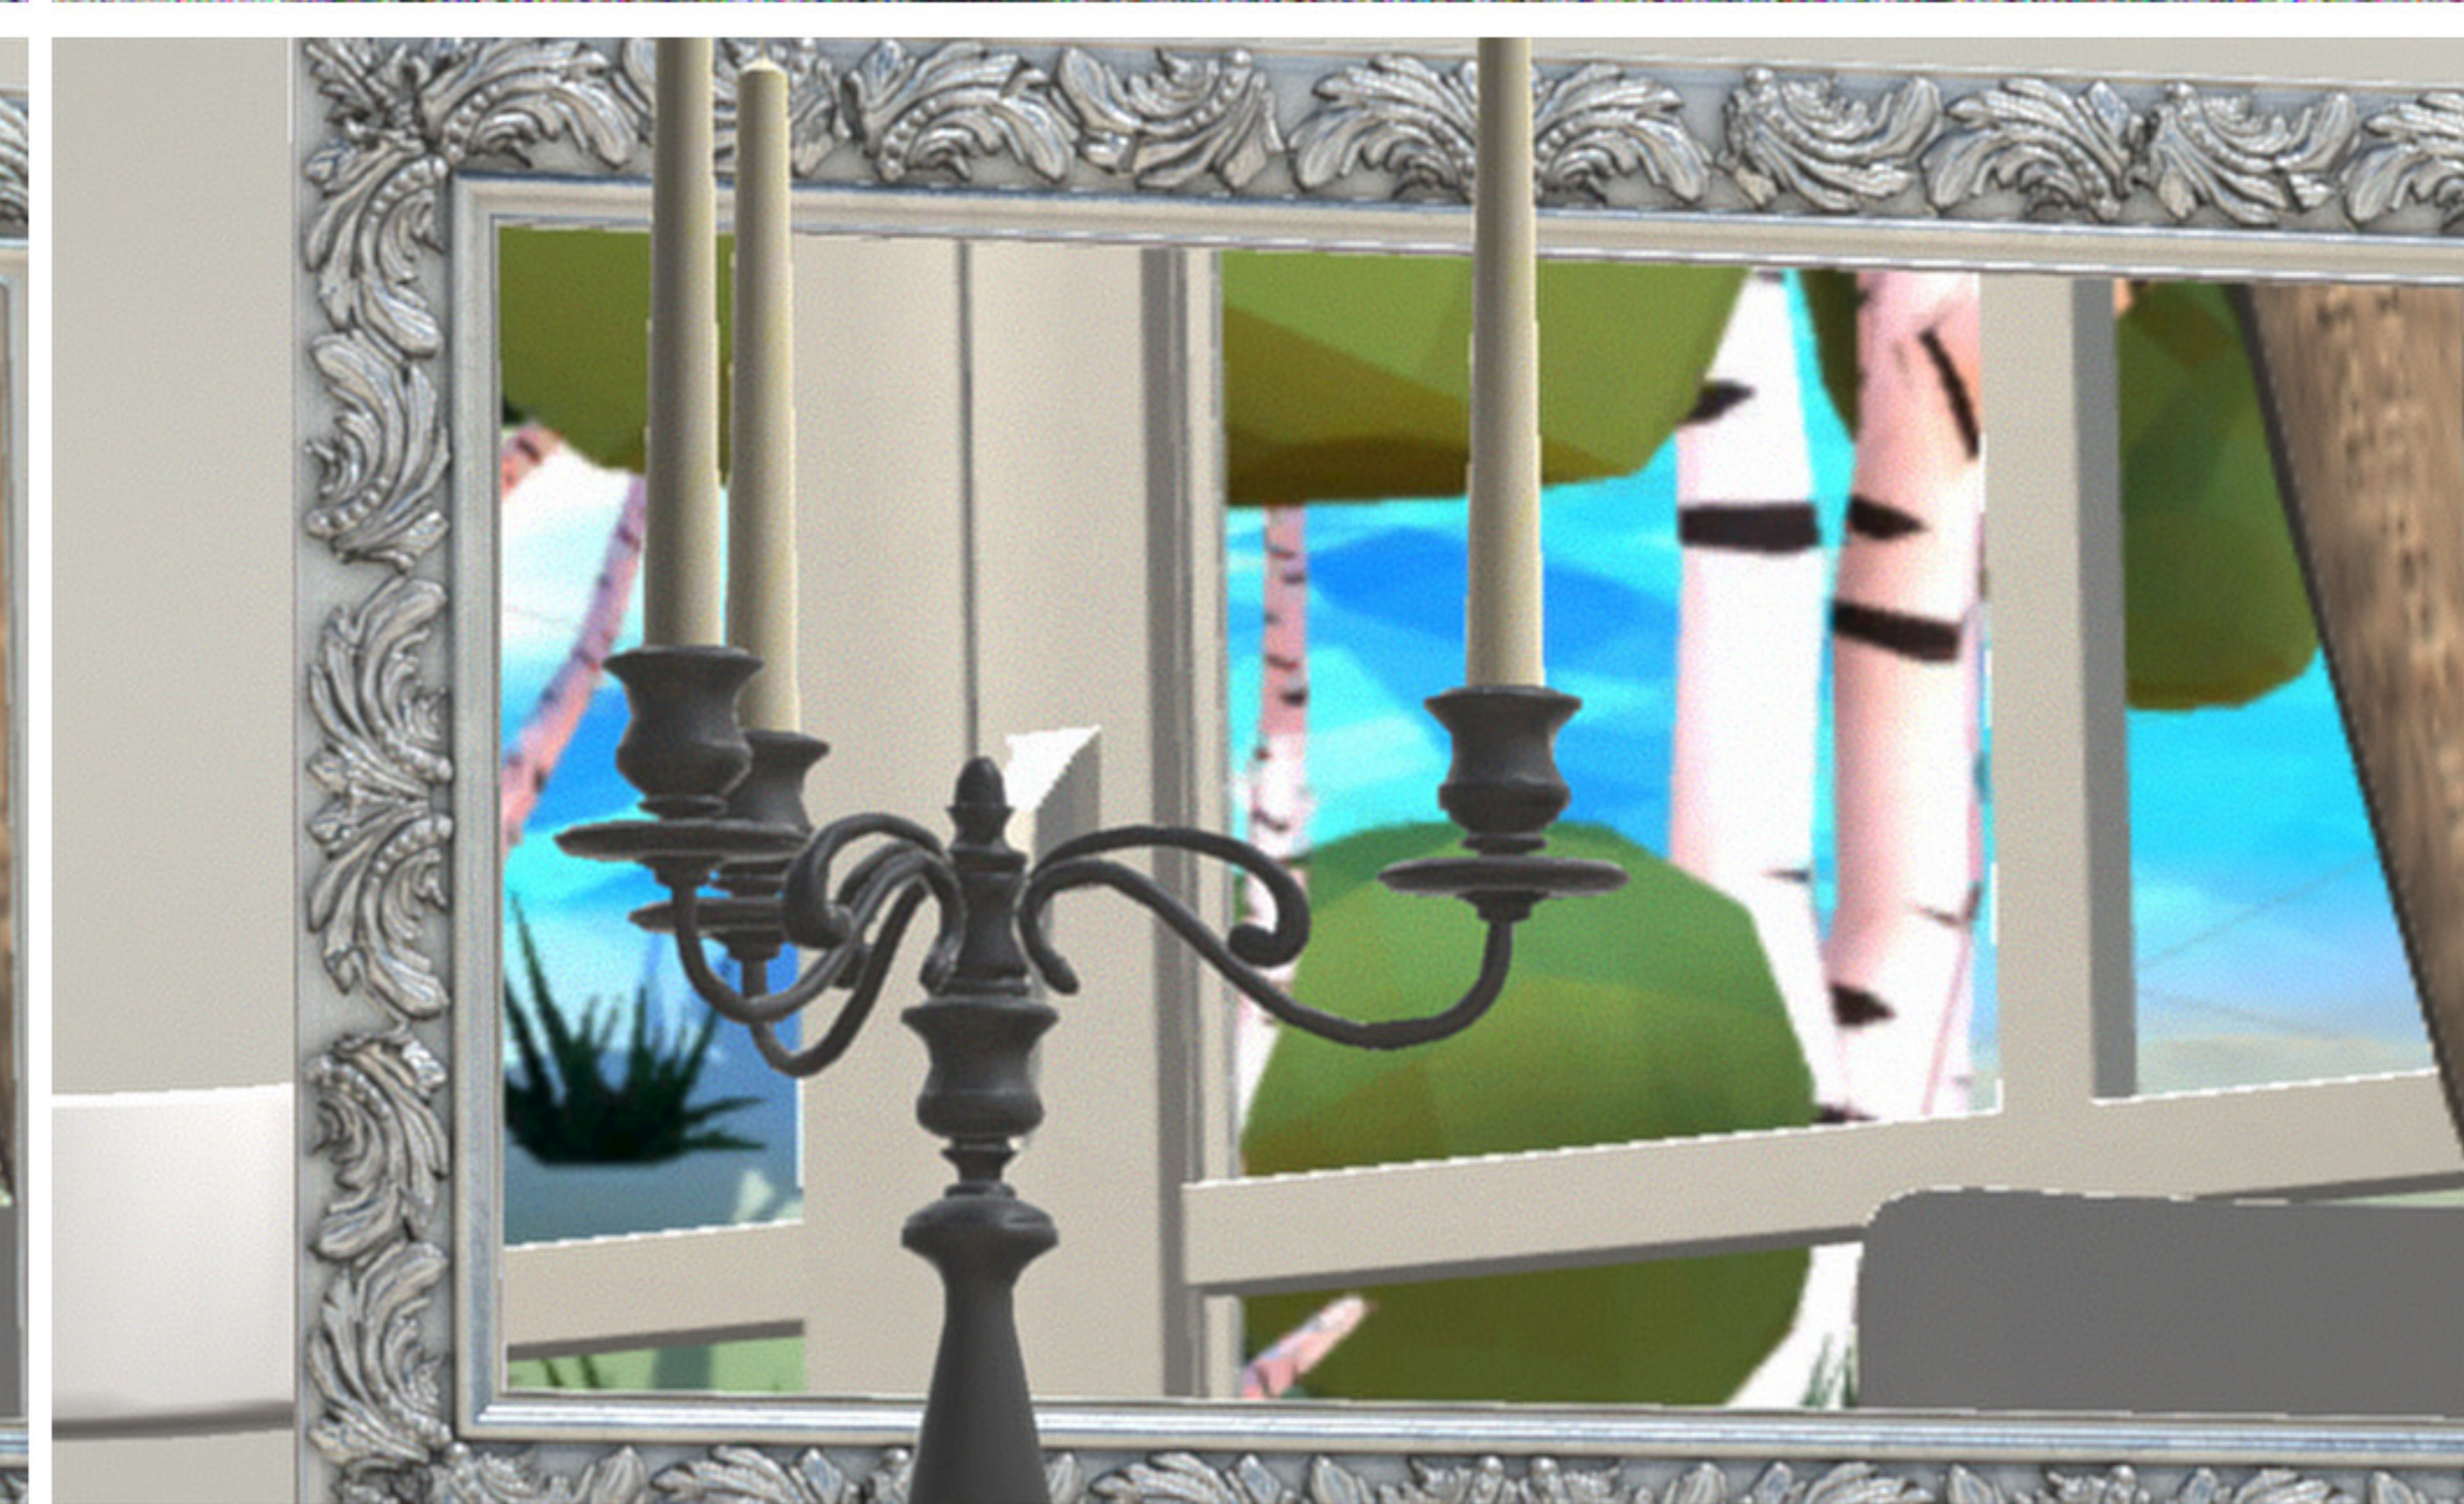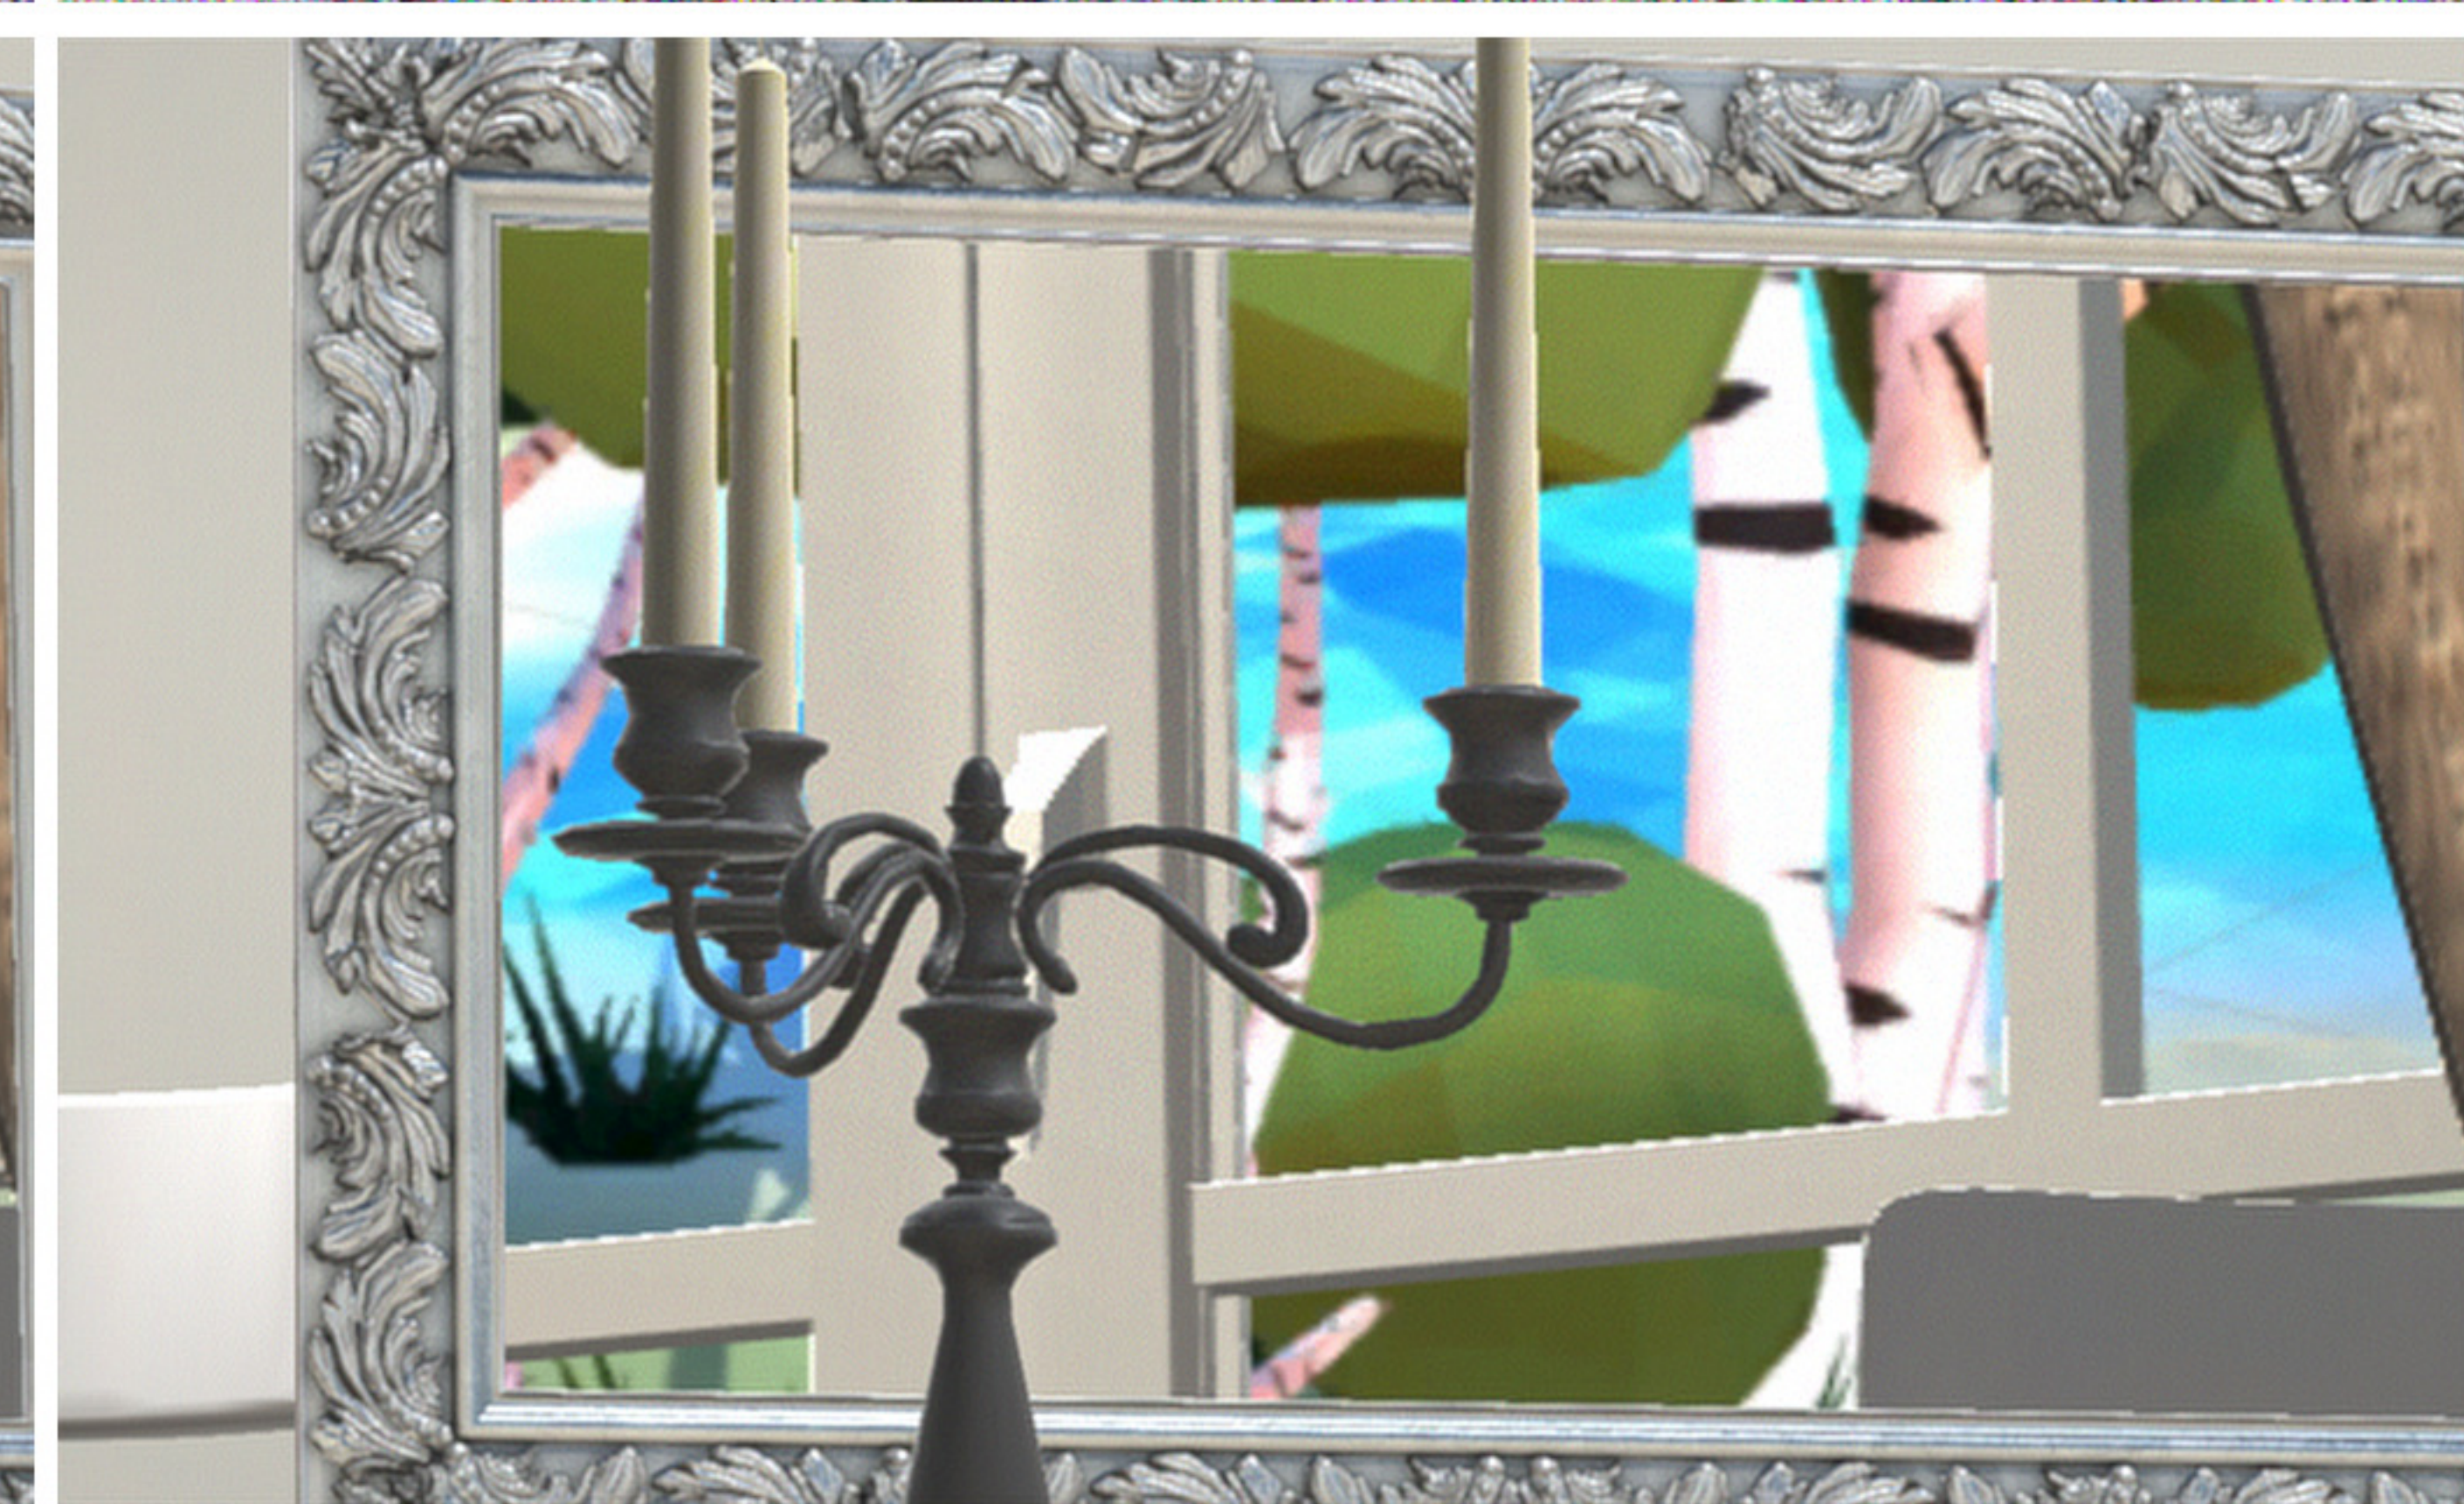

Supplement: Supplementary file 1 [file suppl_results_4d_ablation_1_lf_simulation_compressed.pdf]
